# Supplementary material for: High-throughput calculations of spin Hall conductivity in non-magnetic 2D materials
Source: arXiv:2501.02110 ancillary file (2025-01-03)
Supplement: Supplementary file 1 [file supp.pdf]

# Supplementary Material: High-throughput calculations of spin Hall conductivity in non-magnetic 2D materials

Jiaqi Zhou,[1,*] Samuel Poncé,[2,3,†] and Jean-Christophe Charlier[1,‡]

[1] *Institute of Condensed Matter and Nanosciences, Université catholique de Louvain, 1348 Louvain-la-Neuve, Belgium*

[2] *European Theoretical Spectroscopy Facility and Institute of Condensed Matter and Nanosciences, Université catholique de Louvain, 1348 Louvain-la-Neuve, Belgium*

[3] *WEL Research Institute, Avenue Pasteur 6, 1300 Wavre, Belgium*

(Dated: December 26, 2024)

### Supplementary Sec. 1. Test on the frozen window maximum

The test of the maximum of frozen window is given based on 100 materials which were arbitrarily chosen, including 60 semiconductors and 40 metals. The DFT bands and Wannier bands generated with different frozen window maxima are compared using the band distance, which is defined by Eq. (4) in the main text. As demonstrated by Supplementary Fig. 1(a), $E_F$ + 2 eV gives the optimal result especially for the high-energy bands. The band distance of all the 426 materials is presented in Supplementary Fig. 1(b). Most materials present a small band distance below 2 meV.

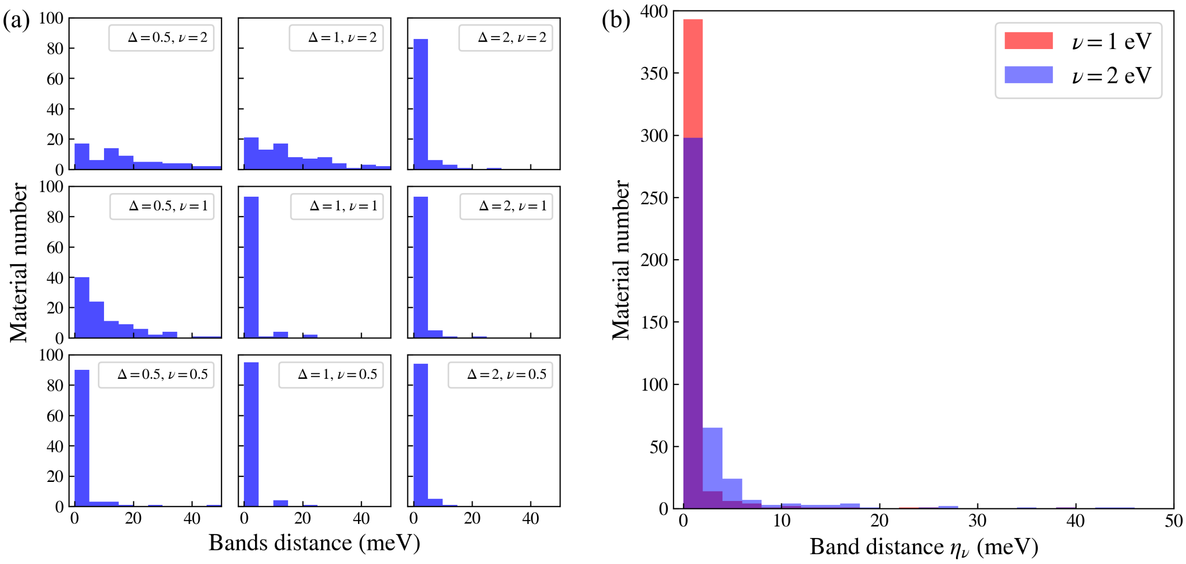


Supplementary Fig. 1. (a) Impact of the maximum of frozen window based on 100 randomly selected materials. In the Wannierization, the maximum of the frozen windows is given by $E_F + \Delta$ (unit: eV) where $\Delta = 0.5$, 1, and 2, respectively. The band distance below $E_F + \nu$ where $\nu = 0.5$, 1, and 2 are respectively evaluated. For insulators, $E_F$ is defined as the conduction band minimum. (b) Distribution of band distances for all the 426 monolayers using a frozen window of $\Delta = 2$ eV.

* jiaqi.zhou@uclouvain.be

† samuel.ponce@uclouvain.be

‡ jean-christophe.charlier@uclouvain.be

## Supplementary Sec. 2. Metals with high SHC

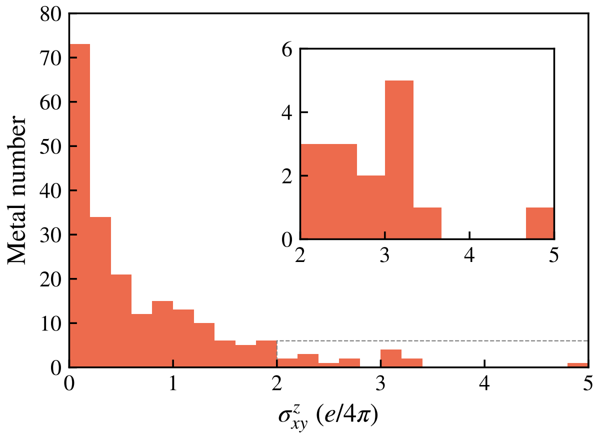


Supplementary Fig. 2. Spin Hall conductivities of 210 monolayer metals. The inset shows the region where 15 materials presents high spin Hall conductivities of $|\sigma_{xy}^{z}| > 2\ e/4\pi$. These 15 materials are reported in Supplementary Table 1.

Supplementary Table 1: 15 monolayer metals with $|\sigma_{xy}^{z}| > 2\ e/4\pi$.

| Monolayer | Space group | $\lvert\sigma_{xy}^{z}\rvert$ $(e/4\pi)$ |
|---|---|---|
| $BiTe_2$ | P-3m1 | 4.88 |
| $LiMnTe_2$ | P3m1 | 3.39 |
| $NaMnTe_2$ | P3m1 | 3.24 |
| $AgCuTe_2$ | Pmm2 | 3.14 |
| $Y_2Cl_2$ | P-3m1 | 3.14 |
| $LiMnSe_2$ | P3m1 | 3.11 |
| $Ta_4Se_2$ | P4/nmm | 3.08 |
| $Sn_2P$ | P-3m1 | 2.75 |
| $Co_2S_2$ | P4/nmm | 2.71 |
| $Sb_2Te_2$ | P-3m1 | 2.55 |
| $Ba_2Ni_3$ | P-3m1 | 2.39 |
| $Y_2Br_2$ | P-3m1 | 2.38 |
| $In_2Te_3$ | P-3m1 | 2.31 |
| $CoBr_2$ | P-3m1 | 2.01 |
| $Tl_2I_2S_2$ | P4/nmm | 2.00 |

## Supplementary Sec. 3. Electronic structures and phonon dispersions of promising materials

Electronic structures and phonon dispersions of 8 materials with superior SHC properties are detailed here. For all the materials, the reproduction of DFT results illustrates the high-quality Wannierization. The absence of imaginary frequency suggests mechanical stability. The $Sn_2P$ and $Y_2Br_2$ monolayers are discussed in more depths since they required special treatments.

The $Sn_2P$ monolayer with the P-3m1 space group presents negative frequencies around Γ as shown in Supplementary Fig. 3, which is consistent with Ref. [1]. To eliminate the negative frequencies, the structure of $Sn_2P$ monolayer was relaxed without any symmetry. To obtain initial structures for relaxation, 10 structures randomly displaced for the equilibrium position were generated with the P1 space group. Then their total energies were calculated, 3 of them present the same total energy minima, and only 1 structure presents a positive phonon dispersion. This relaxed structure is given in Supplementary Table 2. Electronic structure and phonon dispersion of this low-symmetry structure are depicted in Supplementary Fig. 4. The comparison between Supplementary Fig. 3(a) and Supplementary Fig. 4(a) illustrates that the change of electronic structure is negligible. However, the broken symmetry is critical to obtain a positive phonon dispersion as shown in Supplementary Fig. 4(b). This low-symmetry $Sn_2P$ monolayer is the material reported in the main text.

We now focus on $Y_2Br_2$. The possible magnetism of $Y_2Br_2$ has been considered since $Y_2Cl_2$ was predicted to be a ferromagnet [2]. Due to the self-interaction error in exchange-correlation functional, a Hubbard correction was included with magnetism. The *ab initio* Hubbard parameter U = 1.16 eV computing using density-functional perturbation theory and atomic projectors [3]. As shown in Supplementary Fig. 5 and Supplementary Fig. 6, both non-magnetic and ferromagnetic phases present positive phonon dispersions. However, apart from the mechanical stability, the thermal stability of magnetism should also be checked. The magnetic anisotropy is critical for the ferromagnetism in 2D material since it could stabilize the long-range magnetic order by opening up an excitation gap to resist the thermal agitation [4]. Defined as the energy difference between in-plane and out-of-plane magnetic configurations considering spin-orbital coupling, the magnetic anisotropic energy (MAE) of ferromagnetic $Y_2Br_2$ was calculated to be 0.03 meV. Two well-known 2D magnets can be taken as reference: $CrI_3$ monolayer with an MAE of 0.65 meV and a Curie temperature of 45 K [5], and $MnBi_2Te_4$ monolayer with an MAE of 0.15 meV with a Curie temperature of 20 K [6, 7]. With a much smaller MAE, the ferromagnetism of $Y_2Br_2$ is easily vulnerable to the thermal agitation, illustrating the difficulty of maintaining ferromagnetism at room temperature. As a result, $Y_2Br_2$ is expected to be non-magnetic at room temperature, and the non-magnetic configuration has been employed in the main text discussion.

Finally, Supplementary Fig. 7-Supplementary Fig. 12 show the electronic structures with SOC including DFT and Wannier bands and phonon dispersion without SOC.

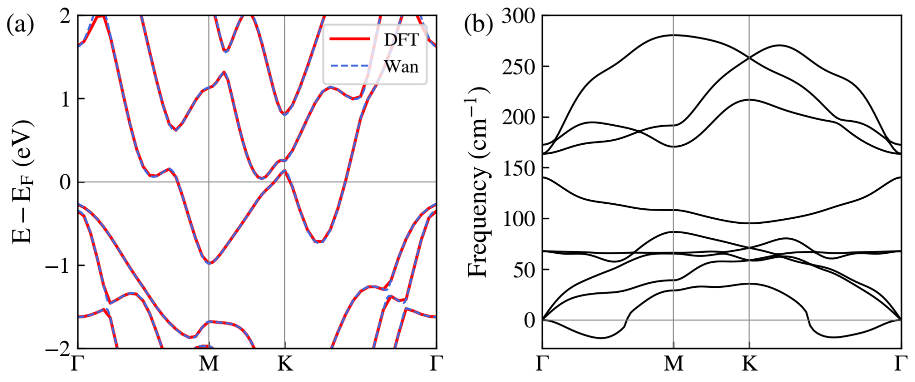


Supplementary Fig. 3. Electronic structure and phonon dispersion of the high-symmetry $Sn_2P$ monolayer.

Supplementary Table 2. Lattice vectors and atomic positions of the stable low-symmetry $Sn_2P$ monolayer.

| Lattice vectors | $x$ (Å) | $y$ (Å) | $z$ (Å) |
|---|---|---|---|
| $\mathbf{a}_1$ | 3.6891078804627813 | –0.0000036894473096 | 0.0000000000000000 |
| $\mathbf{a}_2$ | –1.8445281141002232 | 3.1948732083140299 | 0.0000000000000000 |
| $\mathbf{a}_3$ | 0.0000000000000000 | 0.0000000000000000 | 23.1653976932423795 |
| **Atomic positions** | **$x$ (Å)** | **$y$ (Å)** | **$z$ (Å)** |
| Sn | 0.1155841121498199 | 2.0834497119210194 | 2.1794277321228130 |
| P | 1.9600579913745917 | 1.0184036750440661 | 0.4381801612843048 |
| Sn | 0.1154896622986938 | –0.0464530931859039 | –1.3030736816146300 |

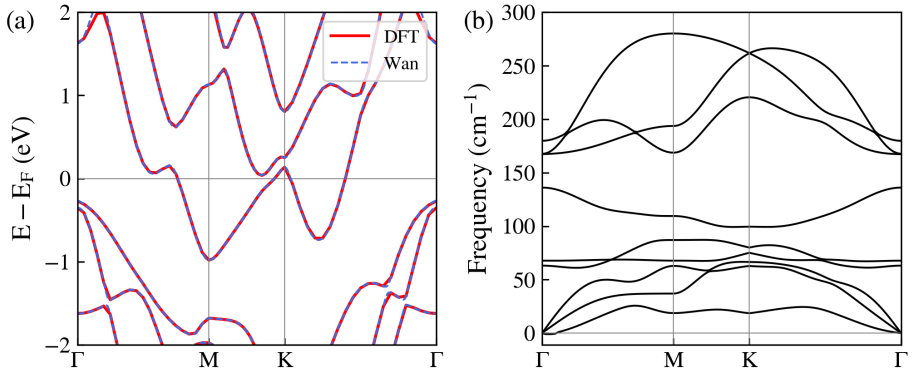


Supplementary Fig. 4. Electronic structure and phonon dispersion of the low-symmetry $Sn_2P$ monolayer.

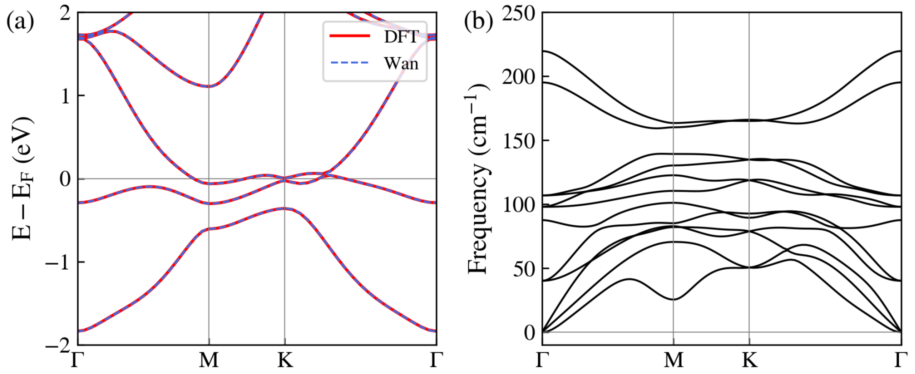


Supplementary Fig. 5. Electronic structure and phonon dispersion of the non-magnetic $Y_2Br_2$ monolayer.

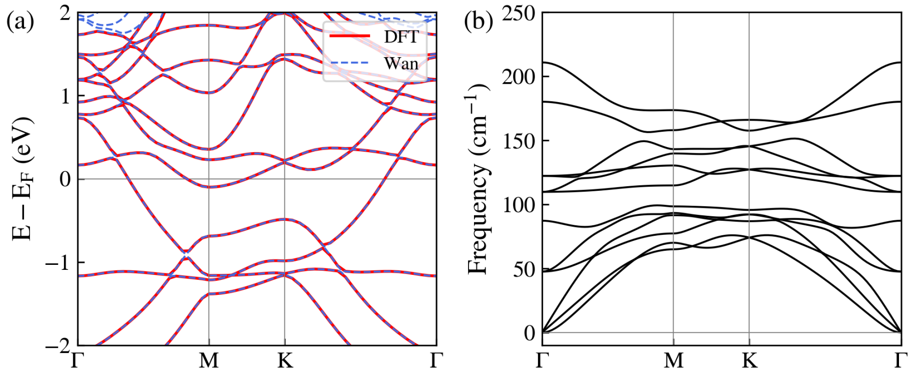


Supplementary Fig. 6. Electronic structure and phonon dispersion of the ferromagnetic $Y_2Br_2$ monolayer.

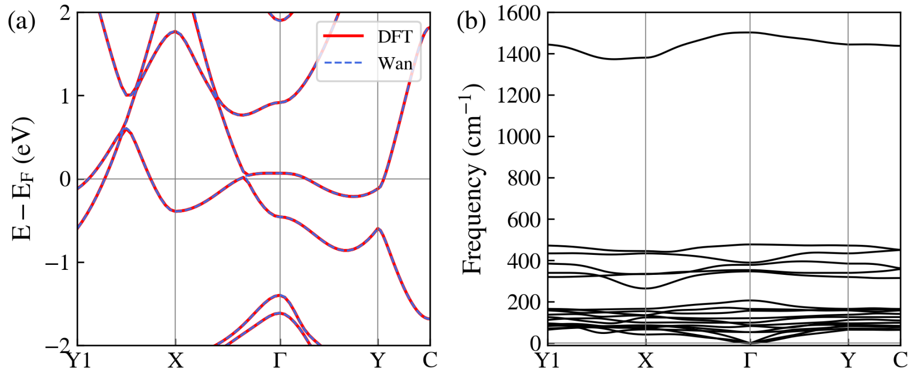


Supplementary Fig. 7. Electronic structure and phonon dispersion of the $Y_2C_2I_2$ monolayer.

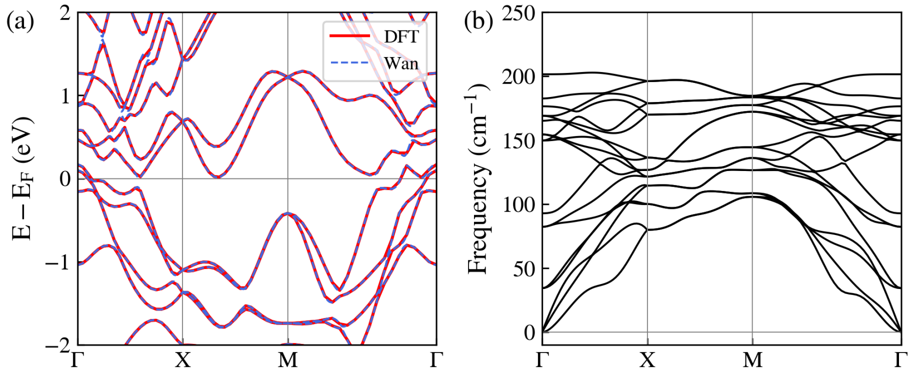


Supplementary Fig. 8. Electronic structure and phonon dispersion of the $Ta_4Se_2$ monolayer.

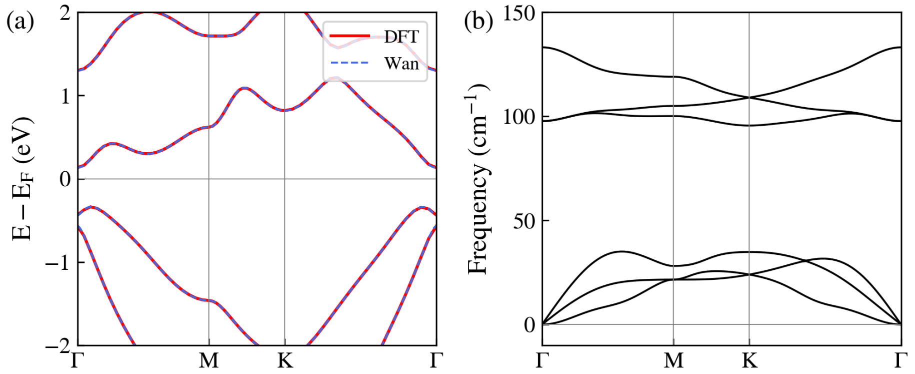


Supplementary Fig. 9. Electronic structure and phonon dispersion of the $Bi_2$ monolayer.

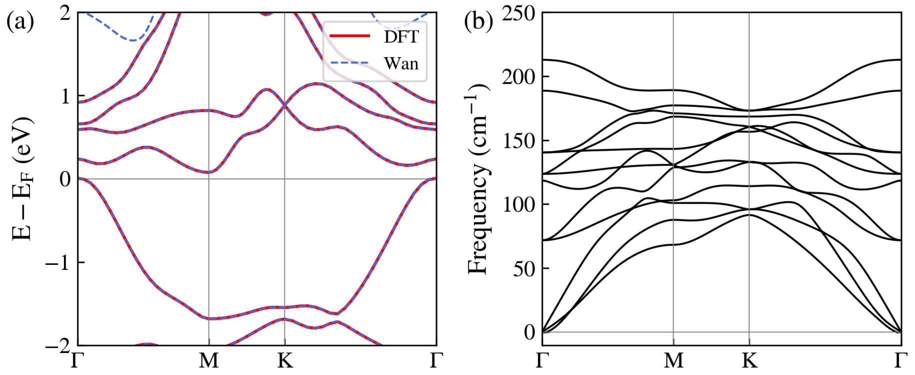


Supplementary Fig. 10. Electronic structure and phonon dispersion of the $Hf_2Br_2$ monolayer.

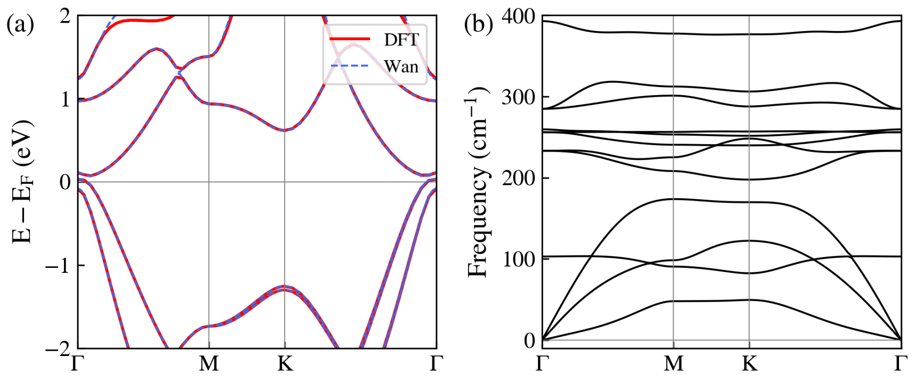


Supplementary Fig. 11. Electronic structure and phonon dispersion of the $CuLi_2As$ monolayer.

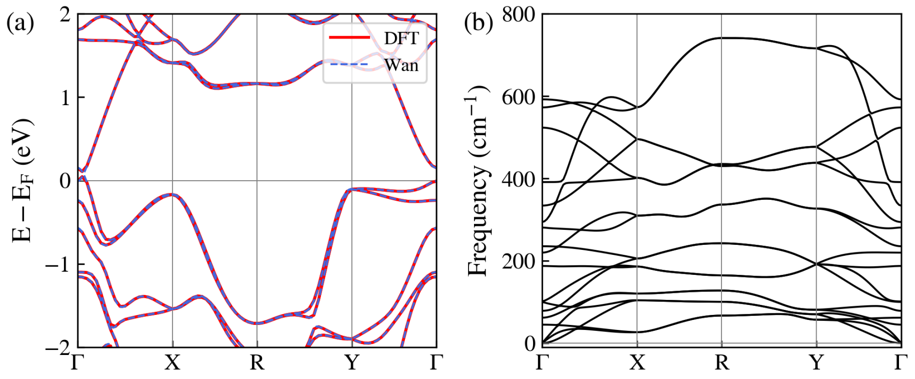


Supplementary Fig. 12. Electronic structure and phonon dispersion of the $Ti_2N_2I_2$ monolayer.

## Supplementary Sec. 4. Fully relativistic electronic structures of 210 monolayer metals

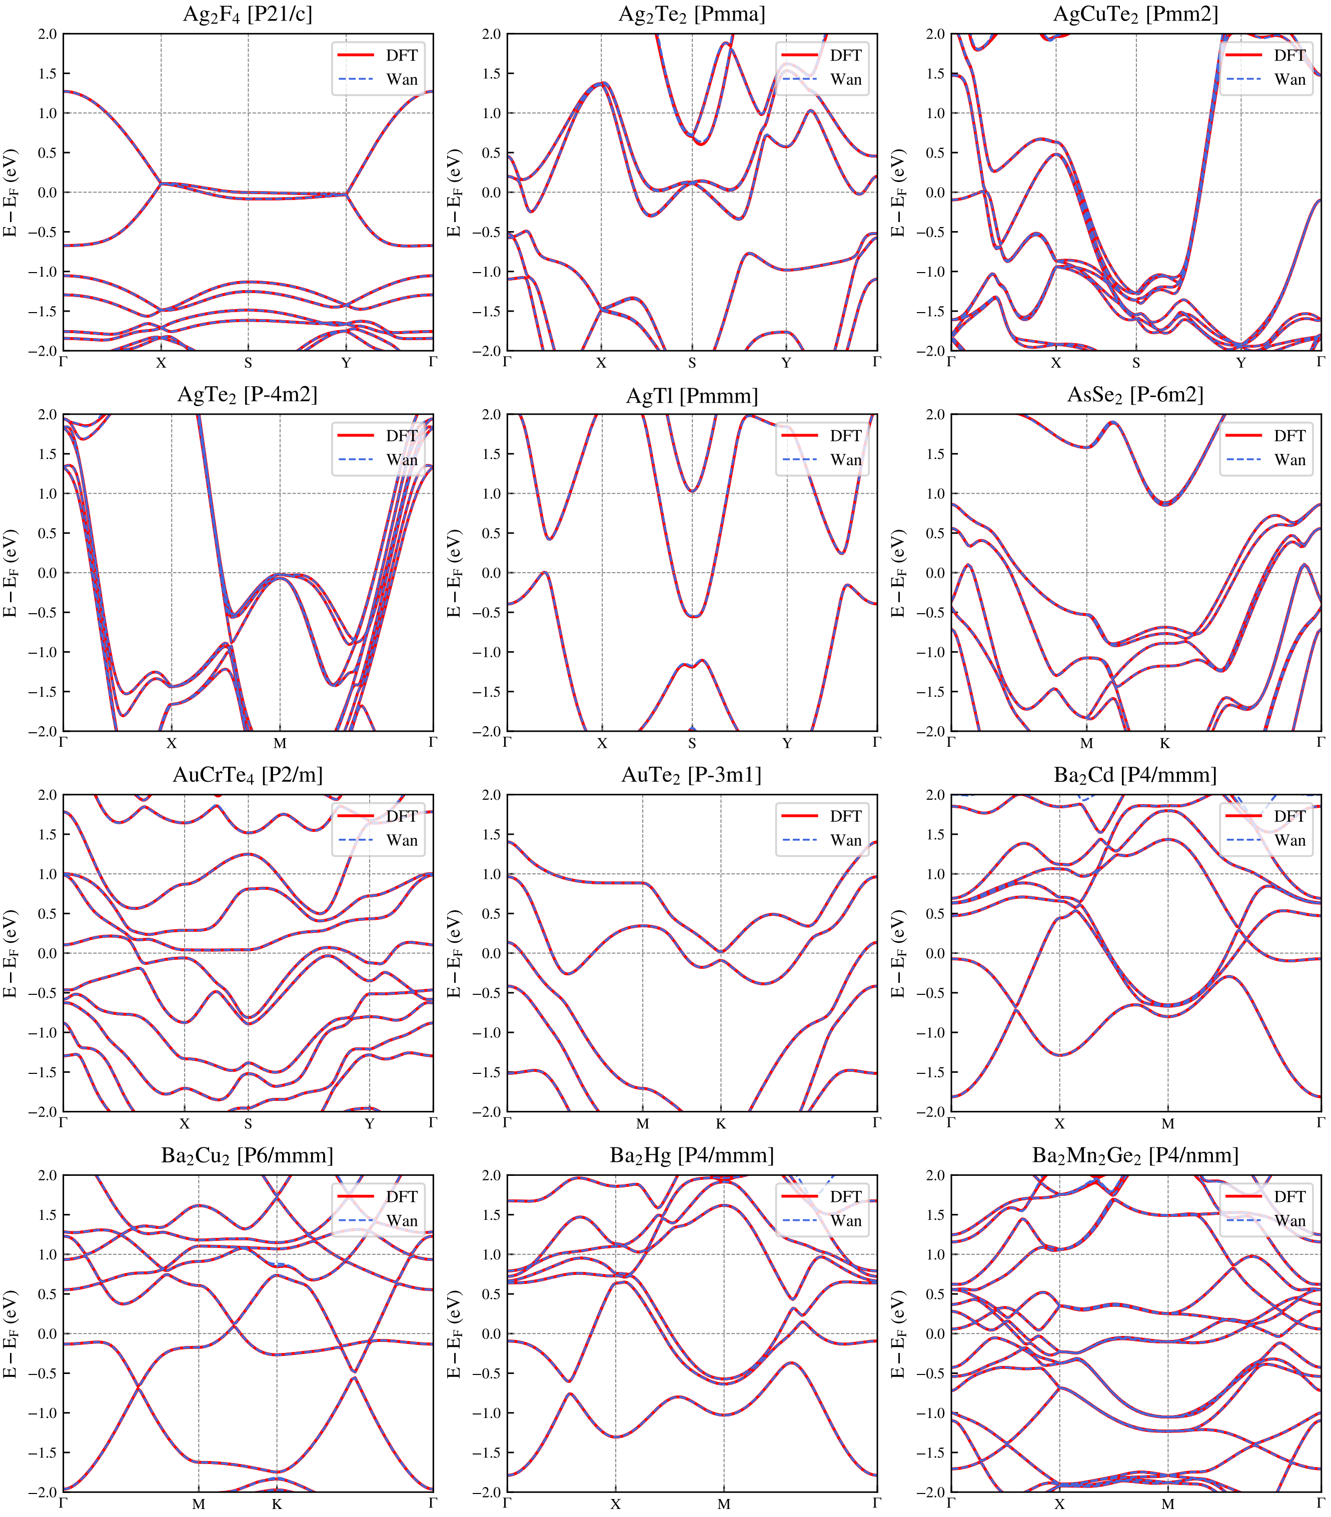

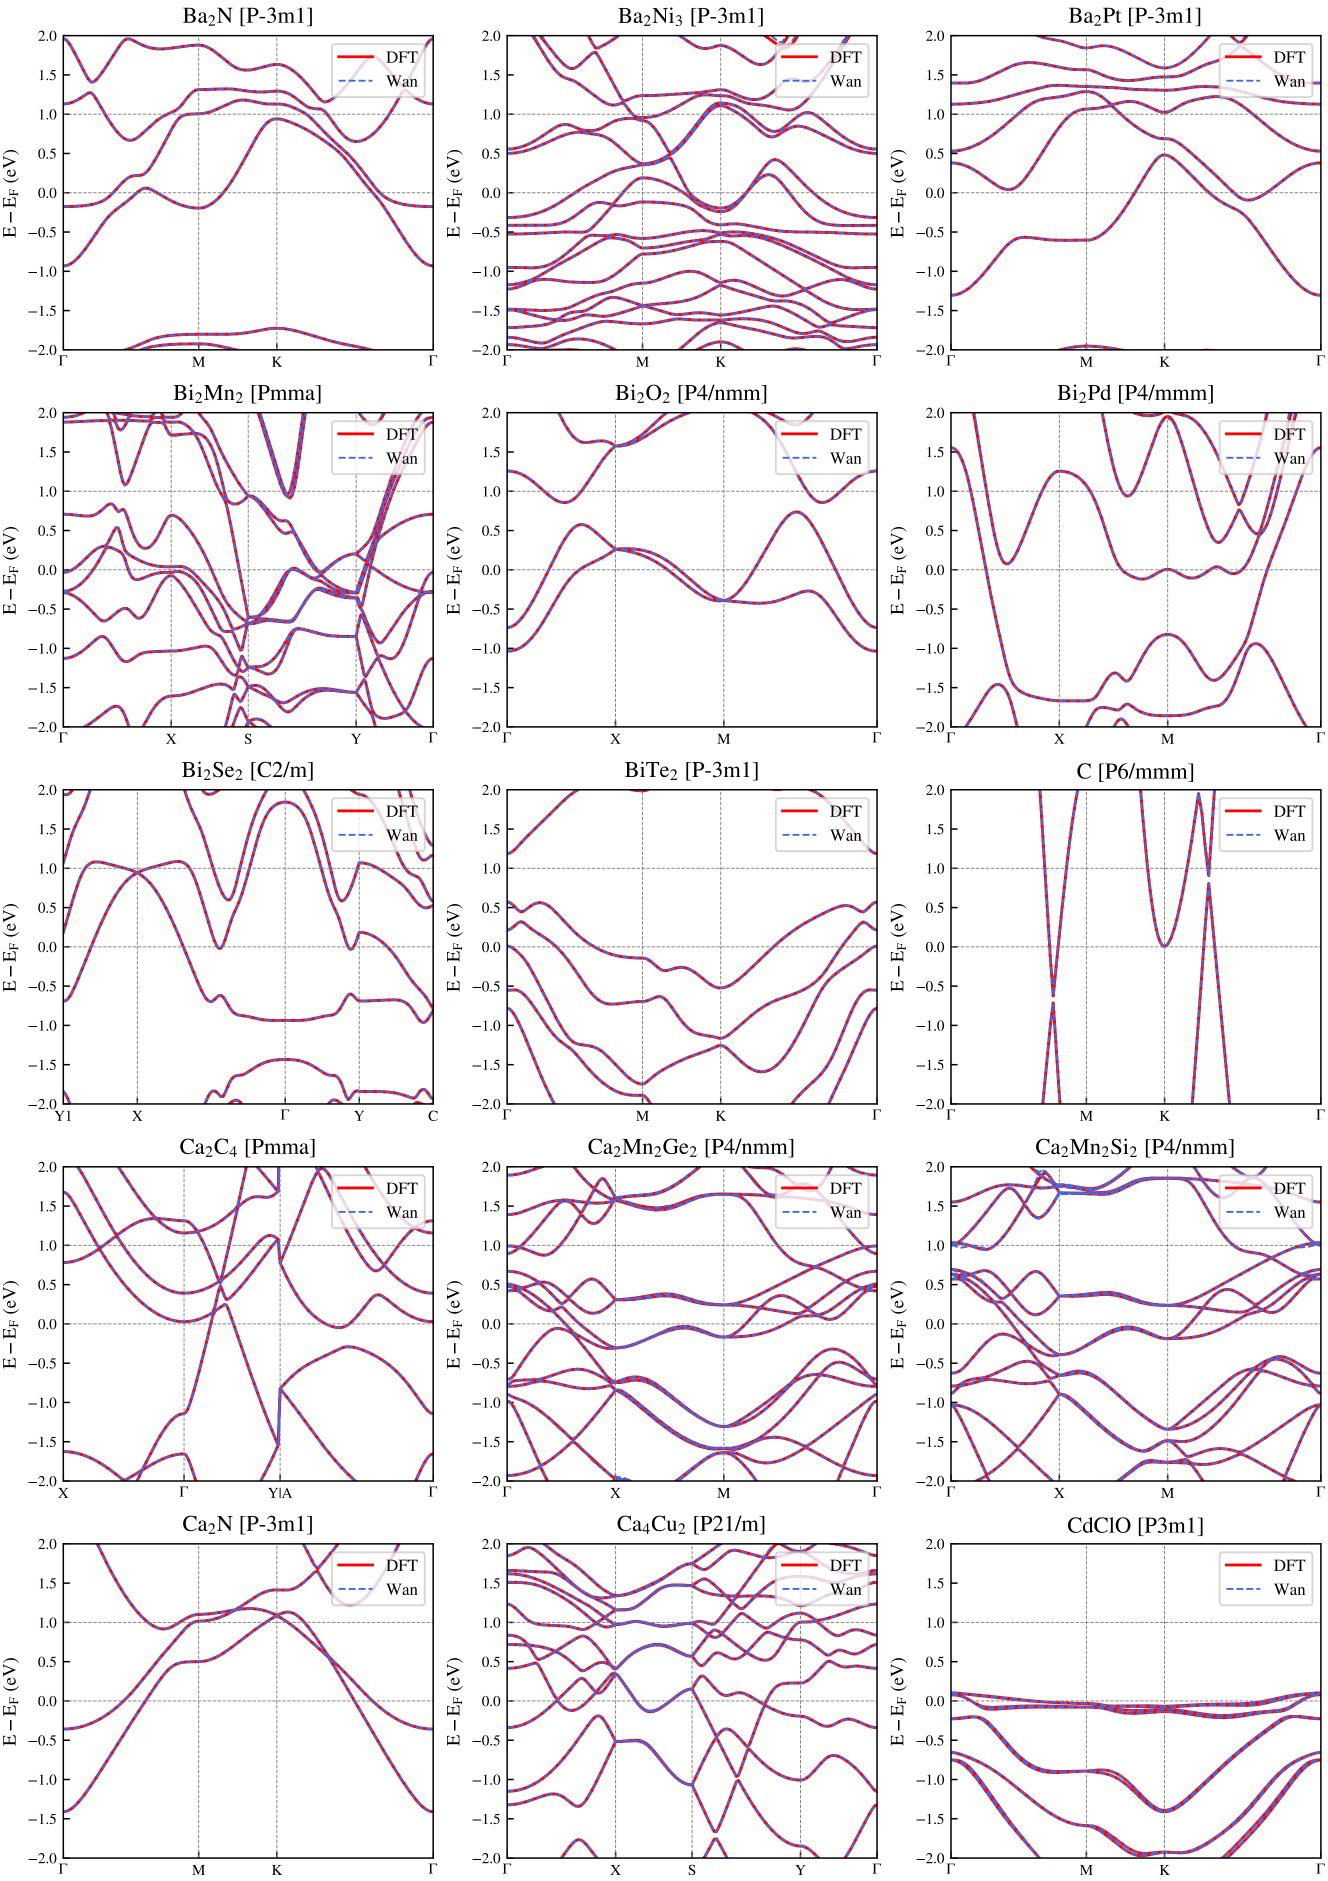
Ba2N [P-3m1]
Ba2Ni3 [P-3m1]
Ba2Pt [P-3m1]
Bi2Mn2 [Pmma]
Bi2O2 [P4/nmm]
Bi2Pd [P4/mmm]
Bi2Se2 [C2/m]
BiTe2 [P-3m1]
C [P6/mmm]
Ca2C4 [Pmma]
Ca2Mn2Ge2 [P4/nmm]
Ca2Mn2Si2 [P4/nmm]
Ca2N [P-3m1]
Ca4Cu2 [P21/m]
CdClO [P3m1]
DFT
Wan
E − EF (eV)

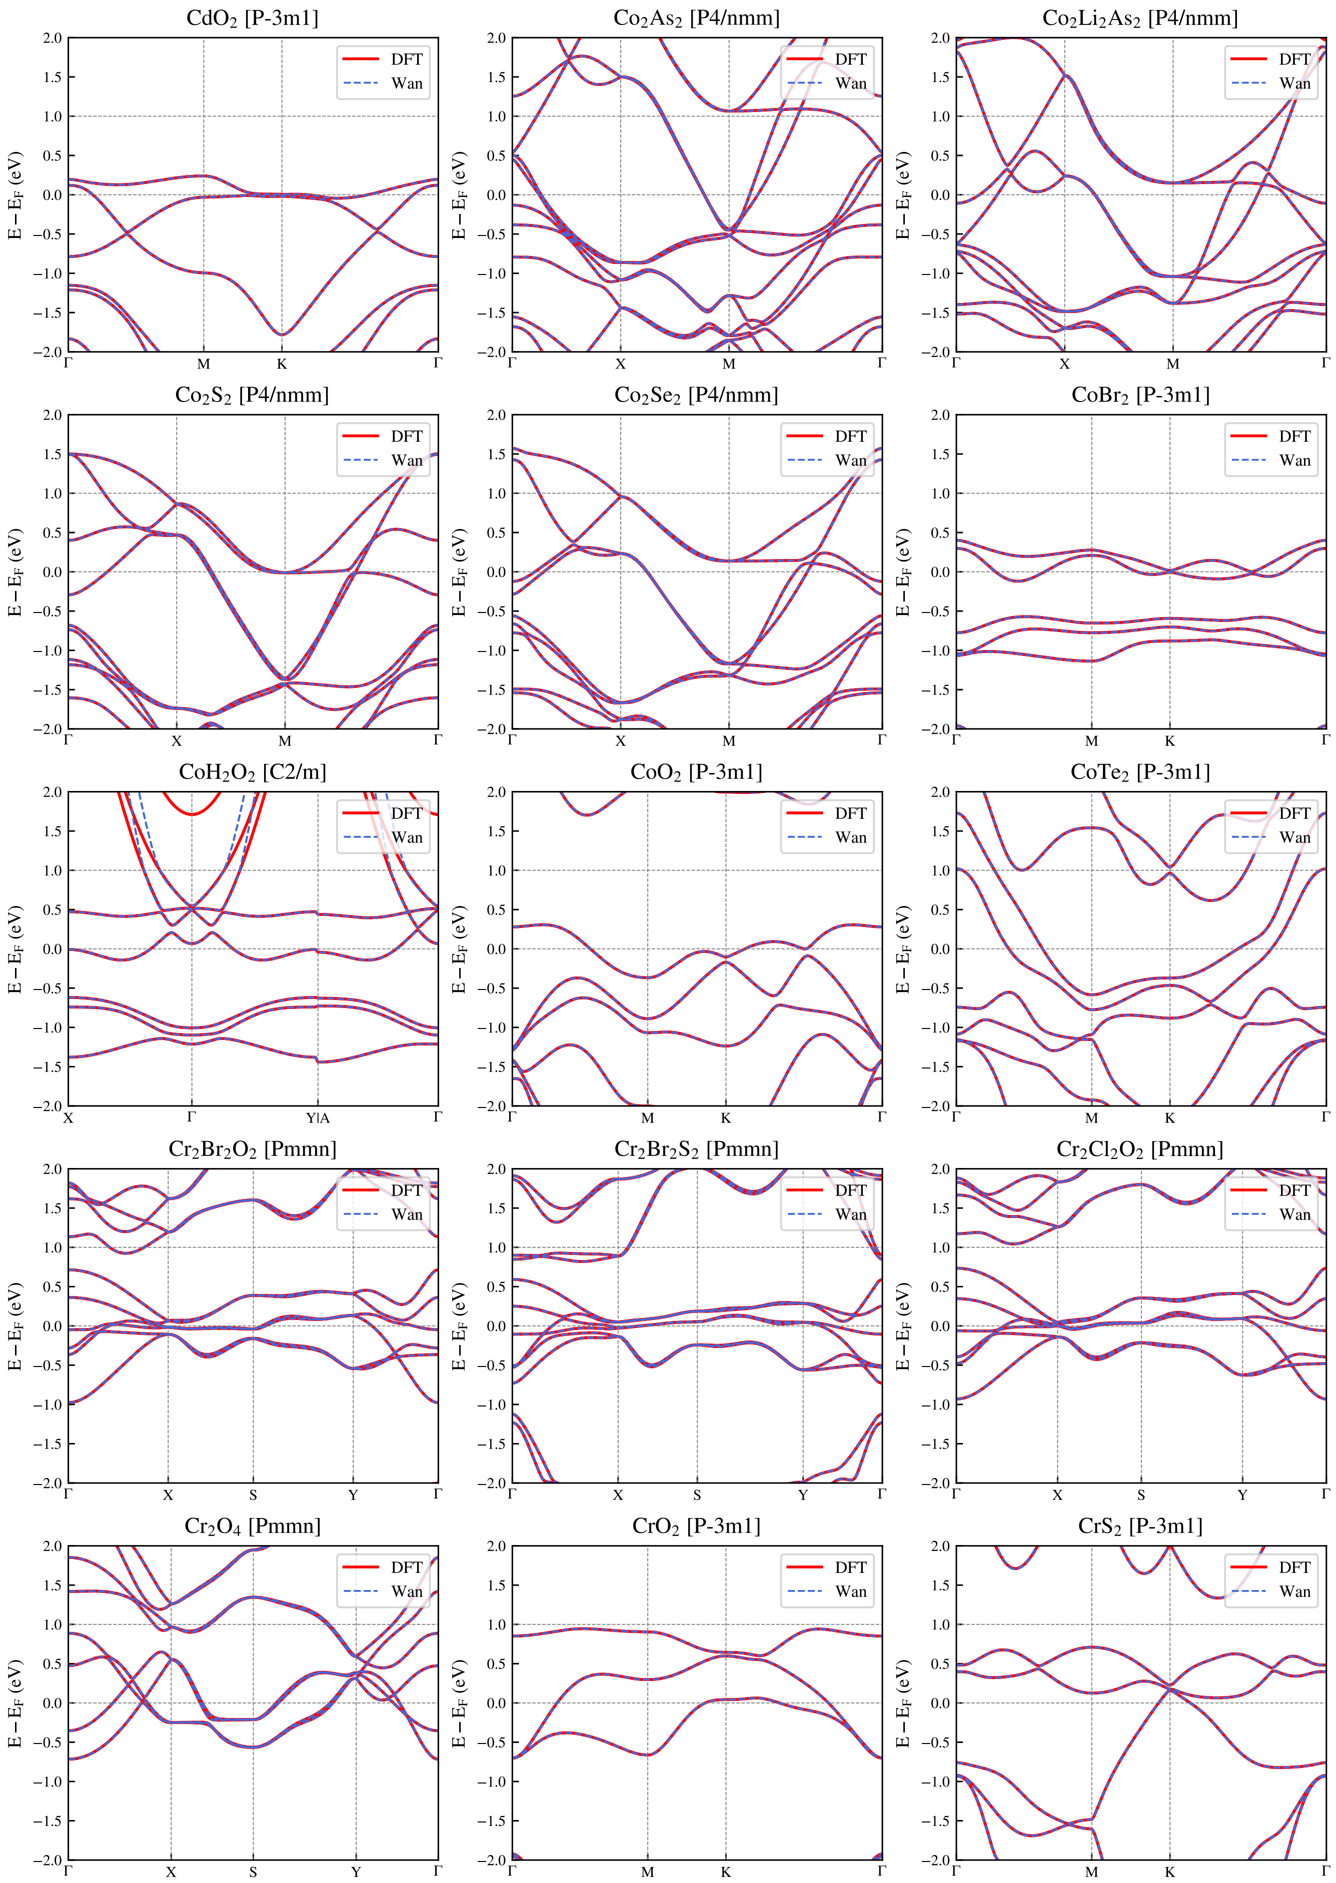

$CdO_2$ [P-3m1]
$Co_2As_2$ [P4/nmm]
$Co_2Li_2As_2$ [P4/nmm]
$Co_2S_2$ [P4/nmm]
$Co_2Se_2$ [P4/nmm]
$CoBr_2$ [P-3m1]
$CoH_2O_2$ [C2/m]
$CoO_2$ [P-3m1]
$CoTe_2$ [P-3m1]
$Cr_2Br_2O_2$ [Pmmn]
$Cr_2Br_2S_2$ [Pmmn]
$Cr_2Cl_2O_2$ [Pmmn]
$Cr_2O_4$ [Pmmn]
$CrO_2$ [P-3m1]
$CrS_2$ [P-3m1]
DFT
Wan
$E - E_F$ (eV)

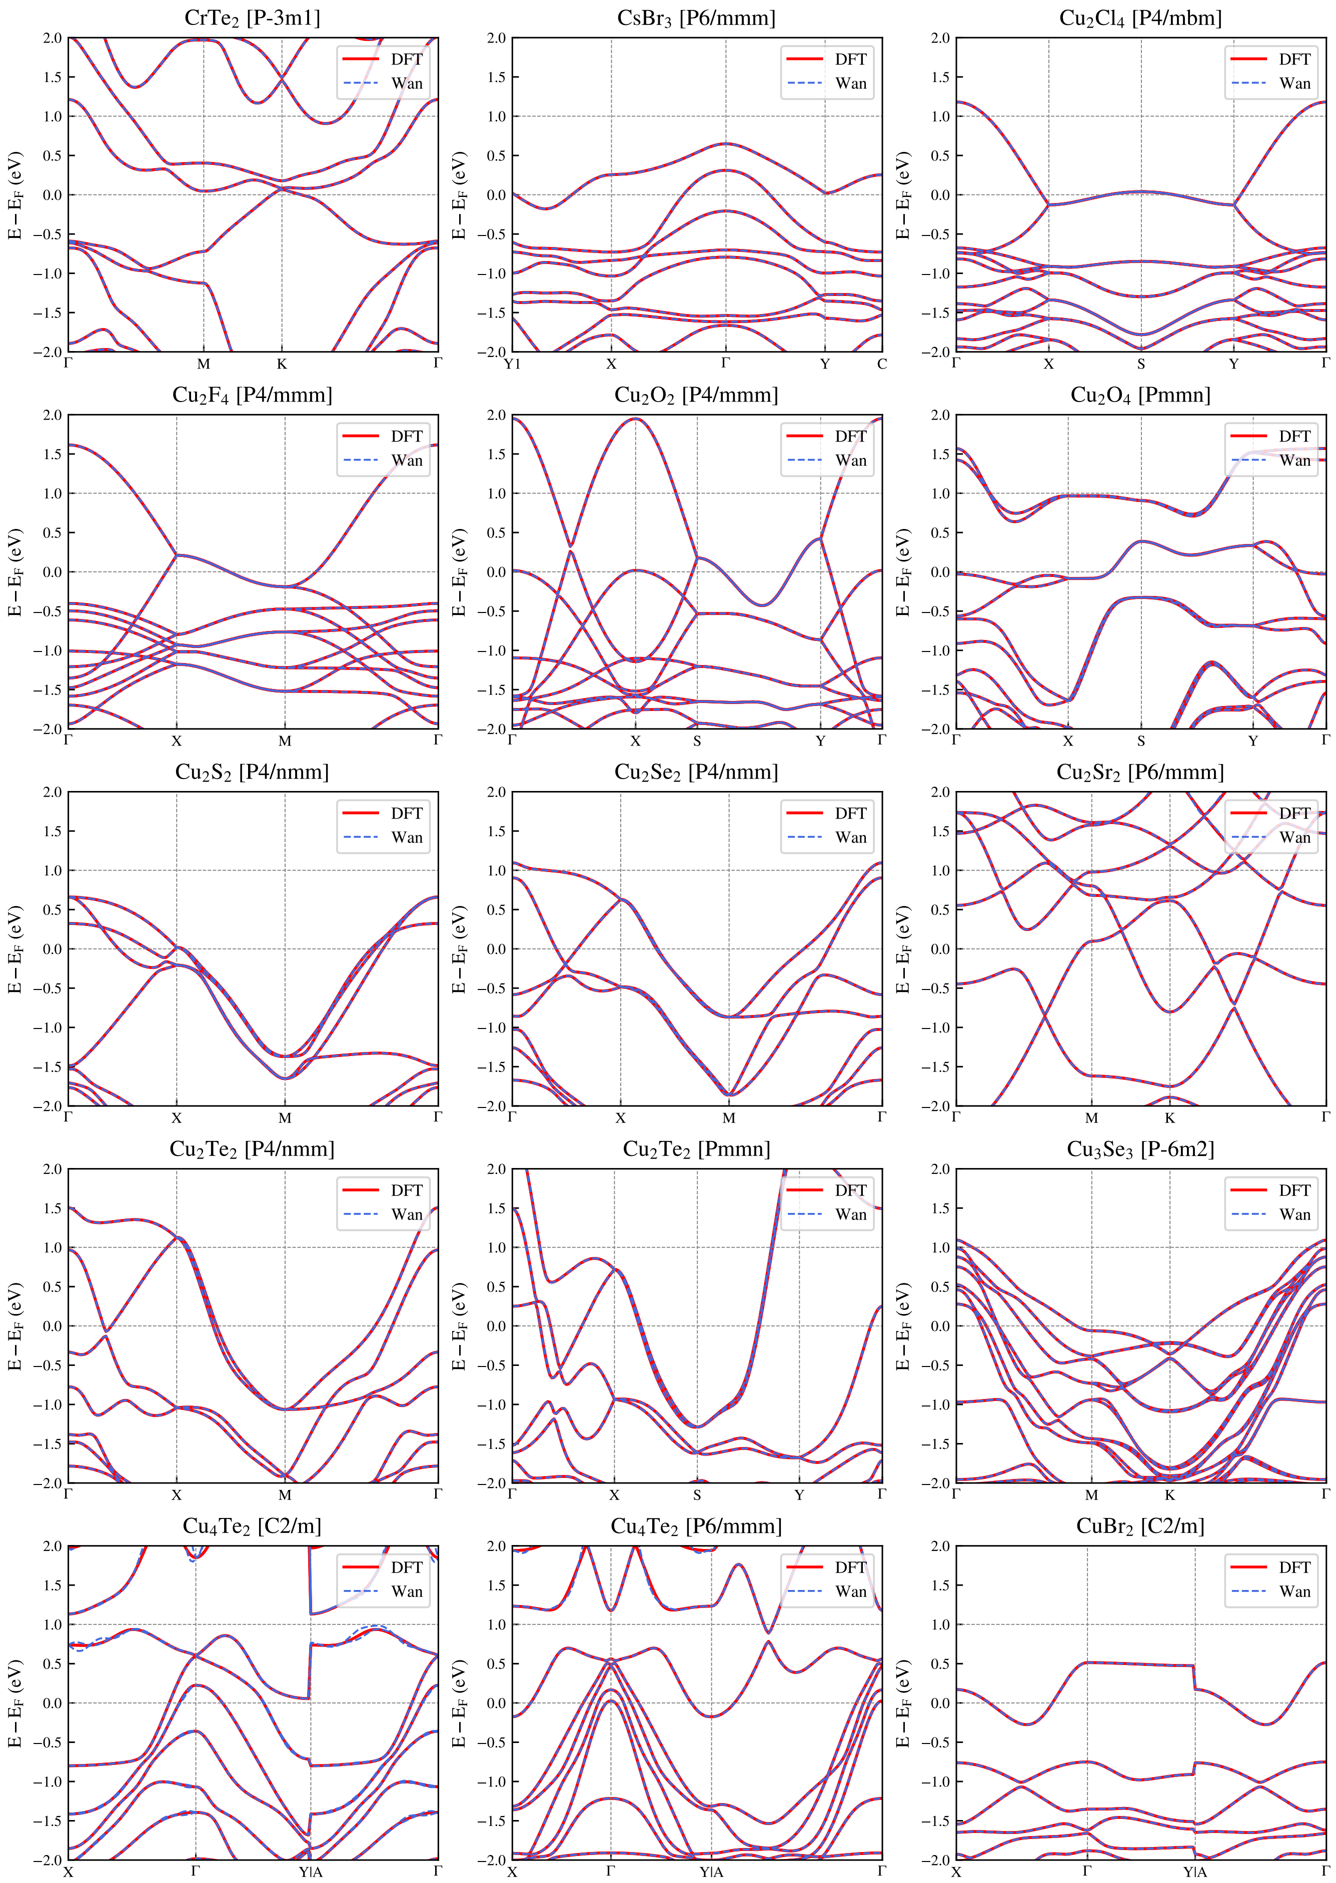
CrTe₂ [P-3m1]
CsBr₃ [P6/mmm]
Cu₂Cl₄ [P4/mbm]
Cu₂F₄ [P4/mmm]
Cu₂O₂ [P4/mmm]
Cu₂O₄ [Pmmn]
Cu₂S₂ [P4/nmm]
Cu₂Se₂ [P4/nmm]
Cu₂Sr₂ [P6/mmm]
Cu₂Te₂ [P4/nmm]
Cu₂Te₂ [Pmmn]
Cu₃Se₃ [P-6m2]
Cu₄Te₂ [C2/m]
Cu₄Te₂ [P6/mmm]
CuBr₂ [C2/m]
DFT
Wan
E − E_F (eV)

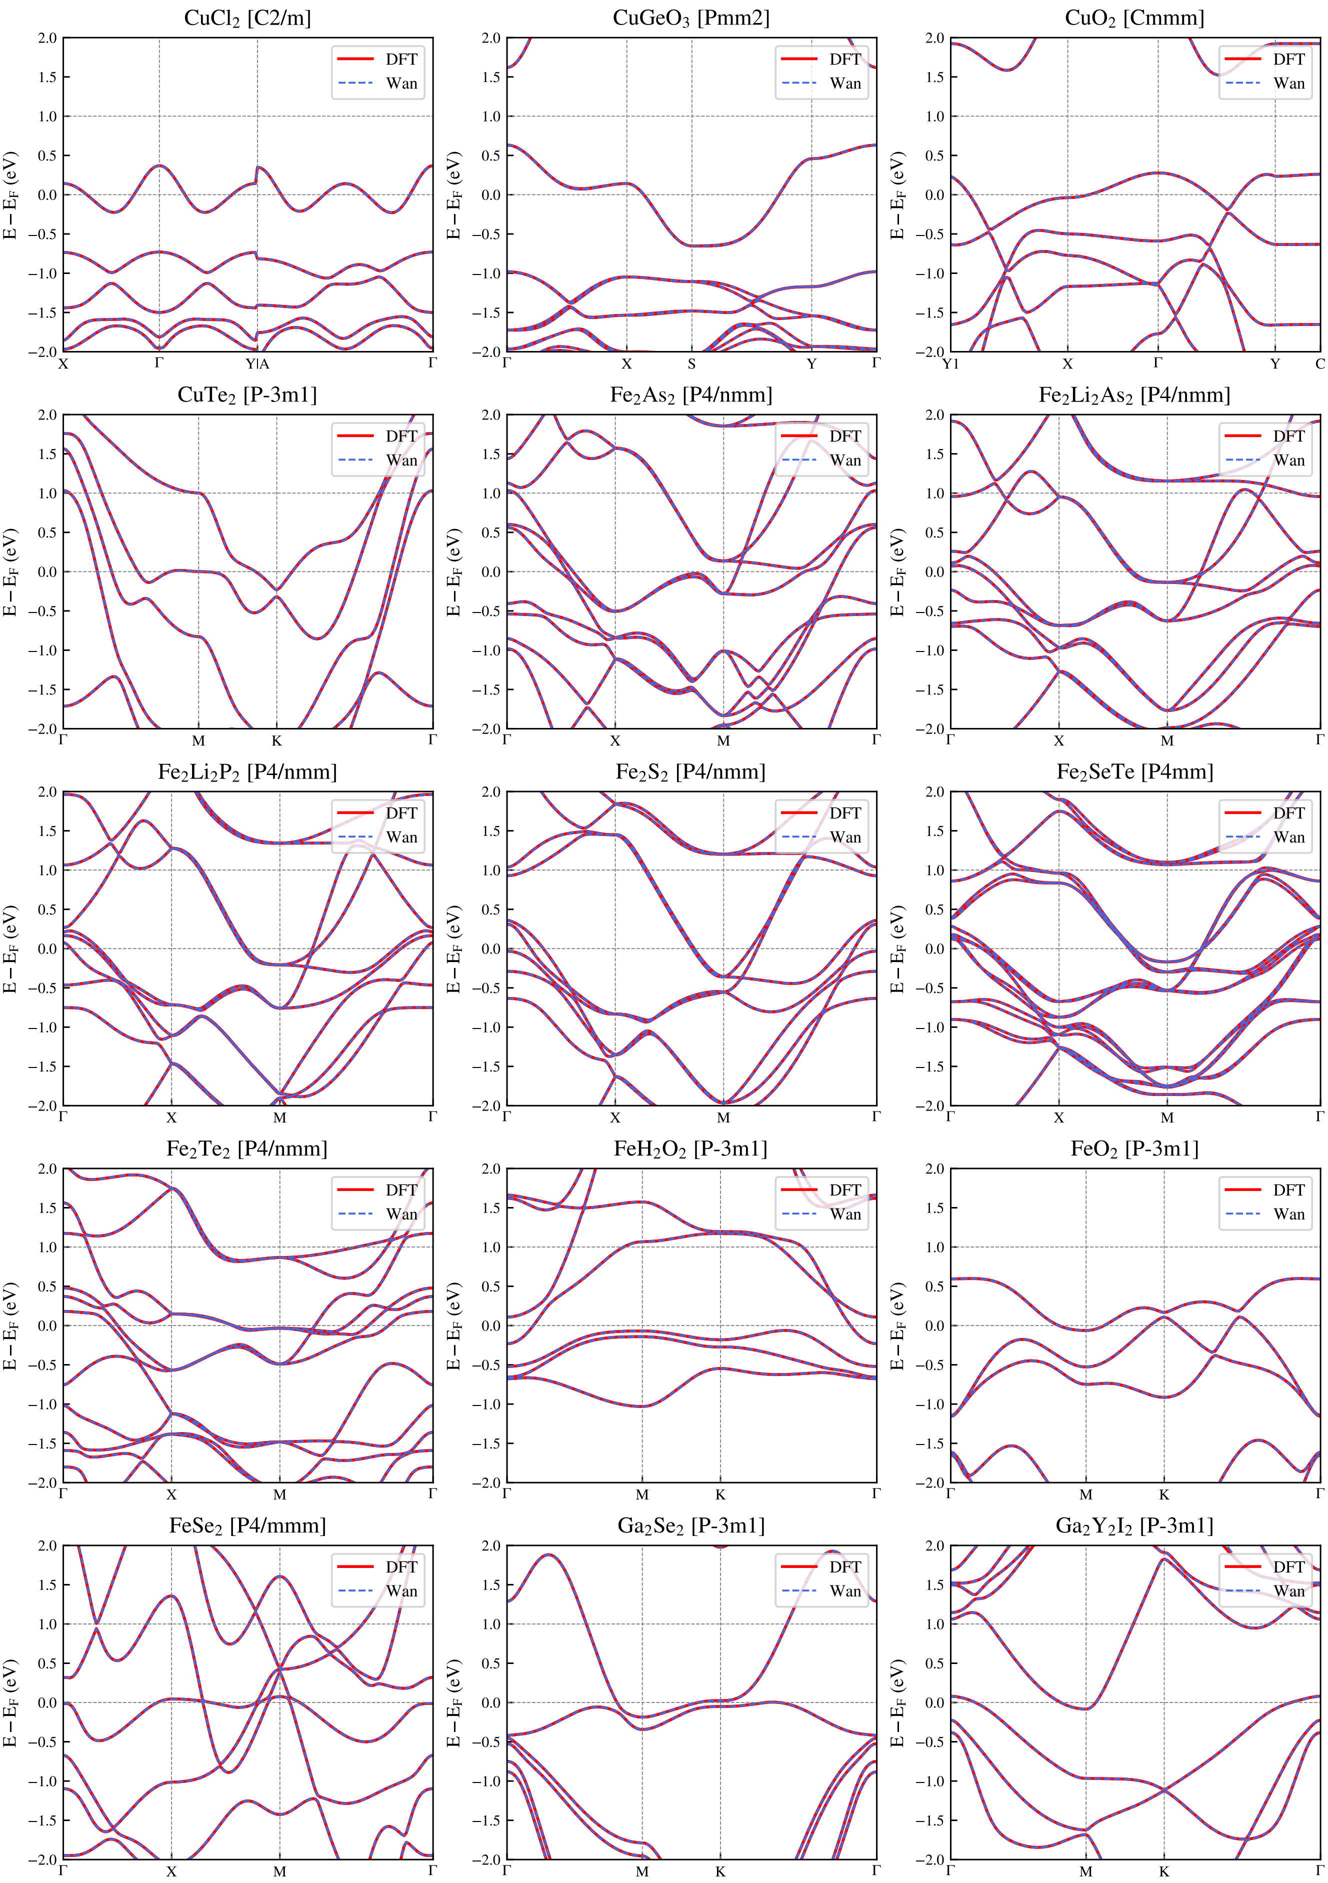
CuCl2 [C2/m]
CuGeO3 [Pmm2]
CuO2 [Cmmm]
CuTe2 [P-3m1]
Fe2As2 [P4/nmm]
Fe2Li2As2 [P4/nmm]
Fe2Li2P2 [P4/nmm]
Fe2S2 [P4/nmm]
Fe2SeTe [P4mm]
Fe2Te2 [P4/nmm]
FeH2O2 [P-3m1]
FeO2 [P-3m1]
FeSe2 [P4/mmm]
Ga2Se2 [P-3m1]
Ga2Y2I2 [P-3m1]
DFT
Wan
E − EF (eV)
X Γ Y|A Γ
Γ X S Y Γ
Y1 X Γ Y C
Γ M K Γ
Γ X M Γ

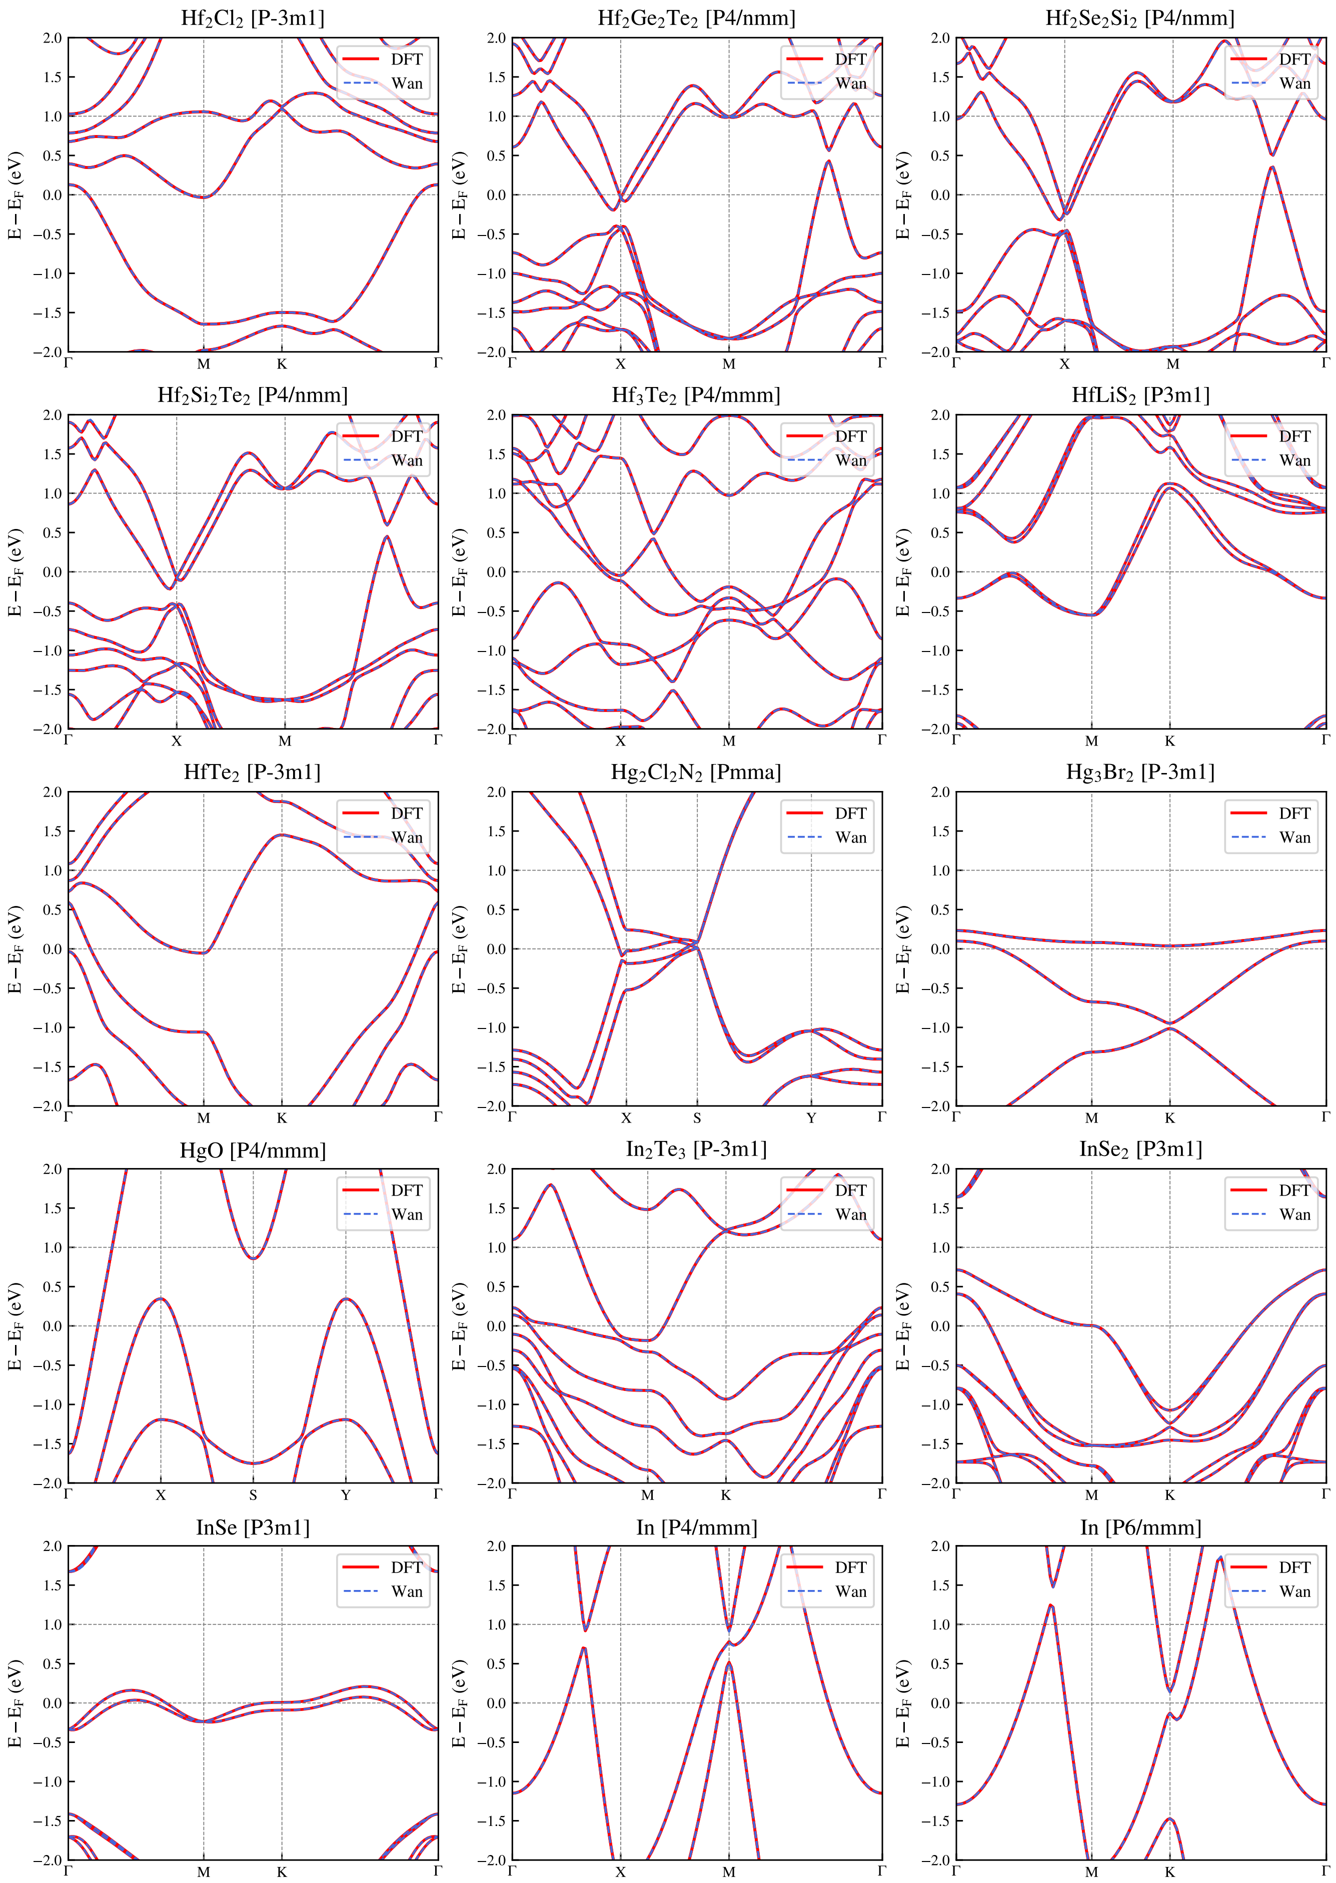
$Hf_2Cl_2$ [P-3m1]
$Hf_2Ge_2Te_2$ [P4/nmm]
$Hf_2Se_2Si_2$ [P4/nmm]
$Hf_2Si_2Te_2$ [P4/nmm]
$Hf_3Te_2$ [P4/mmm]
$HfLiS_2$ [P3m1]
$HfTe_2$ [P-3m1]
$Hg_2Cl_2N_2$ [Pmma]
$Hg_3Br_2$ [P-3m1]
HgO [P4/mmm]
$In_2Te_3$ [P-3m1]
$InSe_2$ [P3m1]
InSe [P3m1]
In [P4/mmm]
In [P6/mmm]
DFT
Wan
$E - E_F$ (eV)
Γ
M
K
X
S
Y

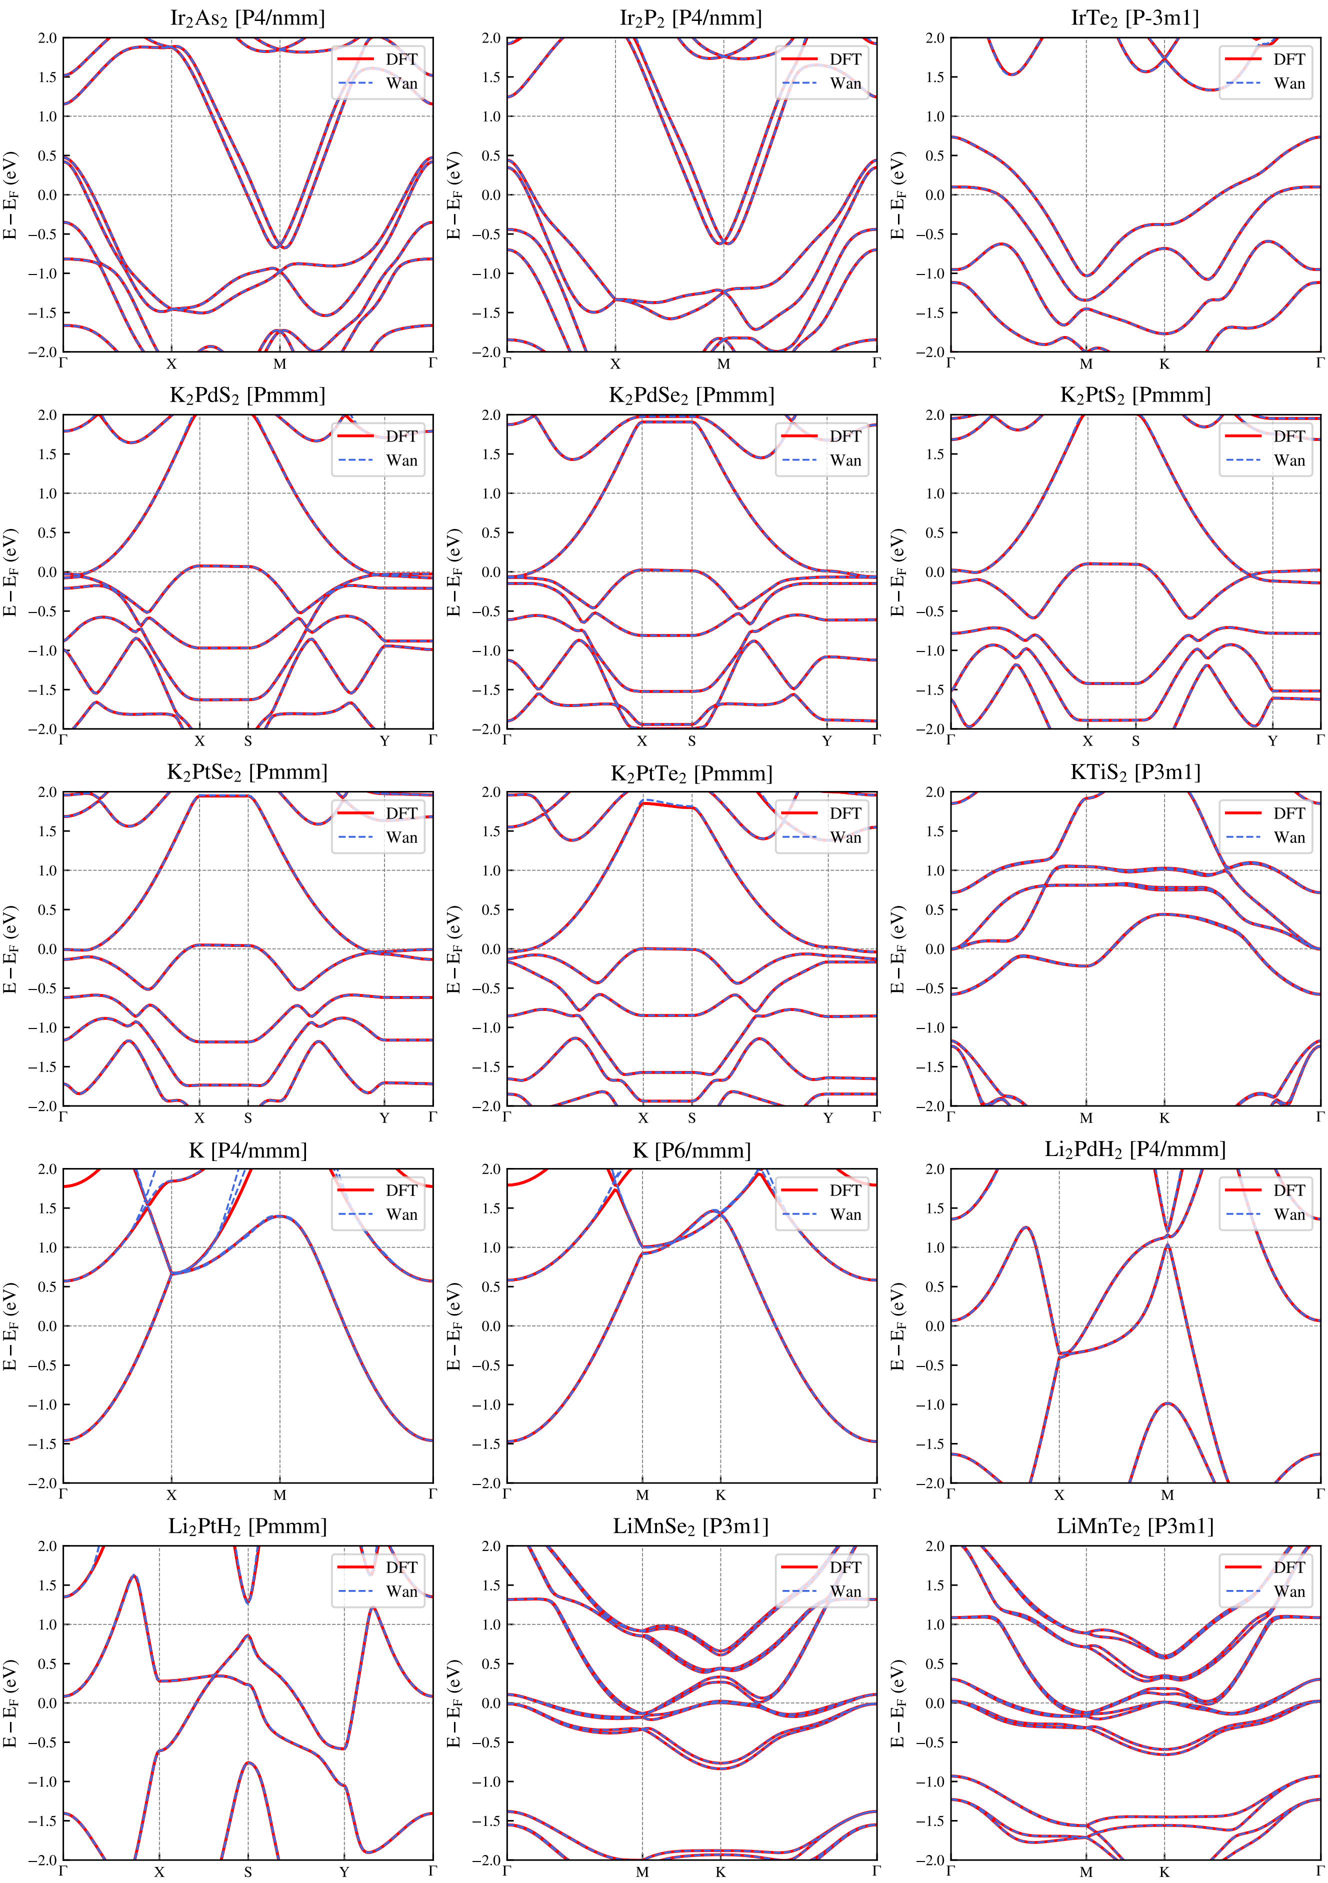
Ir2As2 [P4/nmm]
Ir2P2 [P4/nmm]
IrTe2 [P-3m1]
K2PdS2 [Pmmm]
K2PdSe2 [Pmmm]
K2PtS2 [Pmmm]
K2PtSe2 [Pmmm]
K2PtTe2 [Pmmm]
KTiS2 [P3m1]
K [P4/mmm]
K [P6/mmm]
Li2PdH2 [P4/mmm]
Li2PtH2 [Pmmm]
LiMnSe2 [P3m1]
LiMnTe2 [P3m1]
DFT
Wan
E − EF (eV)
Γ
X
M
K
S
Y

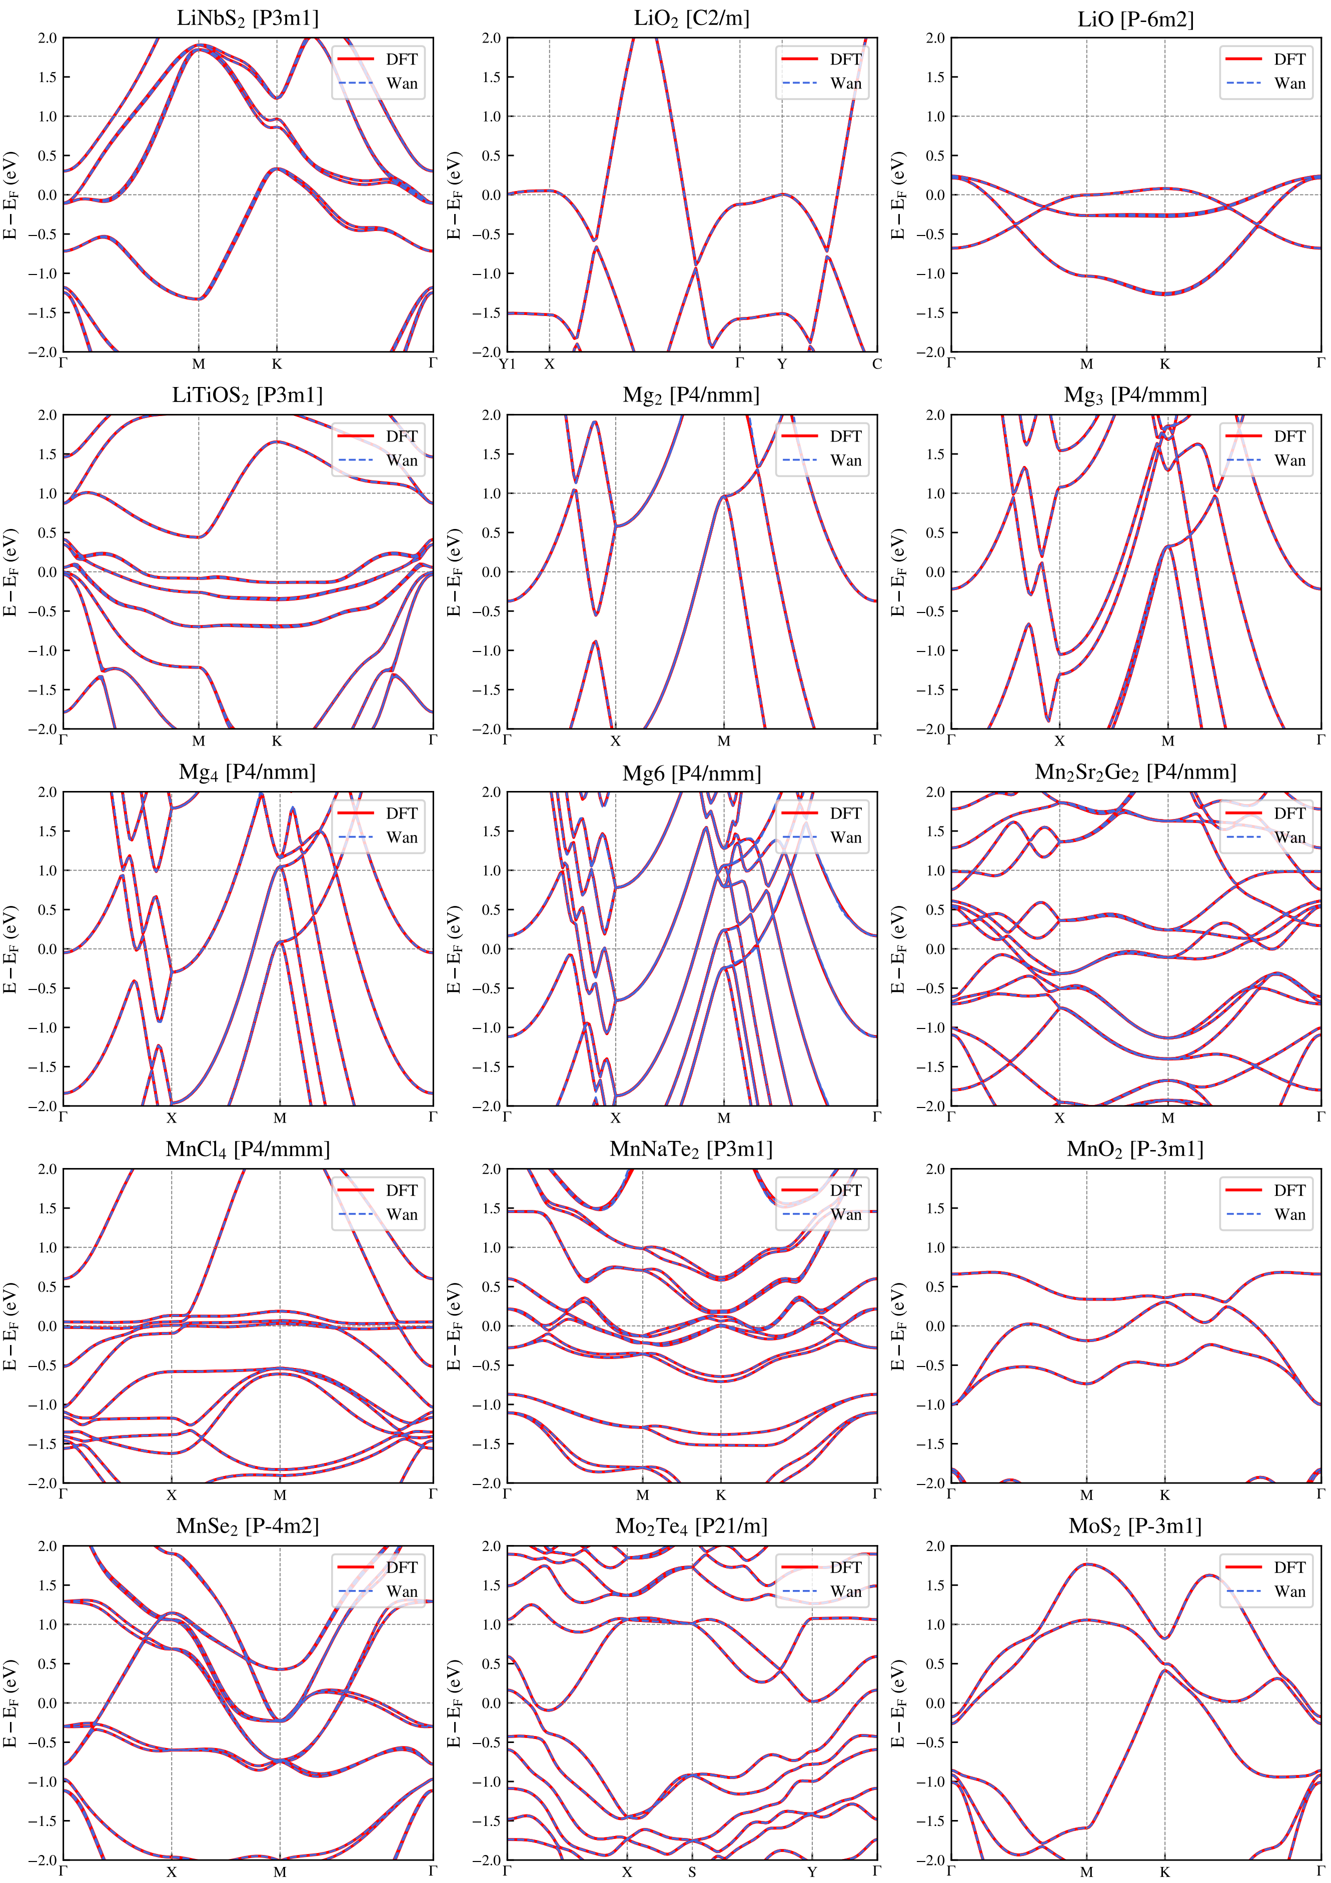
LiNbS2 [P3m1]
Γ M K Γ
LiO2 [C2/m]
Y1 X Γ Y C
LiO [P-6m2]
Γ M K Γ
LiTiOS2 [P3m1]
Γ M K Γ
Mg2 [P4/nmm]
Γ X M Γ
Mg3 [P4/mmm]
Γ X M Γ
Mg4 [P4/nmm]
Γ X M Γ
Mg6 [P4/nmm]
Γ X M Γ
Mn2Sr2Ge2 [P4/nmm]
Γ X M Γ
MnCl4 [P4/mmm]
Γ X M Γ
MnNaTe2 [P3m1]
Γ M K Γ
MnO2 [P-3m1]
Γ M K Γ
MnSe2 [P-4m2]
Γ X M Γ
Mo2Te4 [P21/m]
Γ X S Y Γ
MoS2 [P-3m1]
Γ M K Γ
E − EF (eV)
DFT
Wan

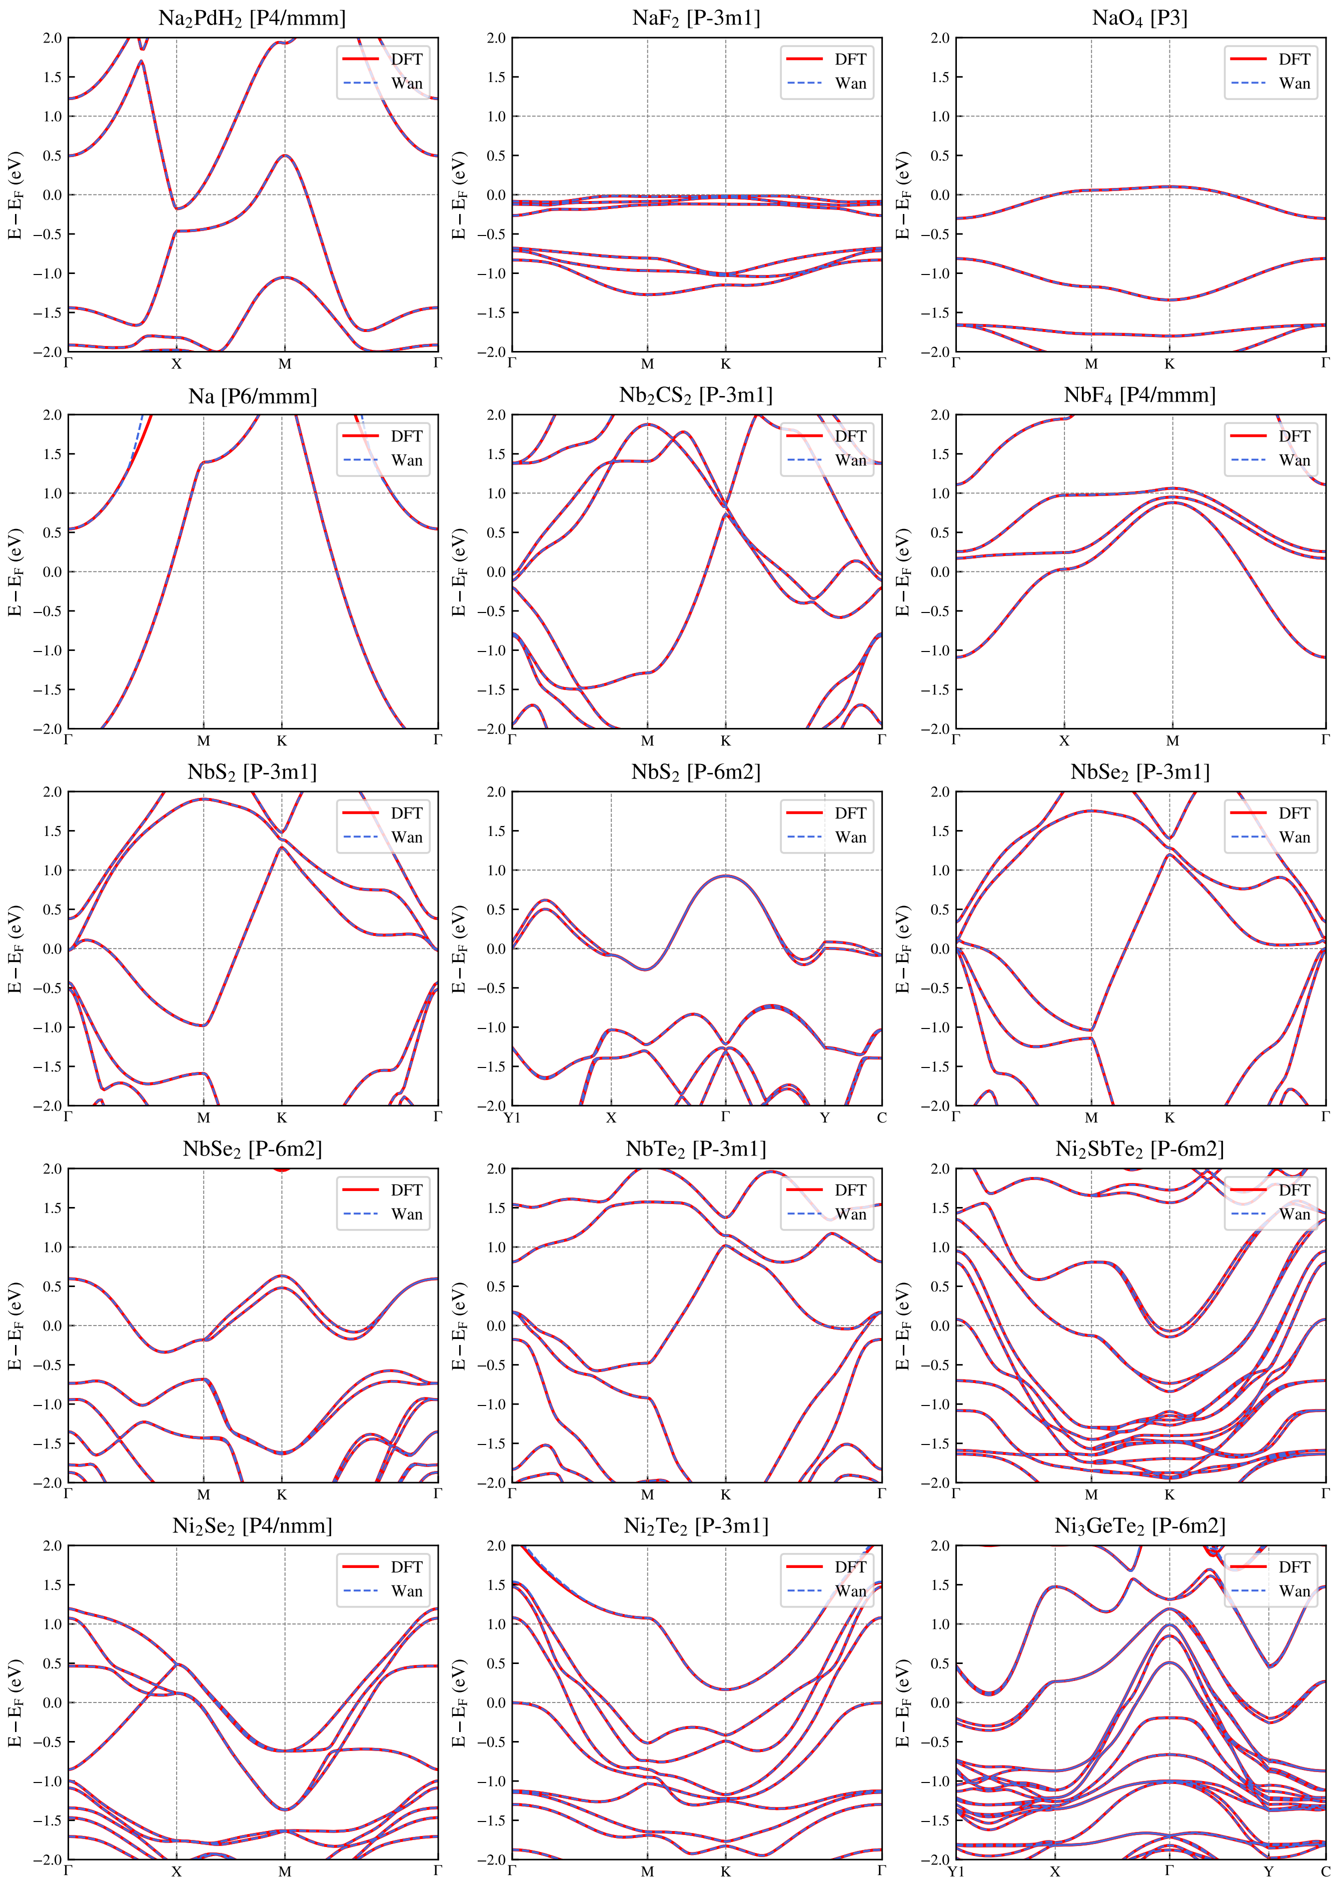
Na2PdH2 [P4/mmm]
NaF2 [P-3m1]
NaO4 [P3]
Na [P6/mmm]
Nb2CS2 [P-3m1]
NbF4 [P4/mmm]
NbS2 [P-3m1]
NbS2 [P-6m2]
NbSe2 [P-3m1]
NbSe2 [P-6m2]
NbTe2 [P-3m1]
Ni2SbTe2 [P-6m2]
Ni2Se2 [P4/nmm]
Ni2Te2 [P-3m1]
Ni3GeTe2 [P-6m2]
DFT
Wan
E − EF (eV)
Γ
X
M
K
Y1
Y
C

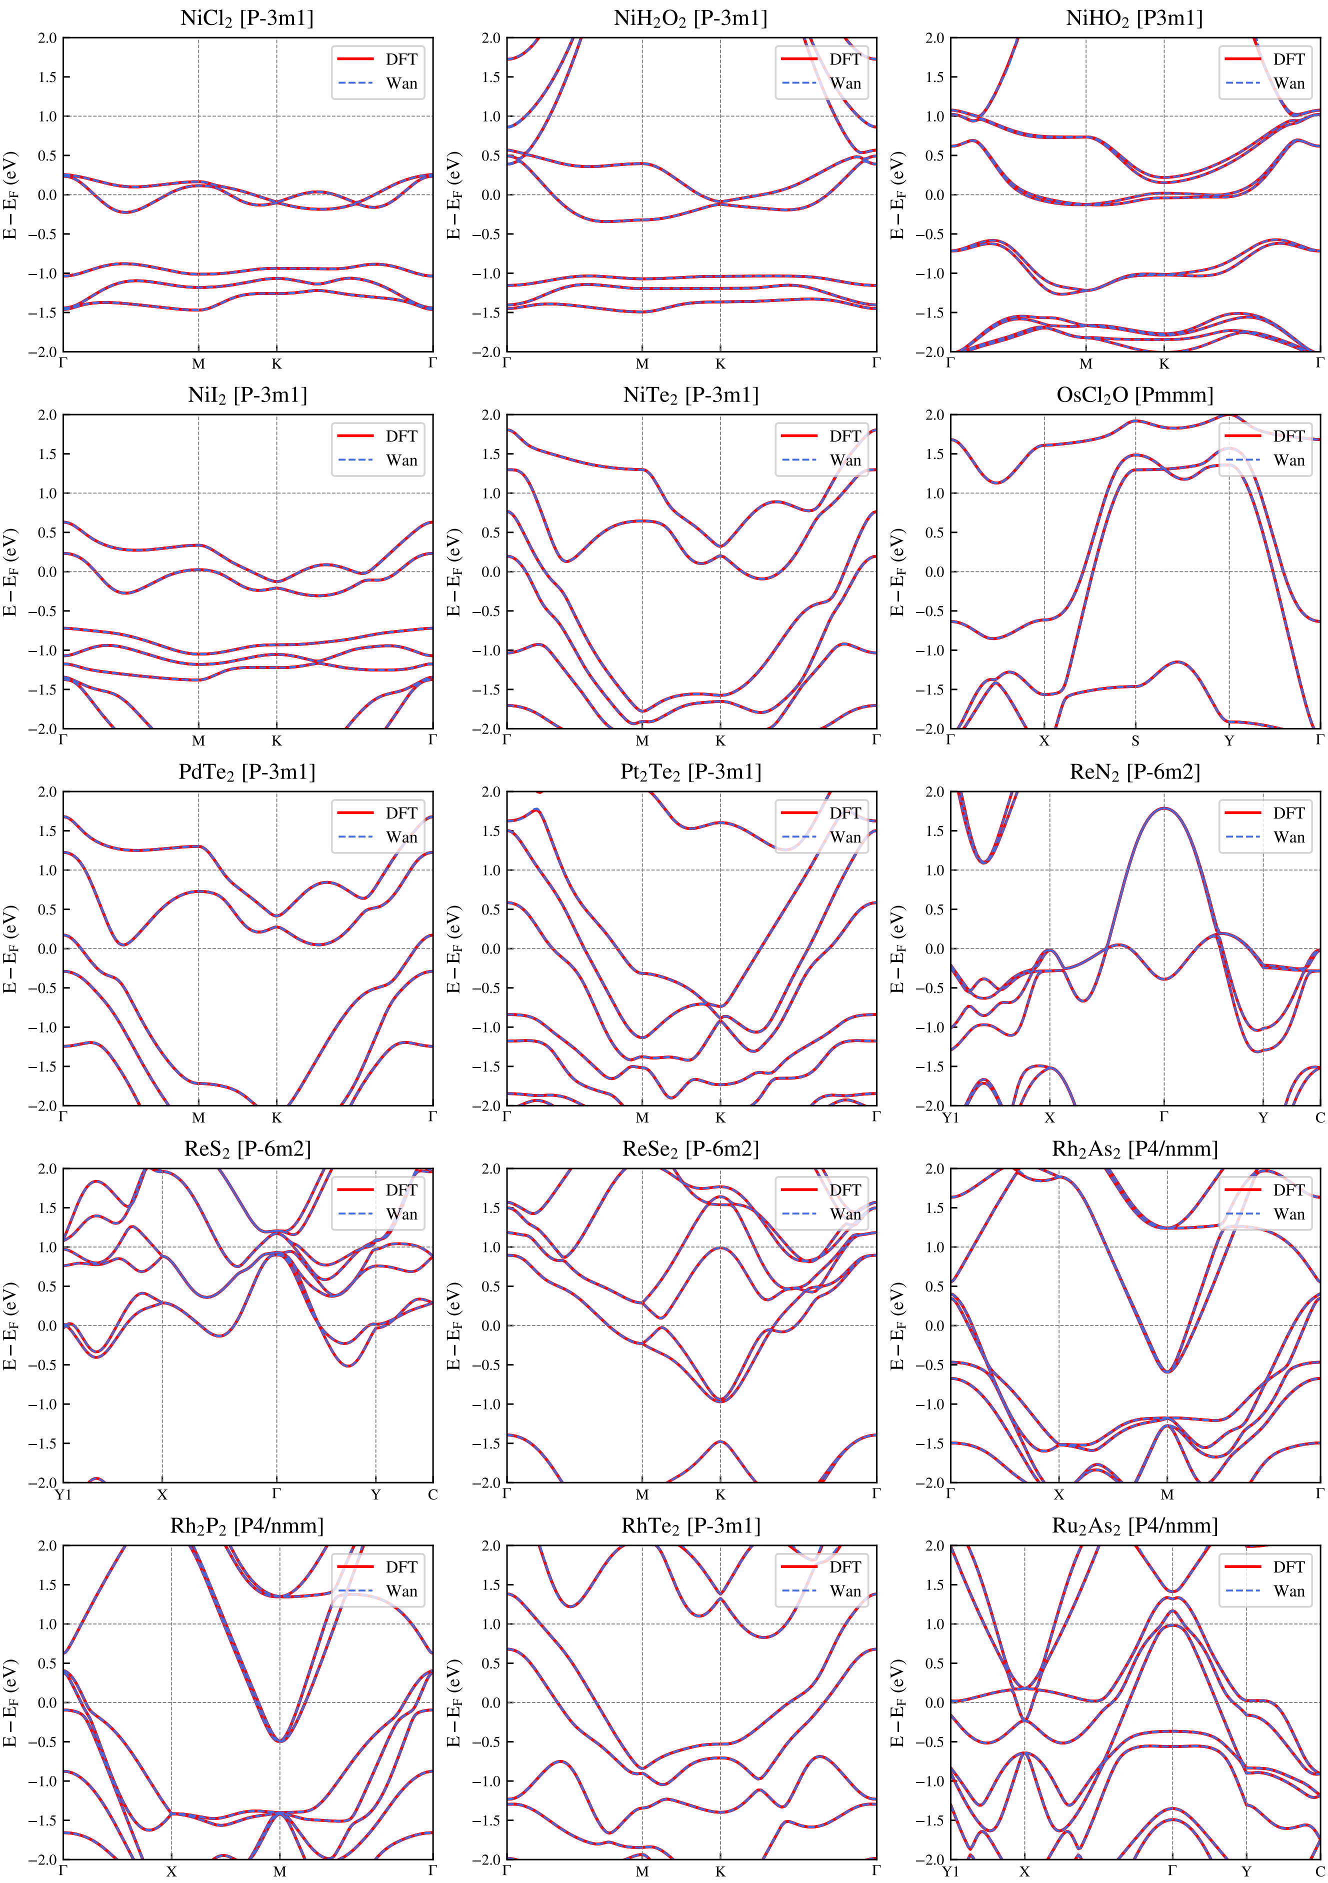
NiCl$_2$ [P-3m1]
NiH$_2$O$_2$ [P-3m1]
NiHO$_2$ [P3m1]
NiI$_2$ [P-3m1]
NiTe$_2$ [P-3m1]
OsCl$_2$O [Pmmm]
PdTe$_2$ [P-3m1]
Pt$_2$Te$_2$ [P-3m1]
ReN$_2$ [P-6m2]
ReS$_2$ [P-6m2]
ReSe$_2$ [P-6m2]
Rh$_2$As$_2$ [P4/nmm]
Rh$_2$P$_2$ [P4/nmm]
RhTe$_2$ [P-3m1]
Ru$_2$As$_2$ [P4/nmm]
DFT
Wan
$E - E_F$ (eV)
Γ M K Γ
Γ X S Y Γ
Y1 X Γ Y C
Γ X M Γ

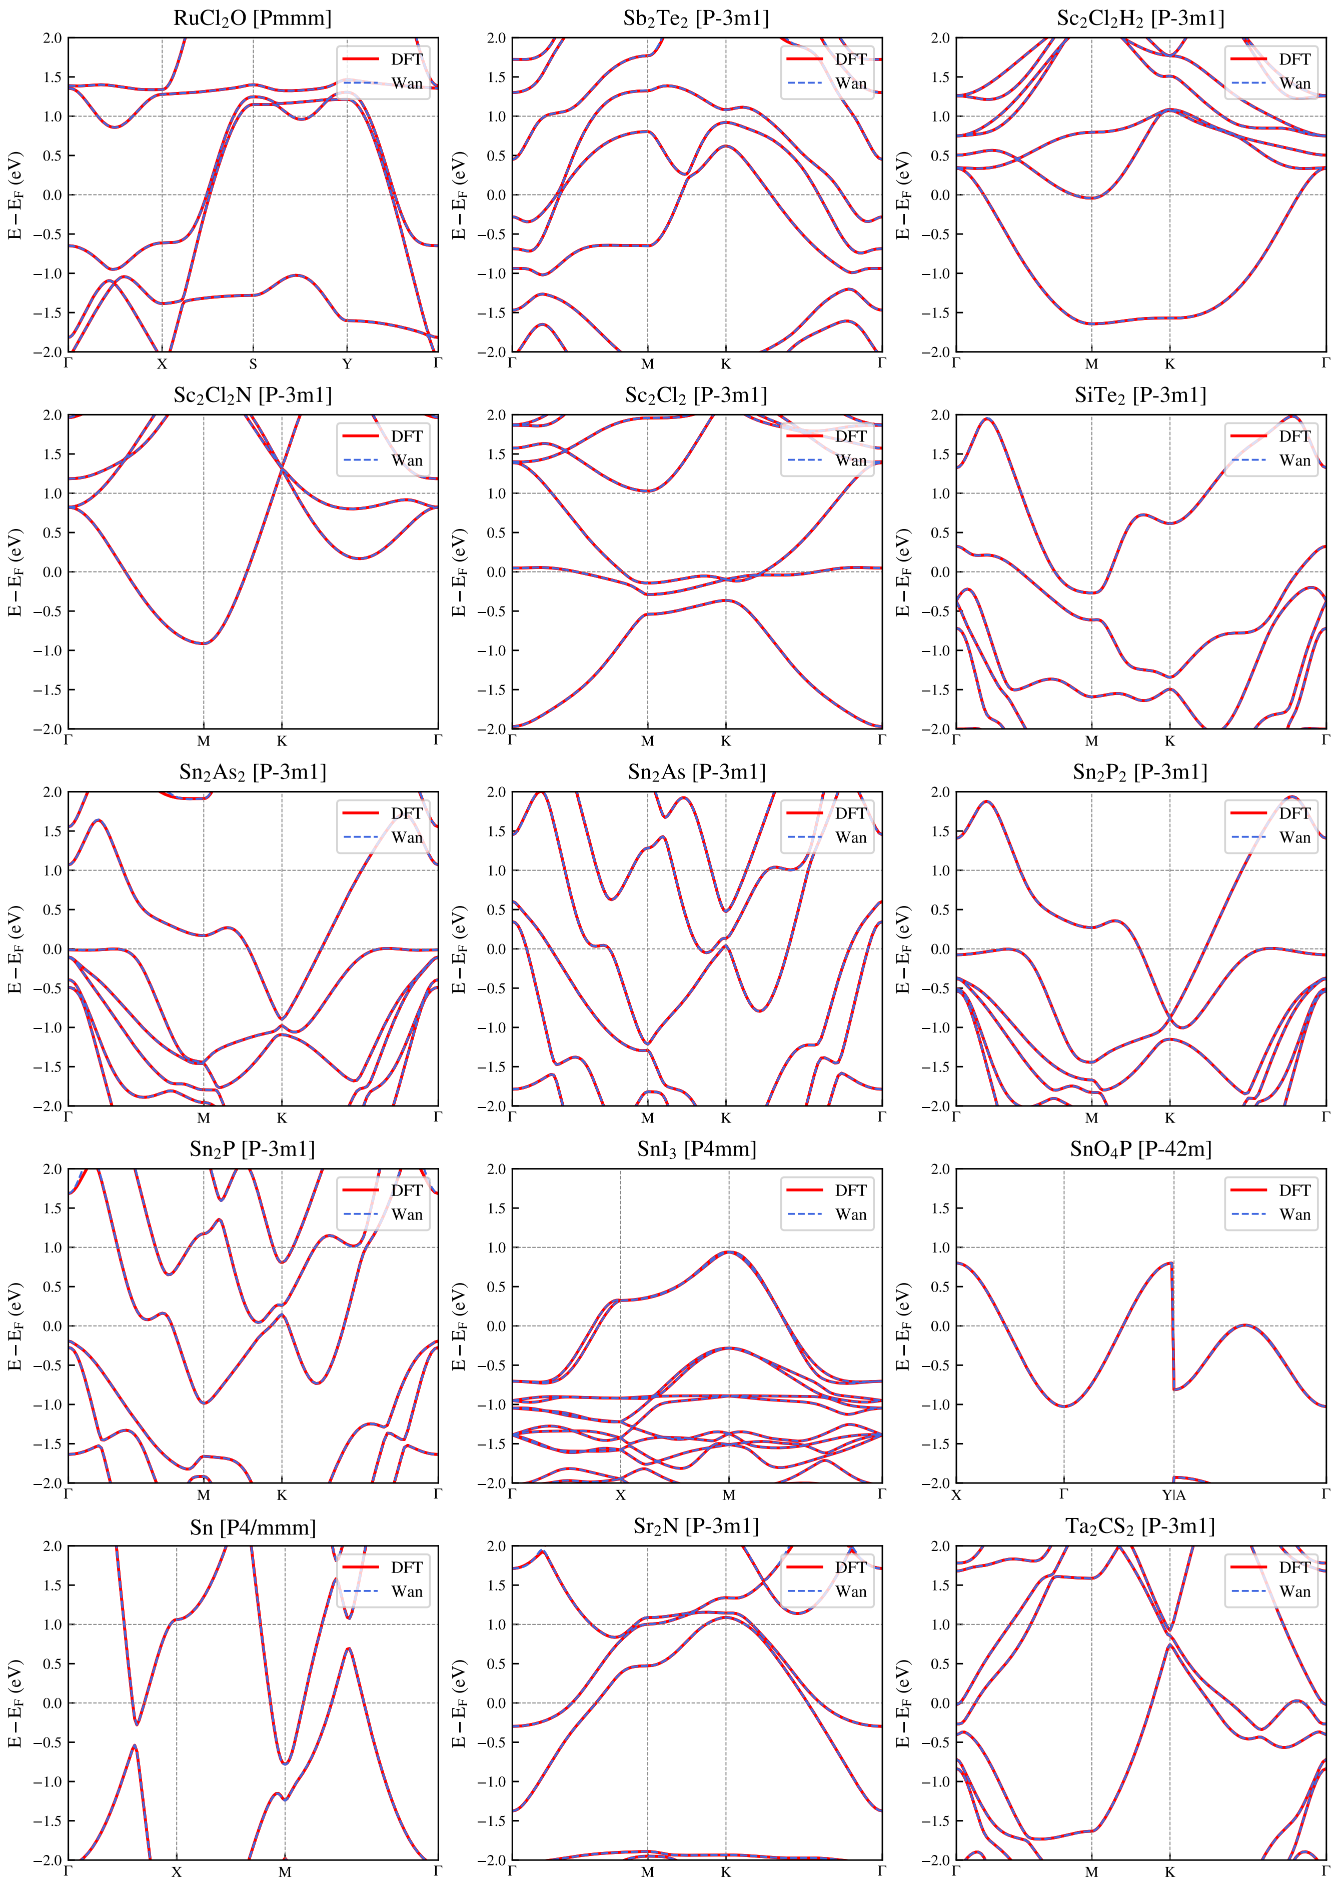
RuCl2O [Pmmm]
Sb2Te2 [P-3m1]
Sc2Cl2H2 [P-3m1]
Sc2Cl2N [P-3m1]
Sc2Cl2 [P-3m1]
SiTe2 [P-3m1]
Sn2As2 [P-3m1]
Sn2As [P-3m1]
Sn2P2 [P-3m1]
Sn2P [P-3m1]
SnI3 [P4mm]
SnO4P [P-42m]
Sn [P4/mmm]
Sr2N [P-3m1]
Ta2CS2 [P-3m1]
DFT
Wan
E − EF (eV)
Γ
X
S
Y
M
K
Y|A

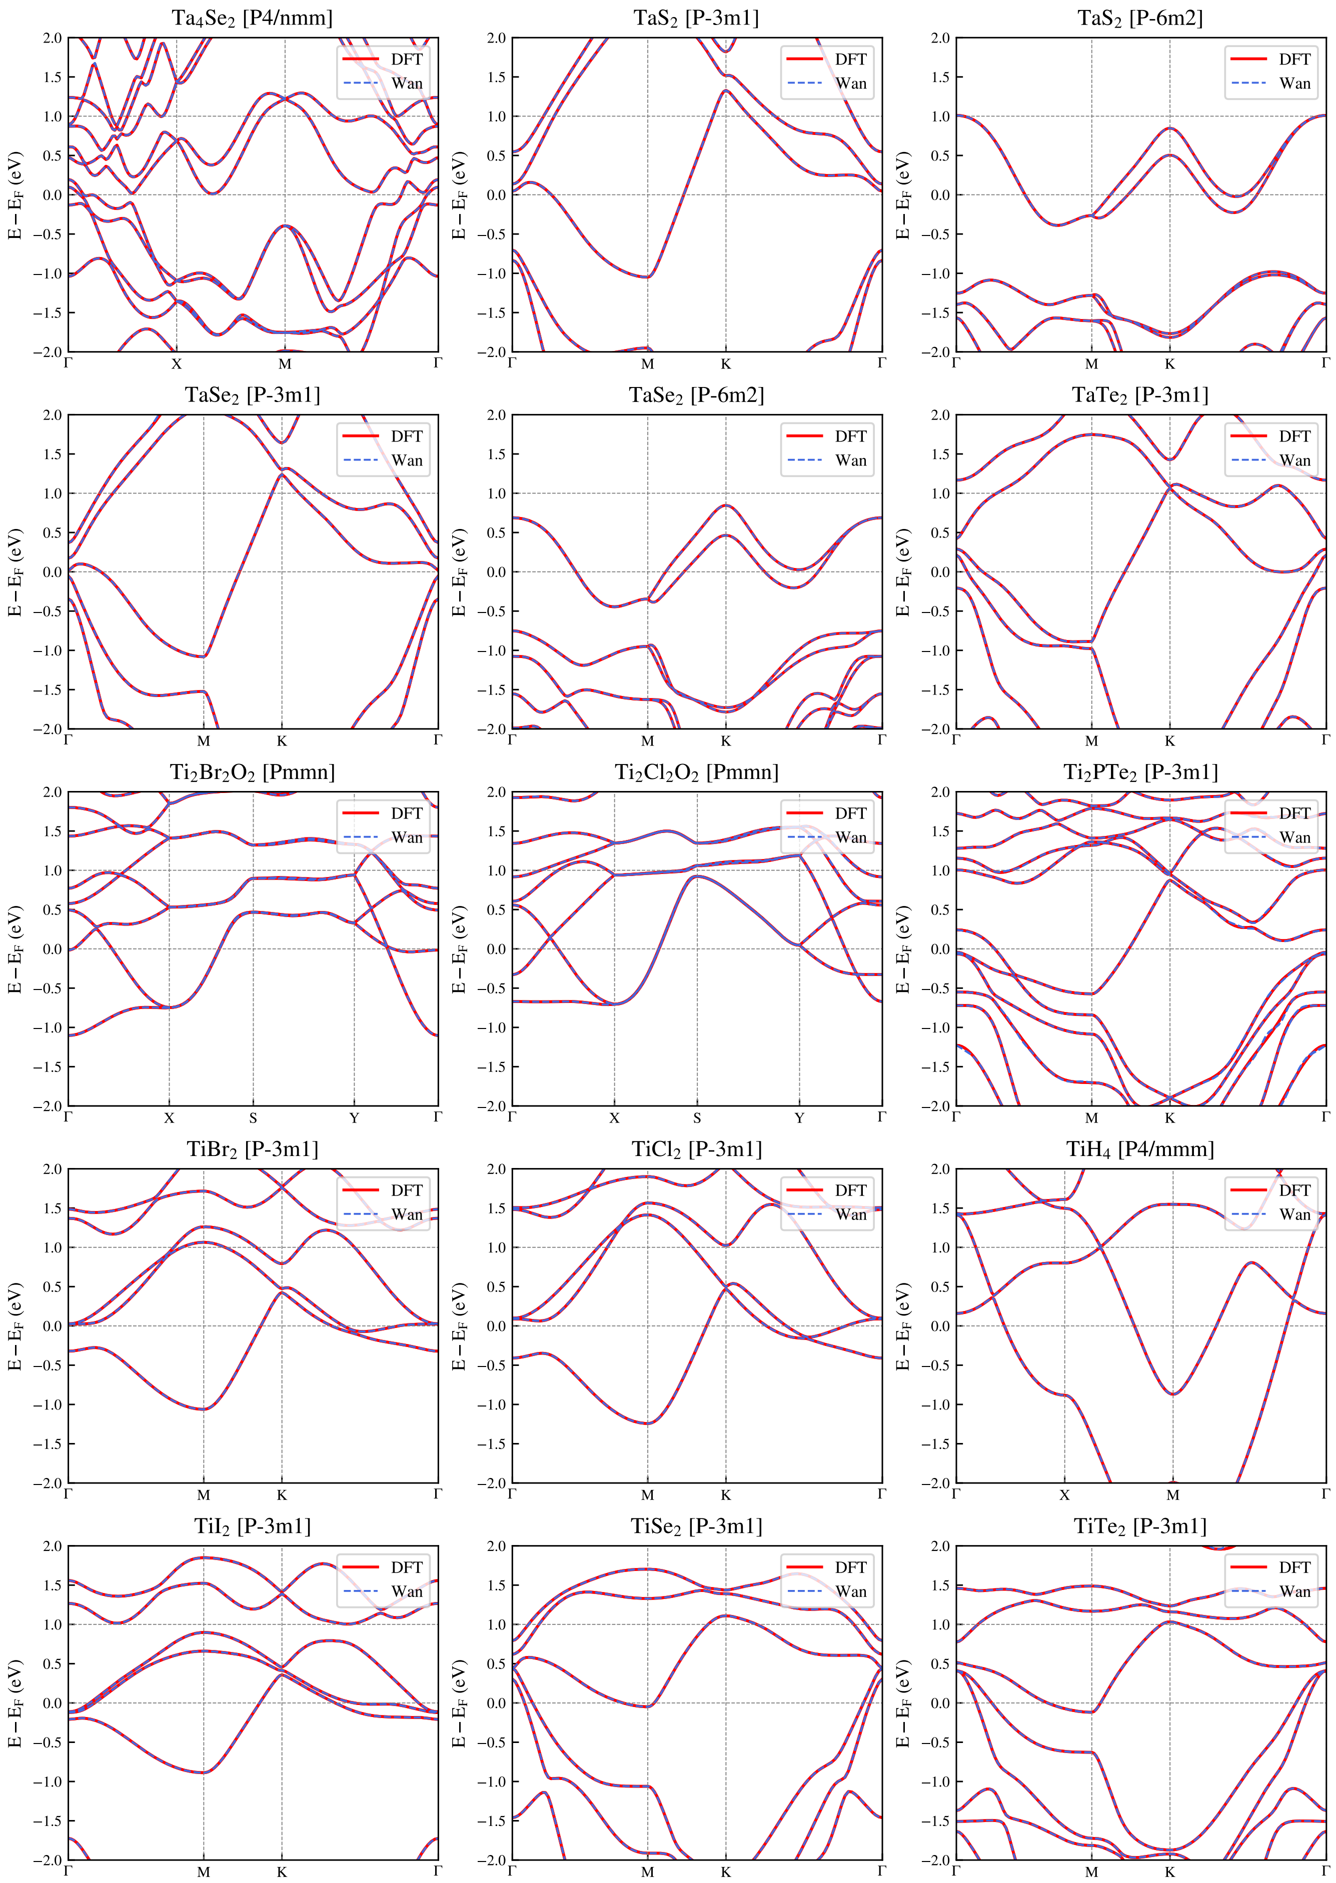
$Ta_4Se_2$ [P4/nmm]
$TaS_2$ [P-3m1]
$TaS_2$ [P-6m2]
$TaSe_2$ [P-3m1]
$TaSe_2$ [P-6m2]
$TaTe_2$ [P-3m1]
$Ti_2Br_2O_2$ [Pmmn]
$Ti_2Cl_2O_2$ [Pmmn]
$Ti_2PTe_2$ [P-3m1]
$TiBr_2$ [P-3m1]
$TiCl_2$ [P-3m1]
$TiH_4$ [P4/mmm]
$TiI_2$ [P-3m1]
$TiSe_2$ [P-3m1]
$TiTe_2$ [P-3m1]
DFT
Wan
$E - E_F$ (eV)
Γ
X
M
K
S
Y

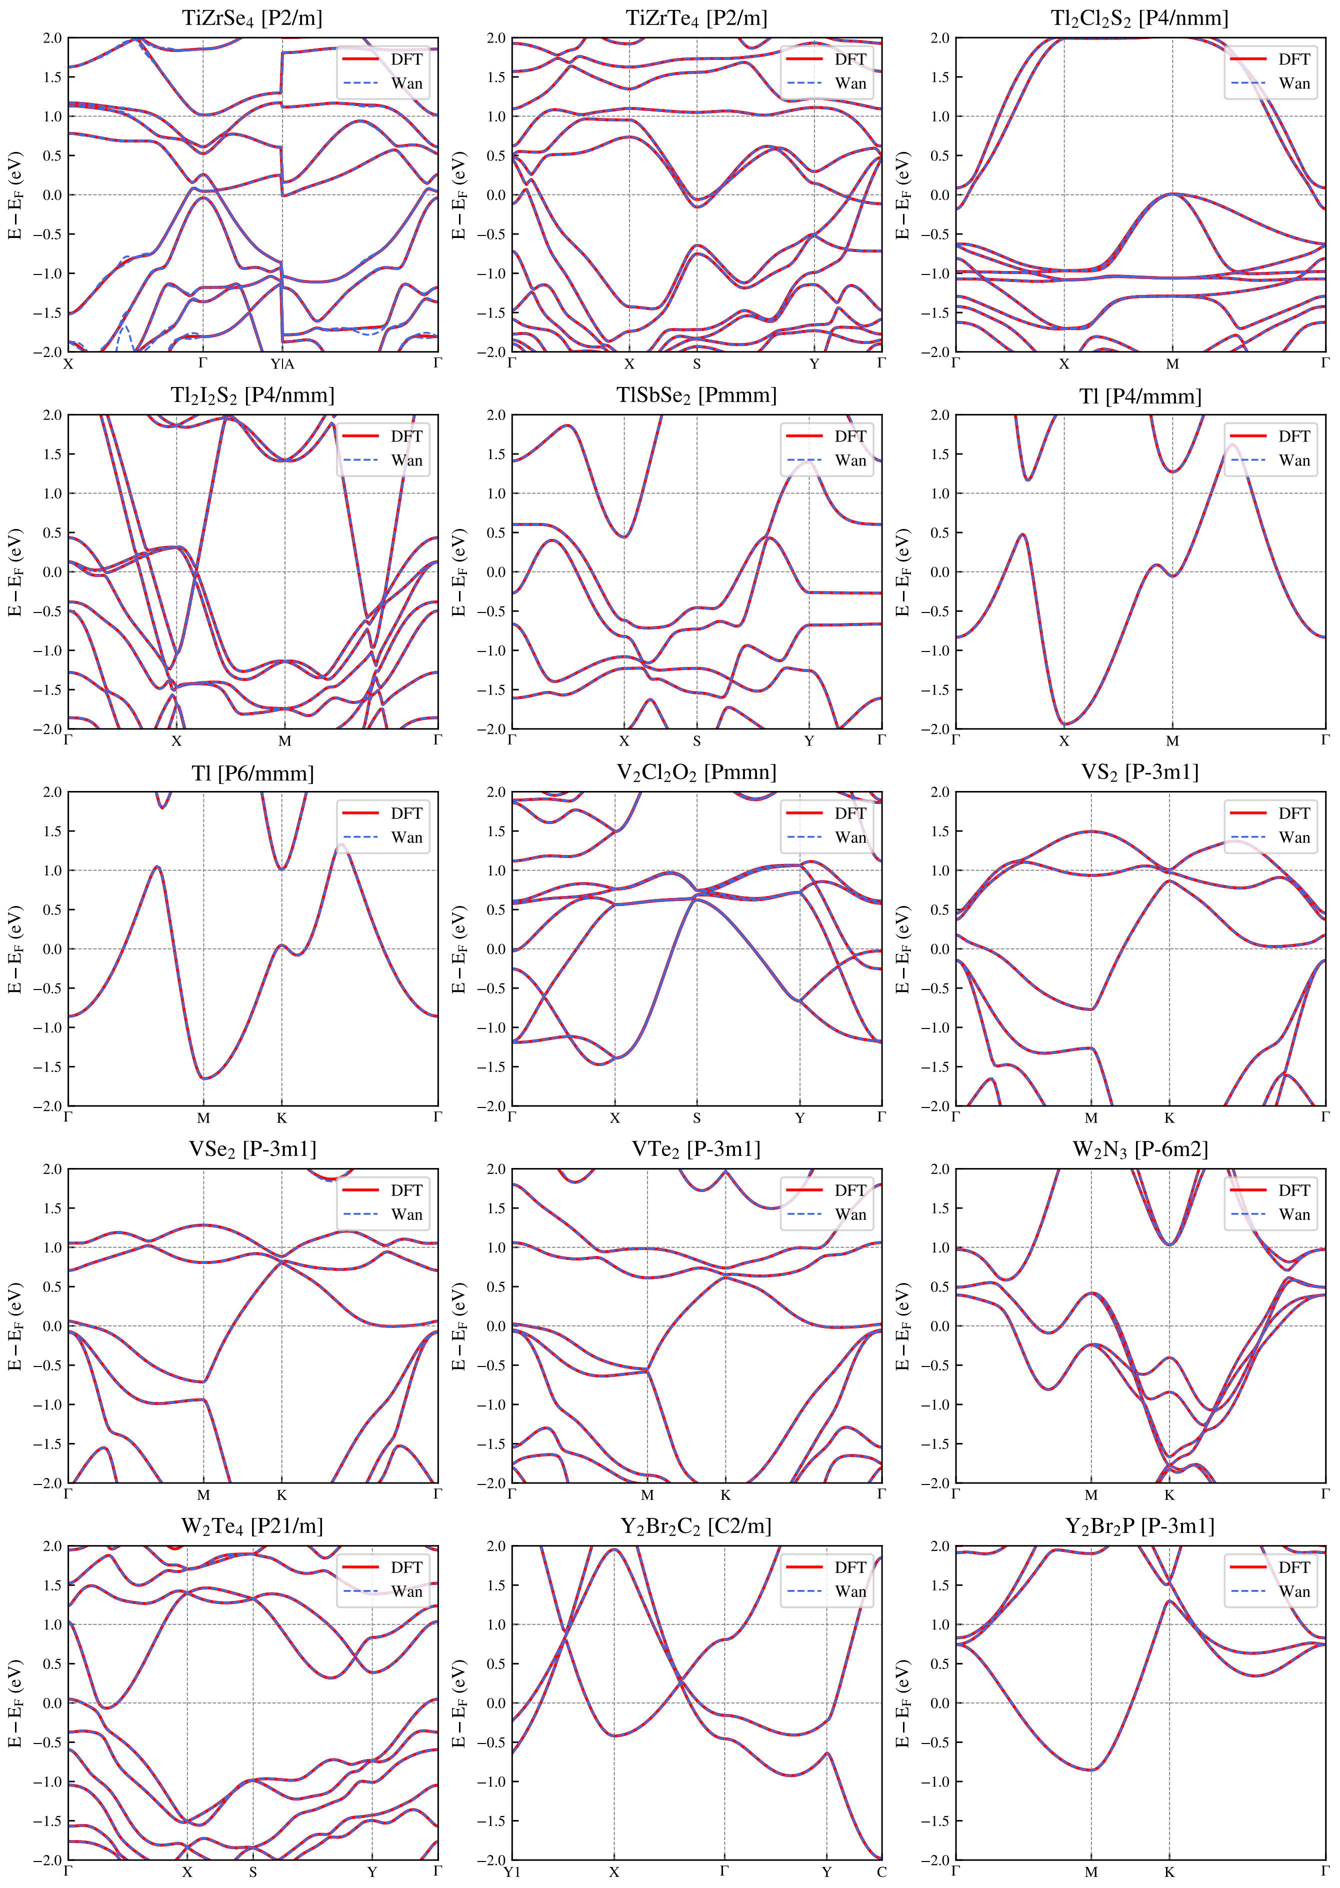
$TiZrSe_4$ [P2/m]
X Γ Y|A Γ
$TiZrTe_4$ [P2/m]
Γ X S Y Γ
$Tl_2Cl_2S_2$ [P4/nmm]
Γ X M Γ
$Tl_2I_2S_2$ [P4/nmm]
Γ X M Γ
$TlSbSe_2$ [Pmmm]
Γ X S Y Γ
Tl [P4/mmm]
Γ X M Γ
Tl [P6/mmm]
Γ M K Γ
$V_2Cl_2O_2$ [Pmmn]
Γ X S Y Γ
$VS_2$ [P-3m1]
Γ M K Γ
$VSe_2$ [P-3m1]
Γ M K Γ
$VTe_2$ [P-3m1]
Γ M K Γ
$W_2N_3$ [P-6m2]
Γ M K Γ
$W_2Te_4$ [P21/m]
Γ X S Y Γ
$Y_2Br_2C_2$ [C2/m]
Y1 X Γ Y C
$Y_2Br_2P$ [P-3m1]
Γ M K Γ
DFT
Wan
$E - E_F$ (eV)
2.0
1.5
1.0
0.5
0.0
−0.5
−1.0
−1.5
−2.0

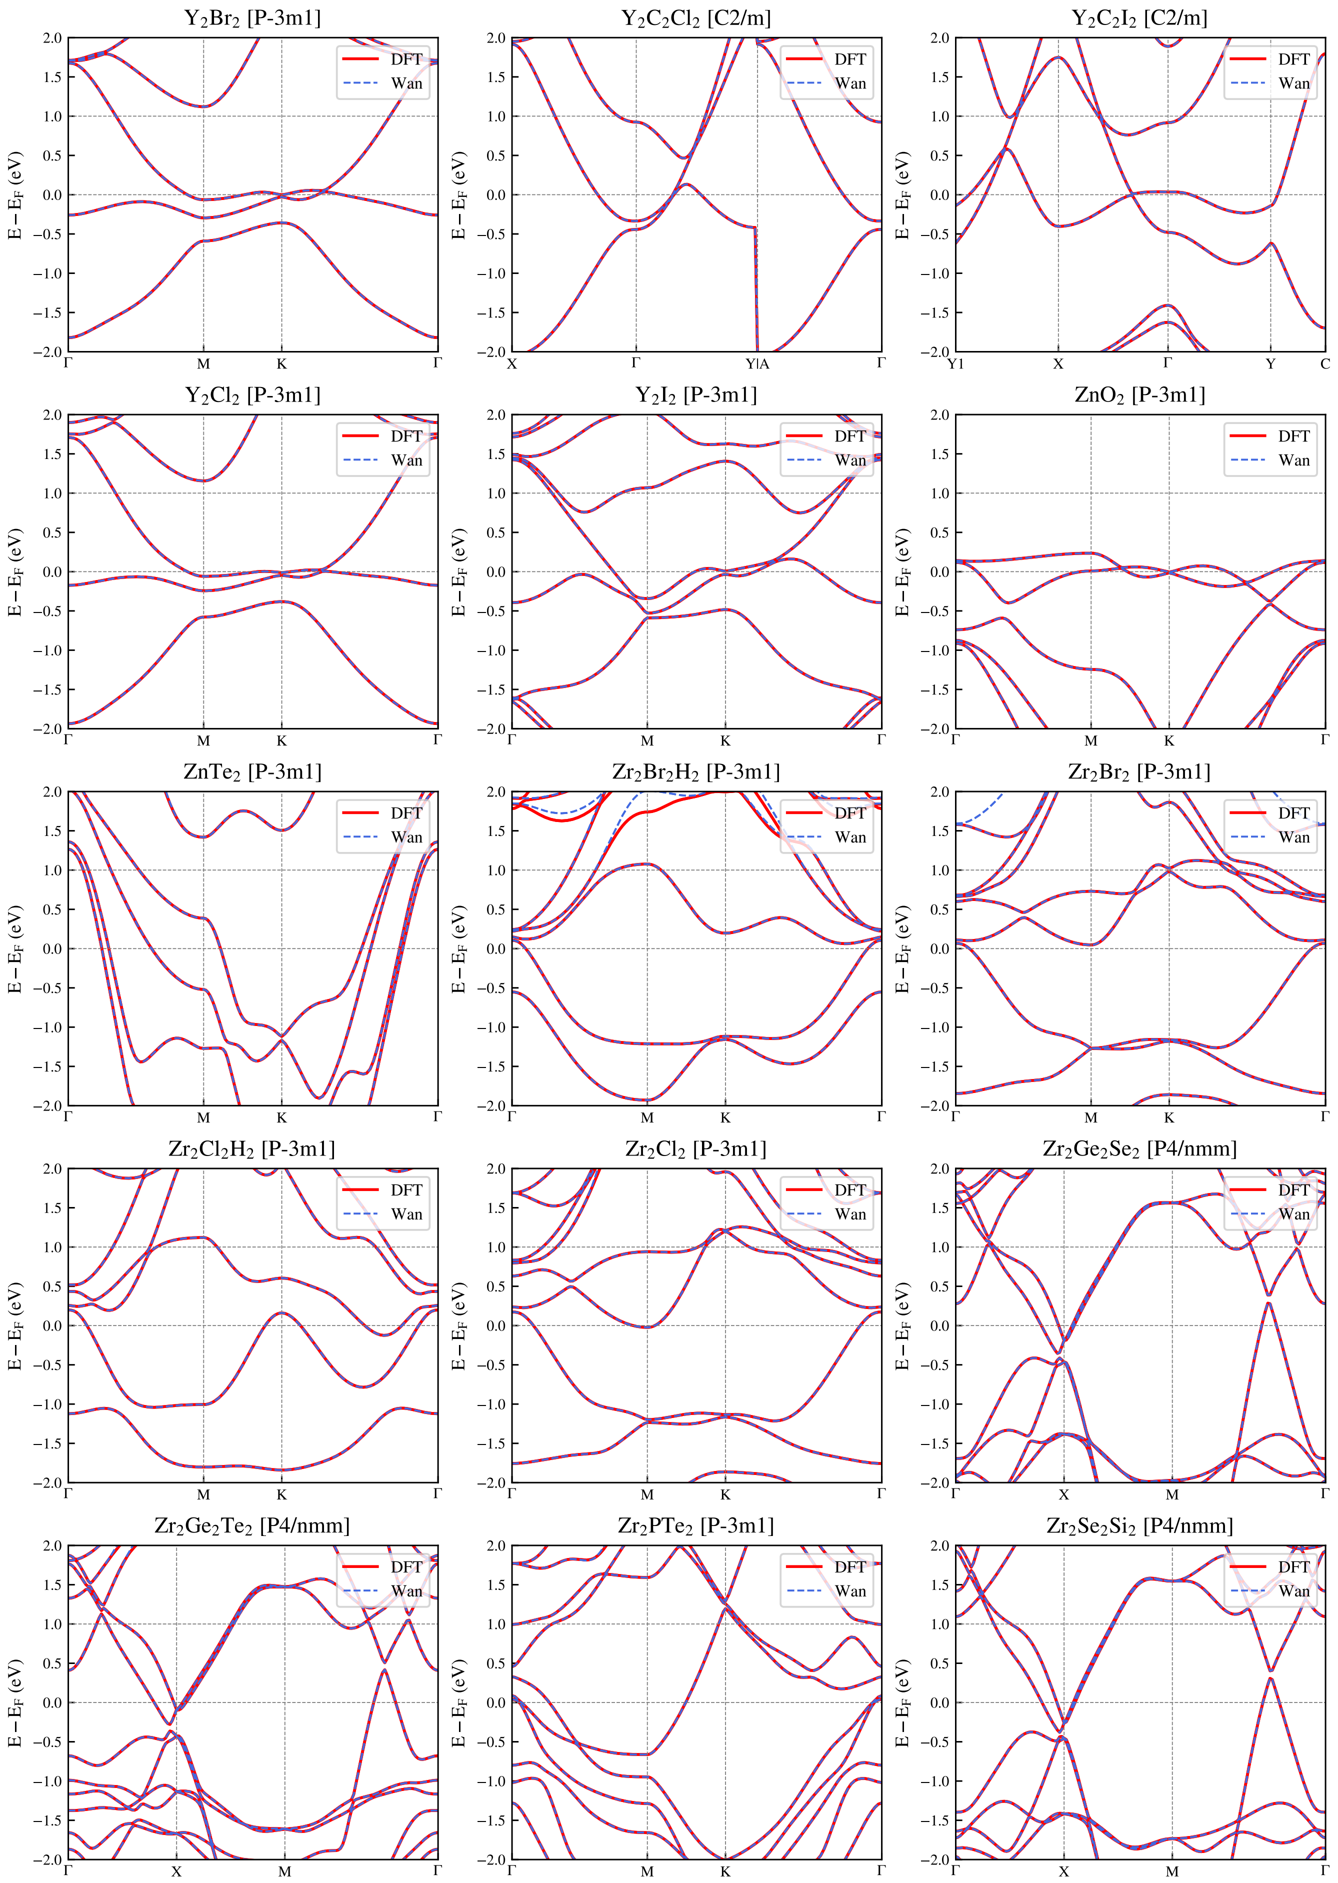

Y2Br2 [P-3m1]
Y2C2Cl2 [C2/m]
Y2C2I2 [C2/m]
Y2Cl2 [P-3m1]
Y2I2 [P-3m1]
ZnO2 [P-3m1]
ZnTe2 [P-3m1]
Zr2Br2H2 [P-3m1]
Zr2Br2 [P-3m1]
Zr2Cl2H2 [P-3m1]
Zr2Cl2 [P-3m1]
Zr2Ge2Se2 [P4/nmm]
Zr2Ge2Te2 [P4/nmm]
Zr2PTe2 [P-3m1]
Zr2Se2Si2 [P4/nmm]
DFT
Wan
E − E_F (eV)
Γ
M
K
X
Y|A
Y1
Y
C

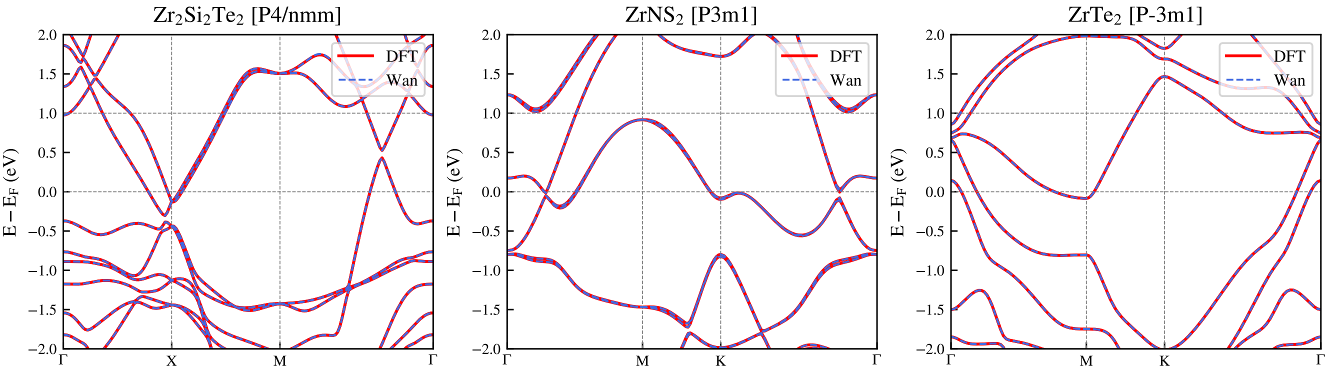
Zr2Si2Te2 [P4/nmm]
ZrNS2 [P3m1]
ZrTe2 [P-3m1]
DFT
Wan
E − EF (eV)
Γ
X
M
K

## Supplementary Sec. 5. Fully relativistic electronic structures of 216 monolayer insulators

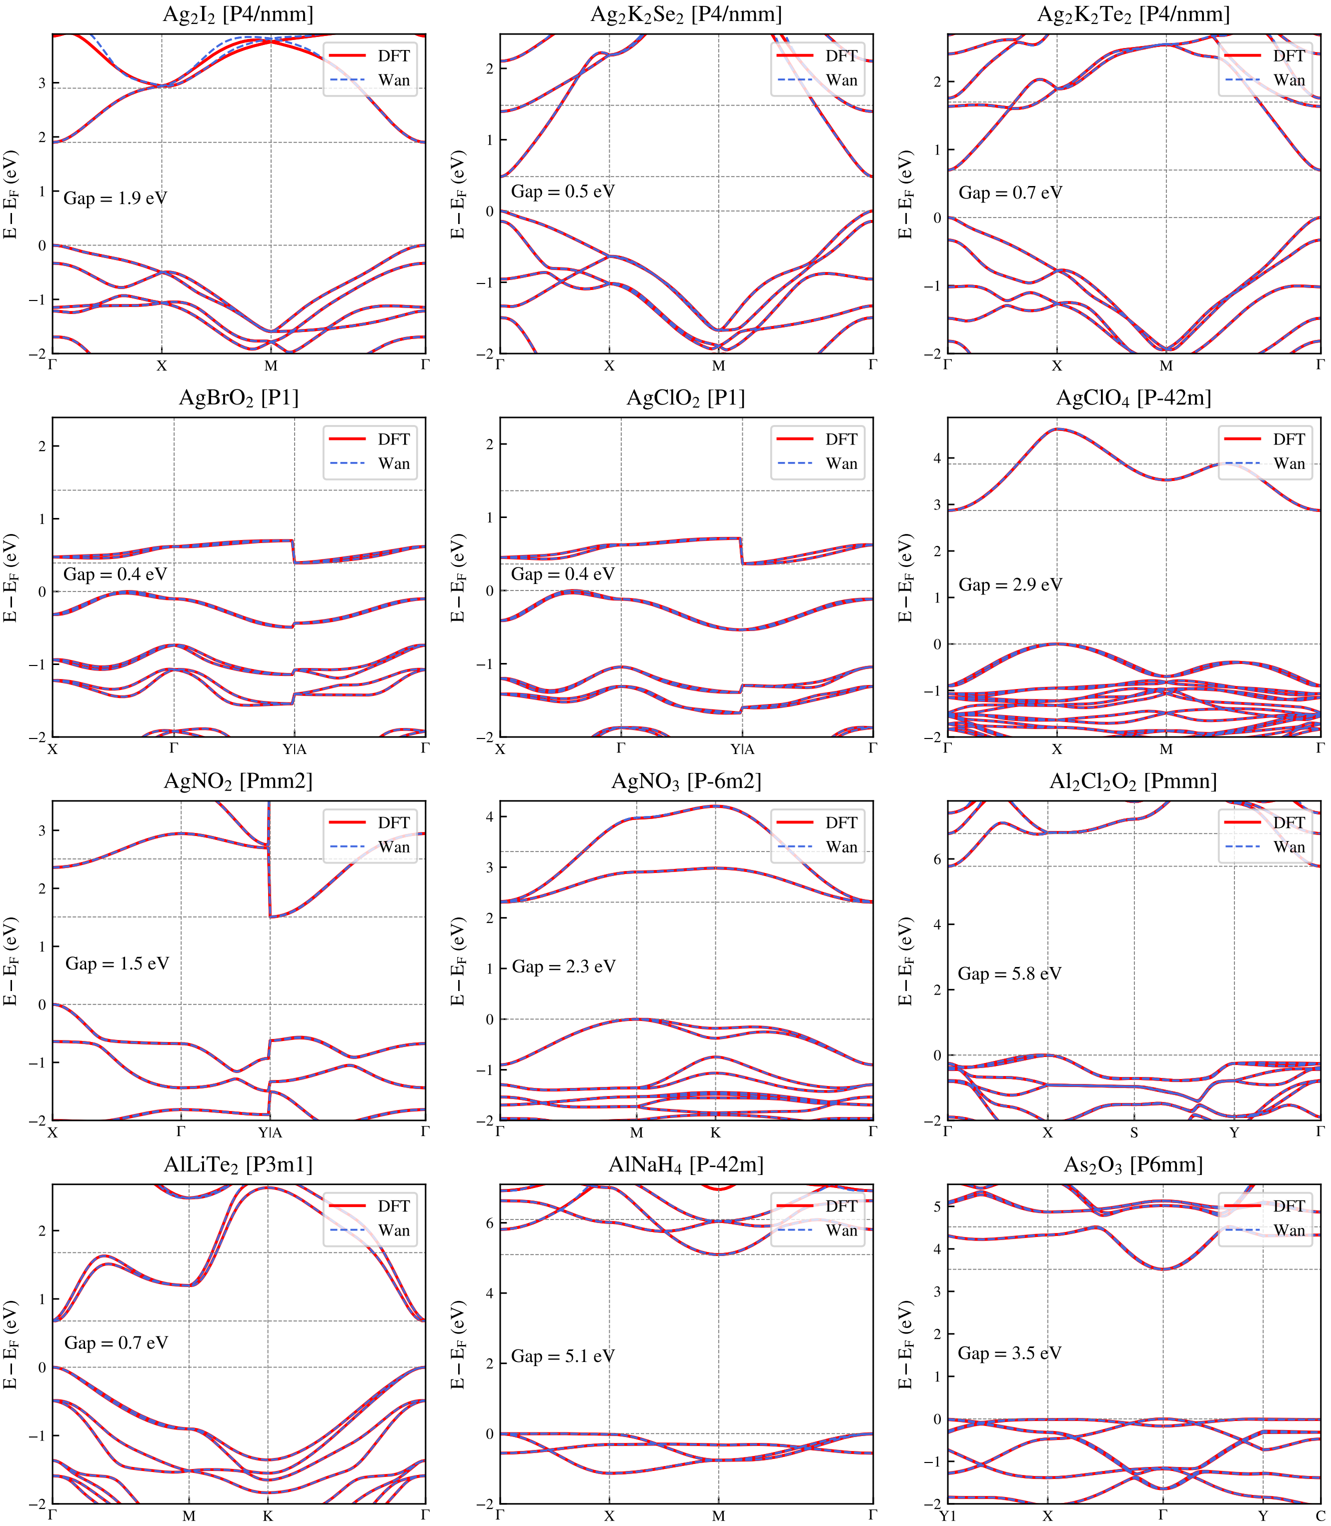

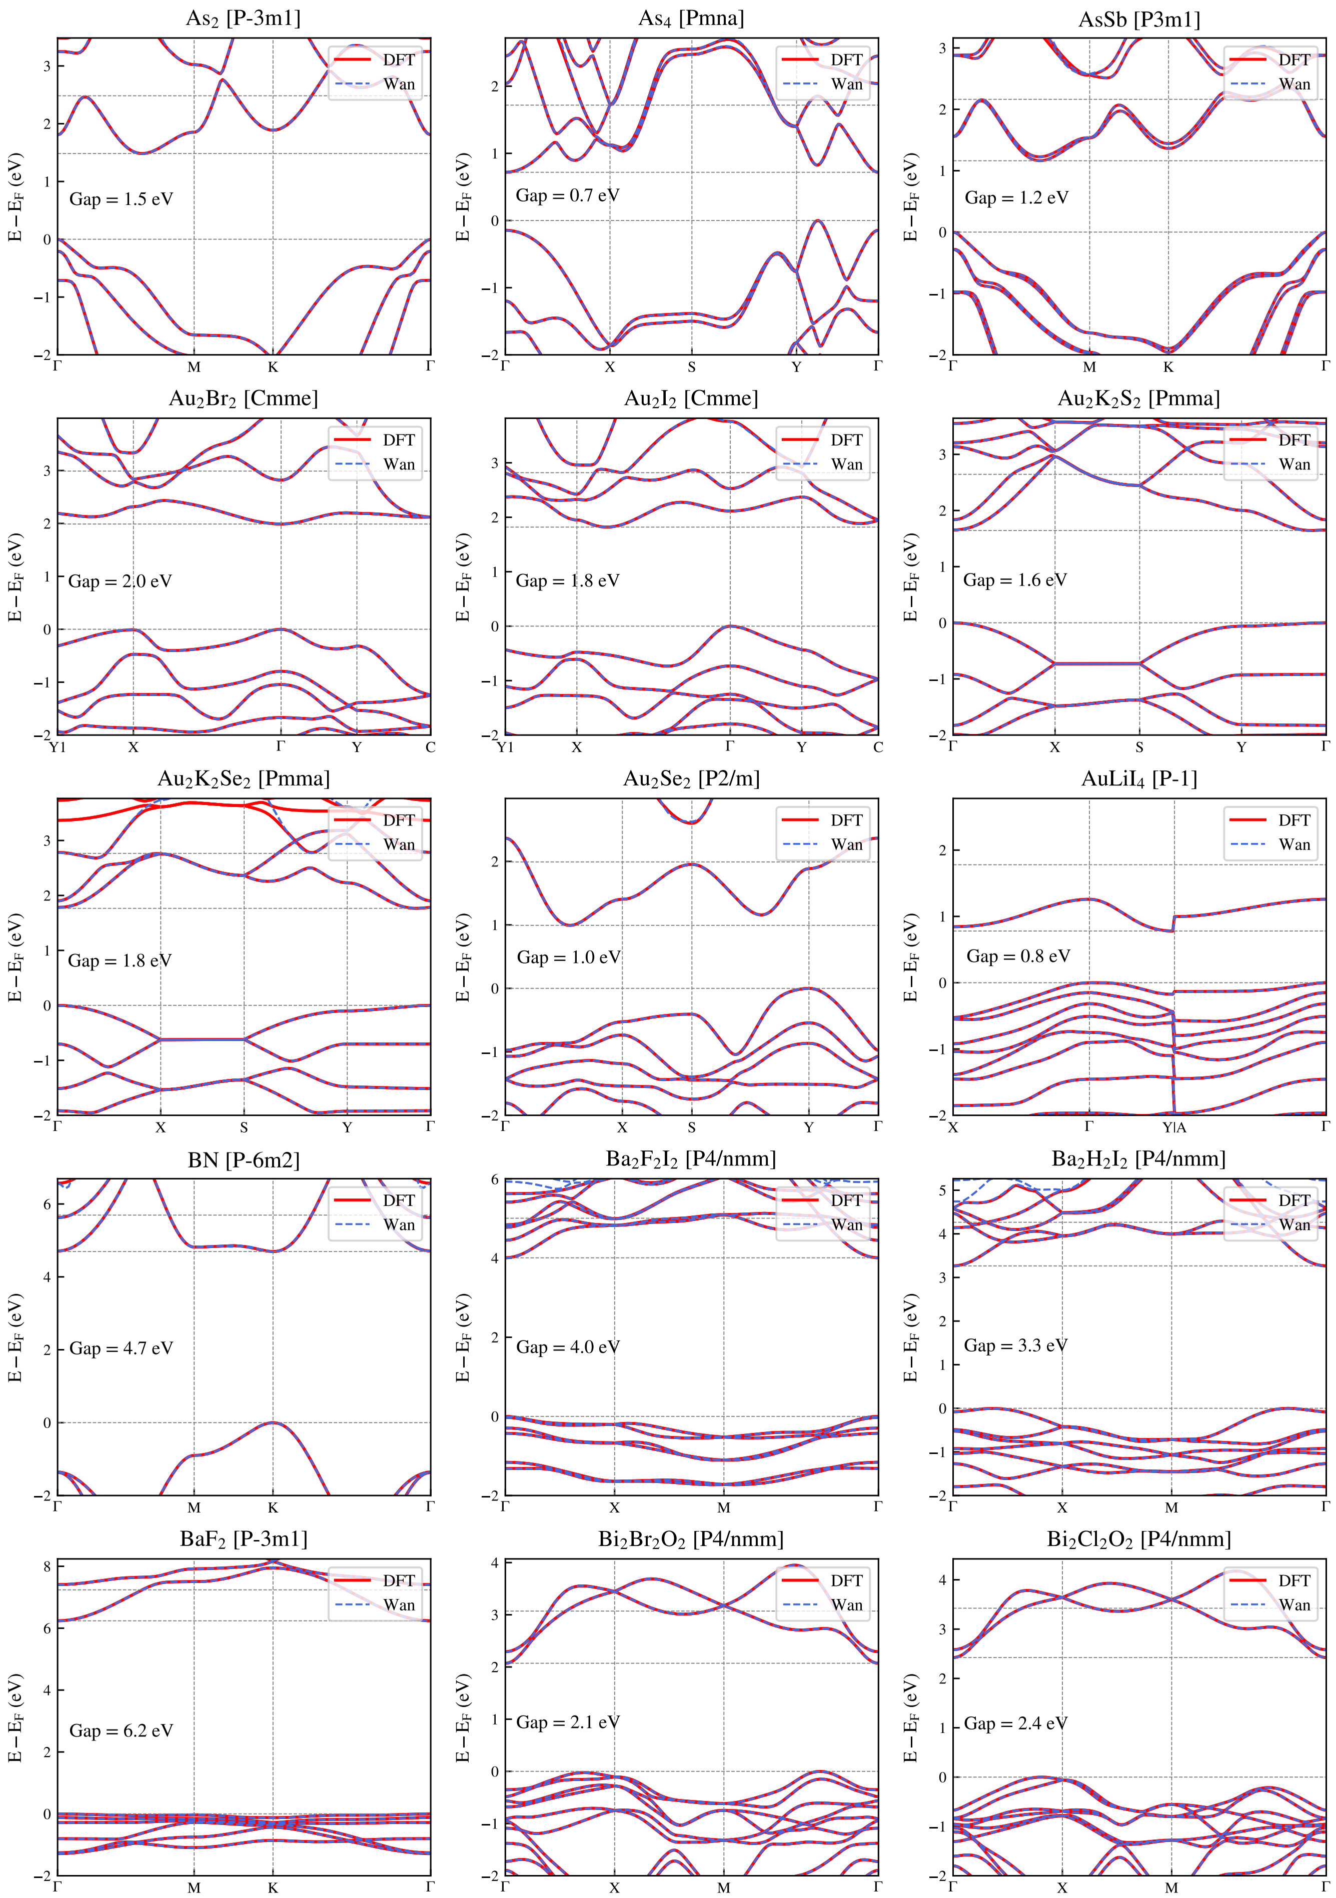
As2 [P-3m1]
Gap = 1.5 eV
As4 [Pmna]
Gap = 0.7 eV
AsSb [P3m1]
Gap = 1.2 eV
Au2Br2 [Cmme]
Gap = 2.0 eV
Au2I2 [Cmme]
Gap = 1.8 eV
Au2K2S2 [Pmma]
Gap = 1.6 eV
Au2K2Se2 [Pmma]
Gap = 1.8 eV
Au2Se2 [P2/m]
Gap = 1.0 eV
AuLiI4 [P-1]
Gap = 0.8 eV
BN [P-6m2]
Gap = 4.7 eV
Ba2F2I2 [P4/nmm]
Gap = 4.0 eV
Ba2H2I2 [P4/nmm]
Gap = 3.3 eV
BaF2 [P-3m1]
Gap = 6.2 eV
Bi2Br2O2 [P4/nmm]
Gap = 2.1 eV
Bi2Cl2O2 [P4/nmm]
Gap = 2.4 eV
DFT
Wan
E − EF (eV)

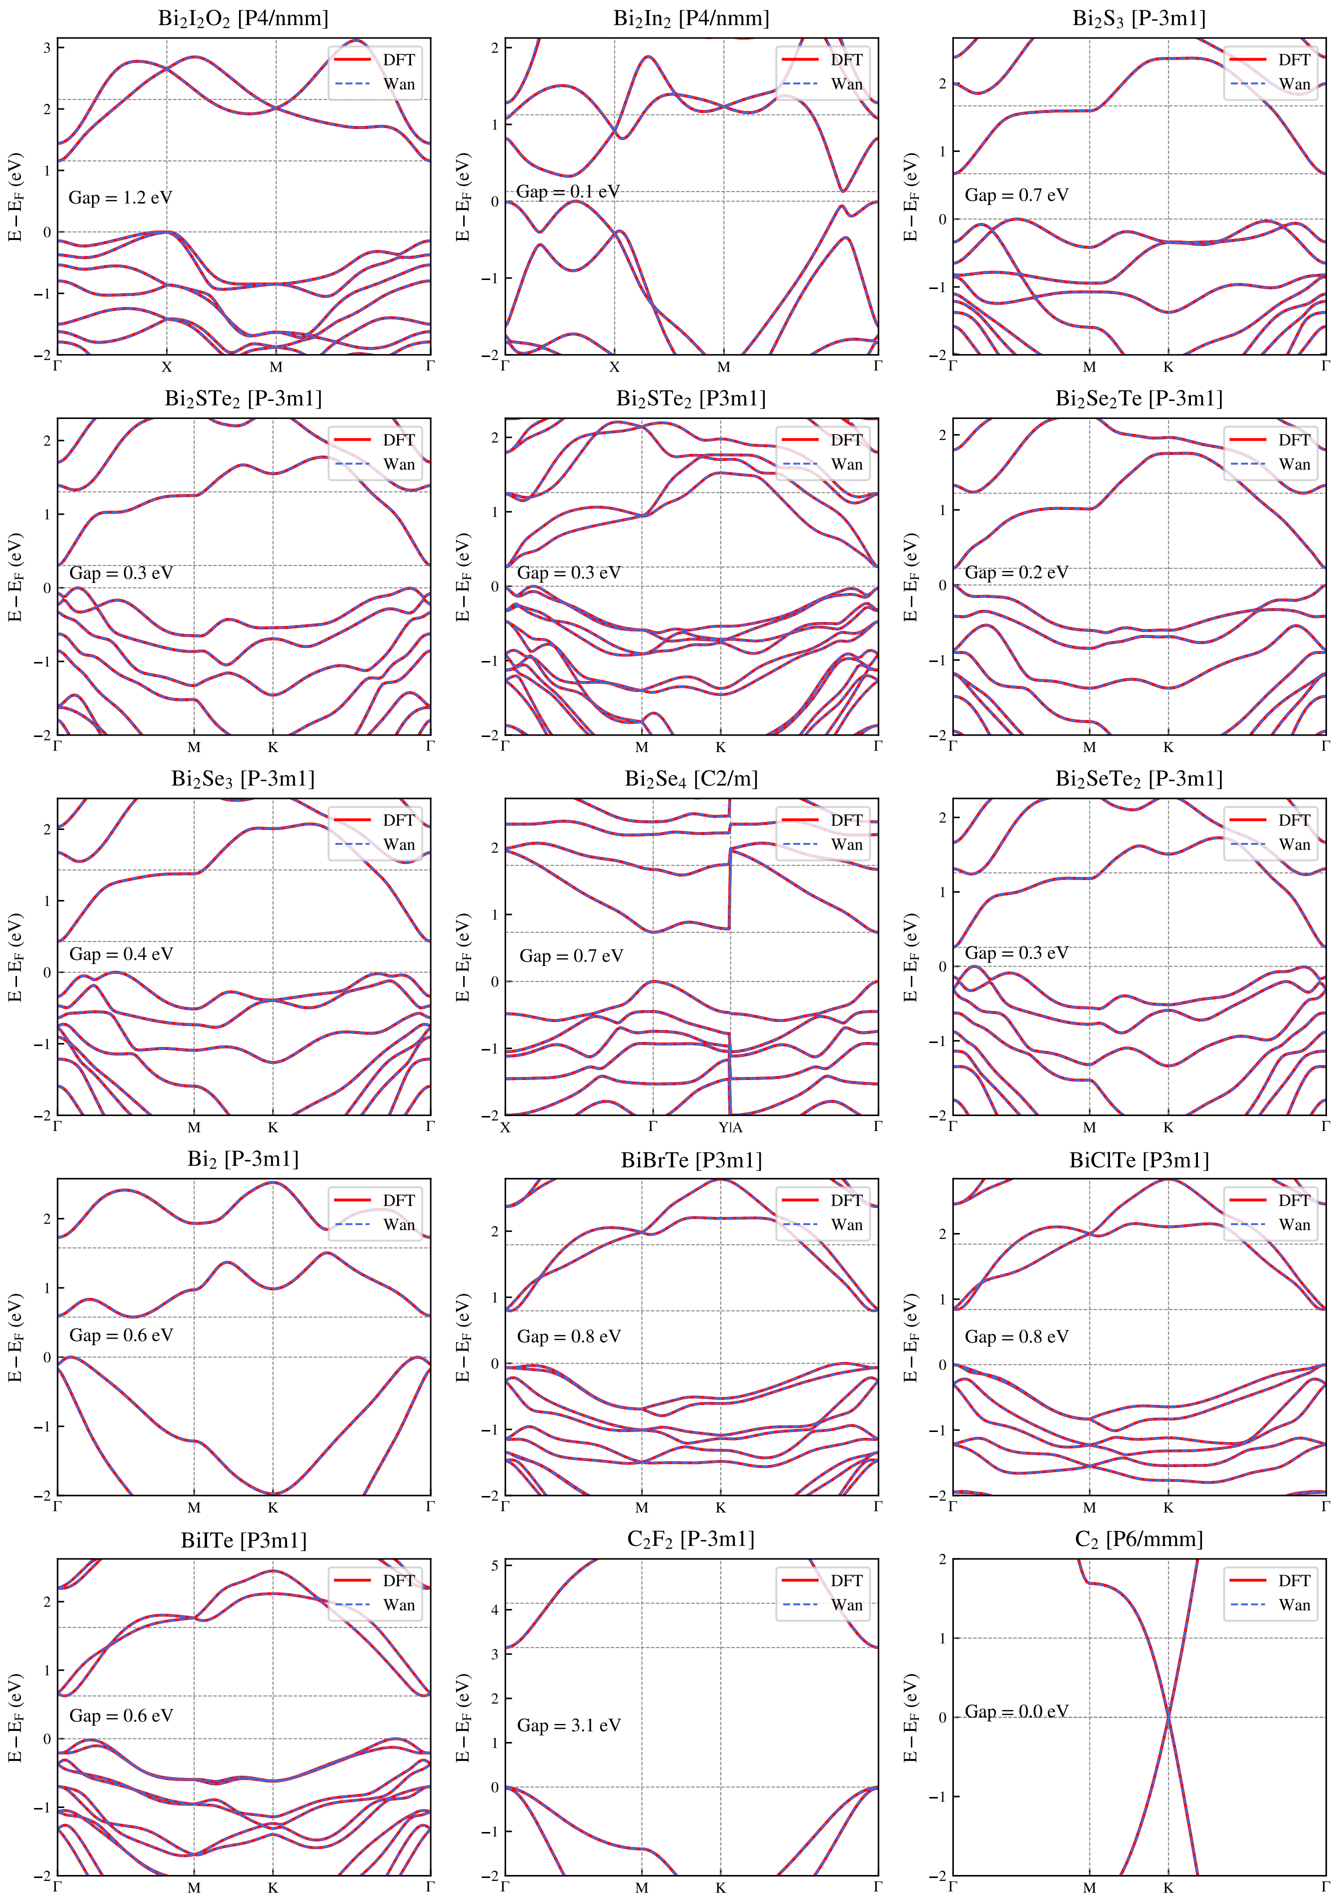

Bi$_2$I$_2$O$_2$ [P4/nmm]
Gap = 1.2 eV
Bi$_2$In$_2$ [P4/nmm]
Gap = 0.1 eV
Bi$_2$S$_3$ [P-3m1]
Gap = 0.7 eV
Bi$_2$STe$_2$ [P-3m1]
Gap = 0.3 eV
Bi$_2$STe$_2$ [P3m1]
Gap = 0.3 eV
Bi$_2$Se$_2$Te [P-3m1]
Gap = 0.2 eV
Bi$_2$Se$_3$ [P-3m1]
Gap = 0.4 eV
Bi$_2$Se$_4$ [C2/m]
Gap = 0.7 eV
Bi$_2$SeTe$_2$ [P-3m1]
Gap = 0.3 eV
Bi$_2$ [P-3m1]
Gap = 0.6 eV
BiBrTe [P3m1]
Gap = 0.8 eV
BiClTe [P3m1]
Gap = 0.8 eV
BiITe [P3m1]
Gap = 0.6 eV
C$_2$F$_2$ [P-3m1]
Gap = 3.1 eV
C$_2$ [P6/mmm]
Gap = 0.0 eV
DFT
Wan
E − E$_F$ (eV)
Γ X M Γ
Γ M K Γ
X Γ Y|A Γ

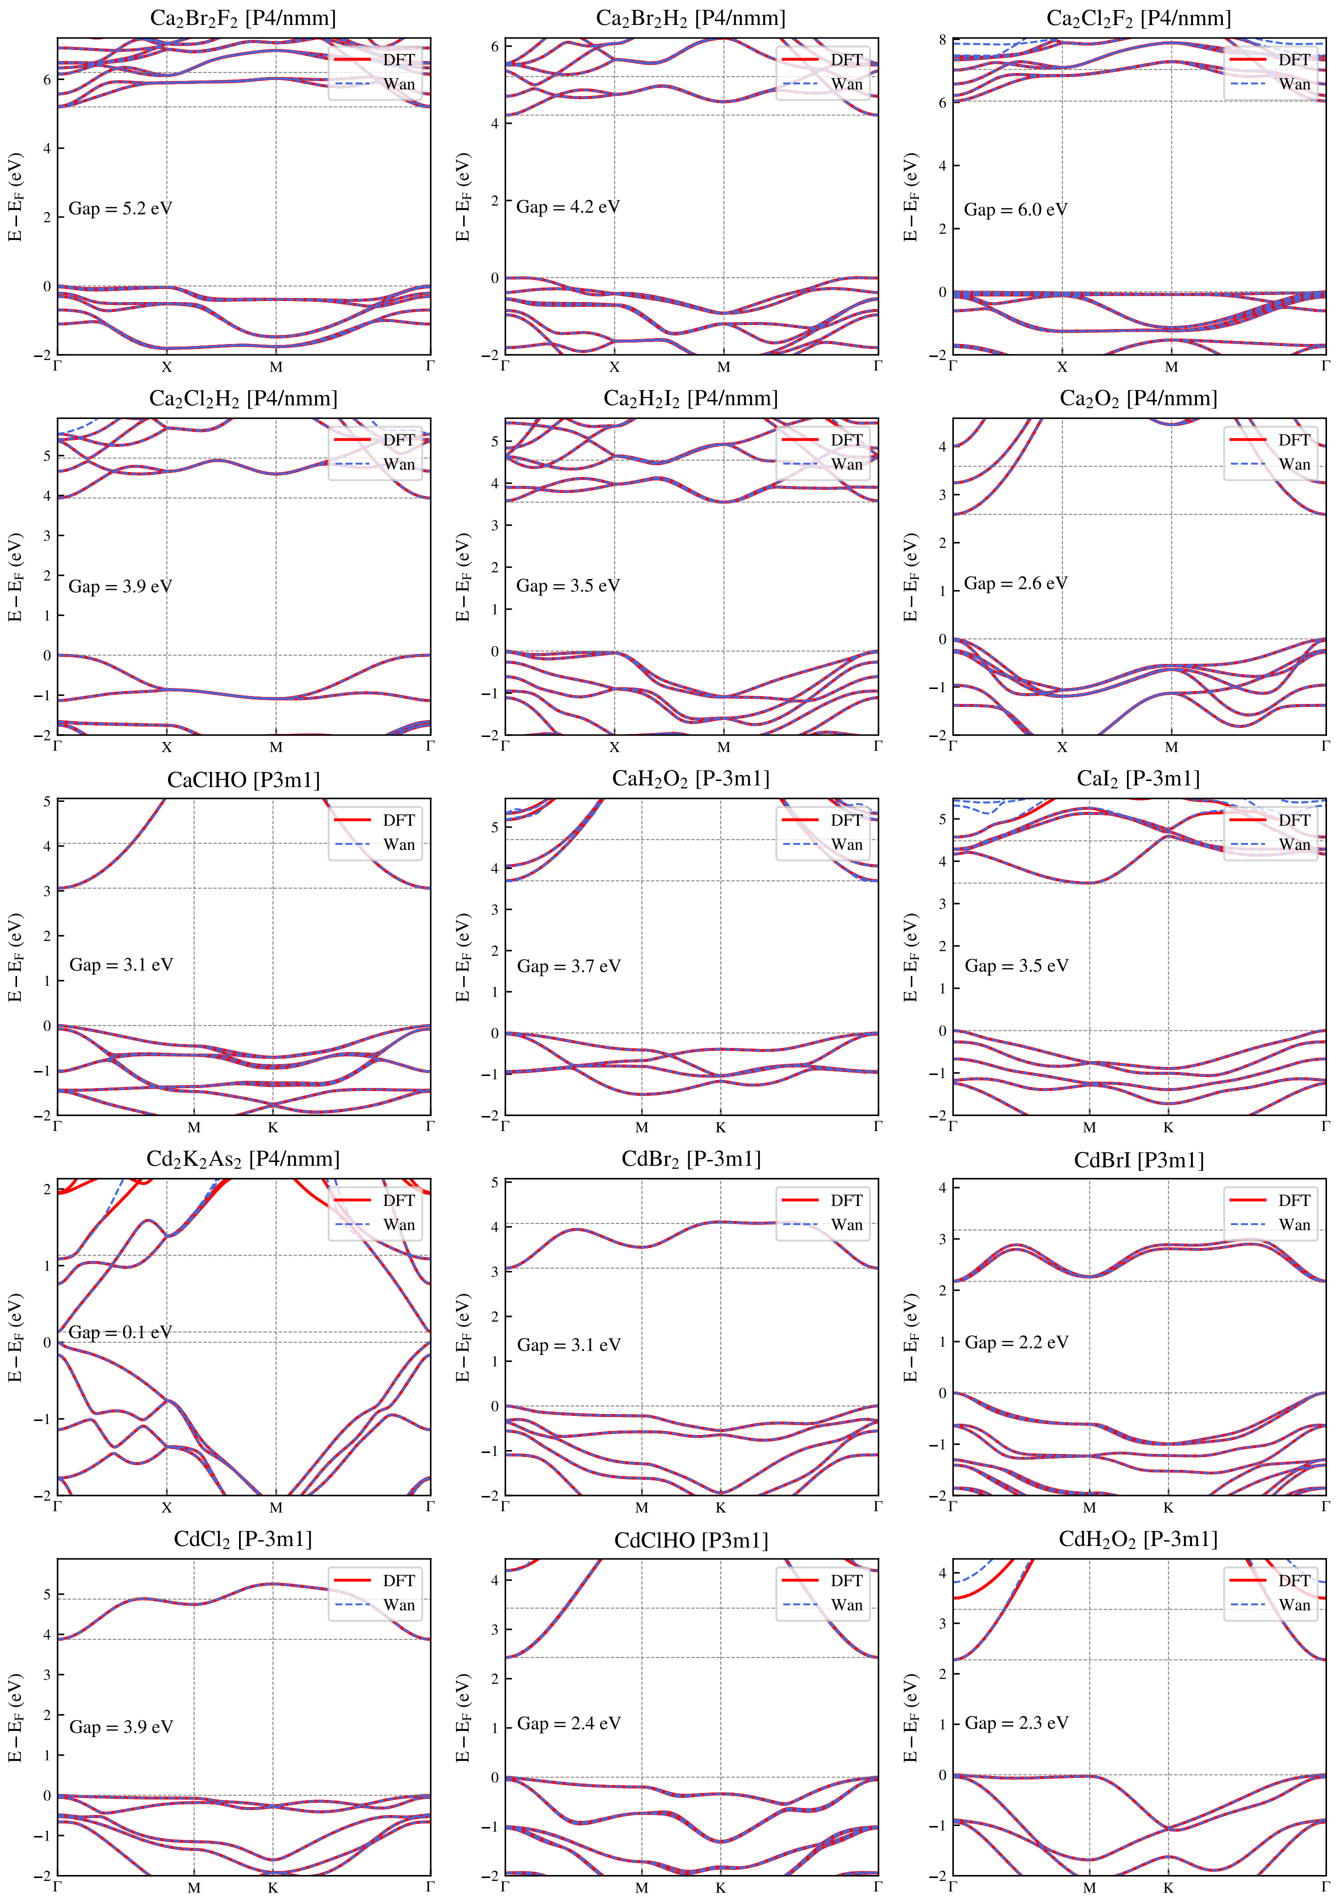
Ca2Br2F2 [P4/nmm]
Gap = 5.2 eV
Ca2Br2H2 [P4/nmm]
Gap = 4.2 eV
Ca2Cl2F2 [P4/nmm]
Gap = 6.0 eV
Ca2Cl2H2 [P4/nmm]
Gap = 3.9 eV
Ca2H2I2 [P4/nmm]
Gap = 3.5 eV
Ca2O2 [P4/nmm]
Gap = 2.6 eV
CaClHO [P3m1]
Gap = 3.1 eV
CaH2O2 [P-3m1]
Gap = 3.7 eV
CaI2 [P-3m1]
Gap = 3.5 eV
Cd2K2As2 [P4/nmm]
Gap = 0.1 eV
CdBr2 [P-3m1]
Gap = 3.1 eV
CdBrI [P3m1]
Gap = 2.2 eV
CdCl2 [P-3m1]
Gap = 3.9 eV
CdClHO [P3m1]
Gap = 2.4 eV
CdH2O2 [P-3m1]
Gap = 2.3 eV
DFT
Wan
E − EF (eV)
Γ
X
M
K

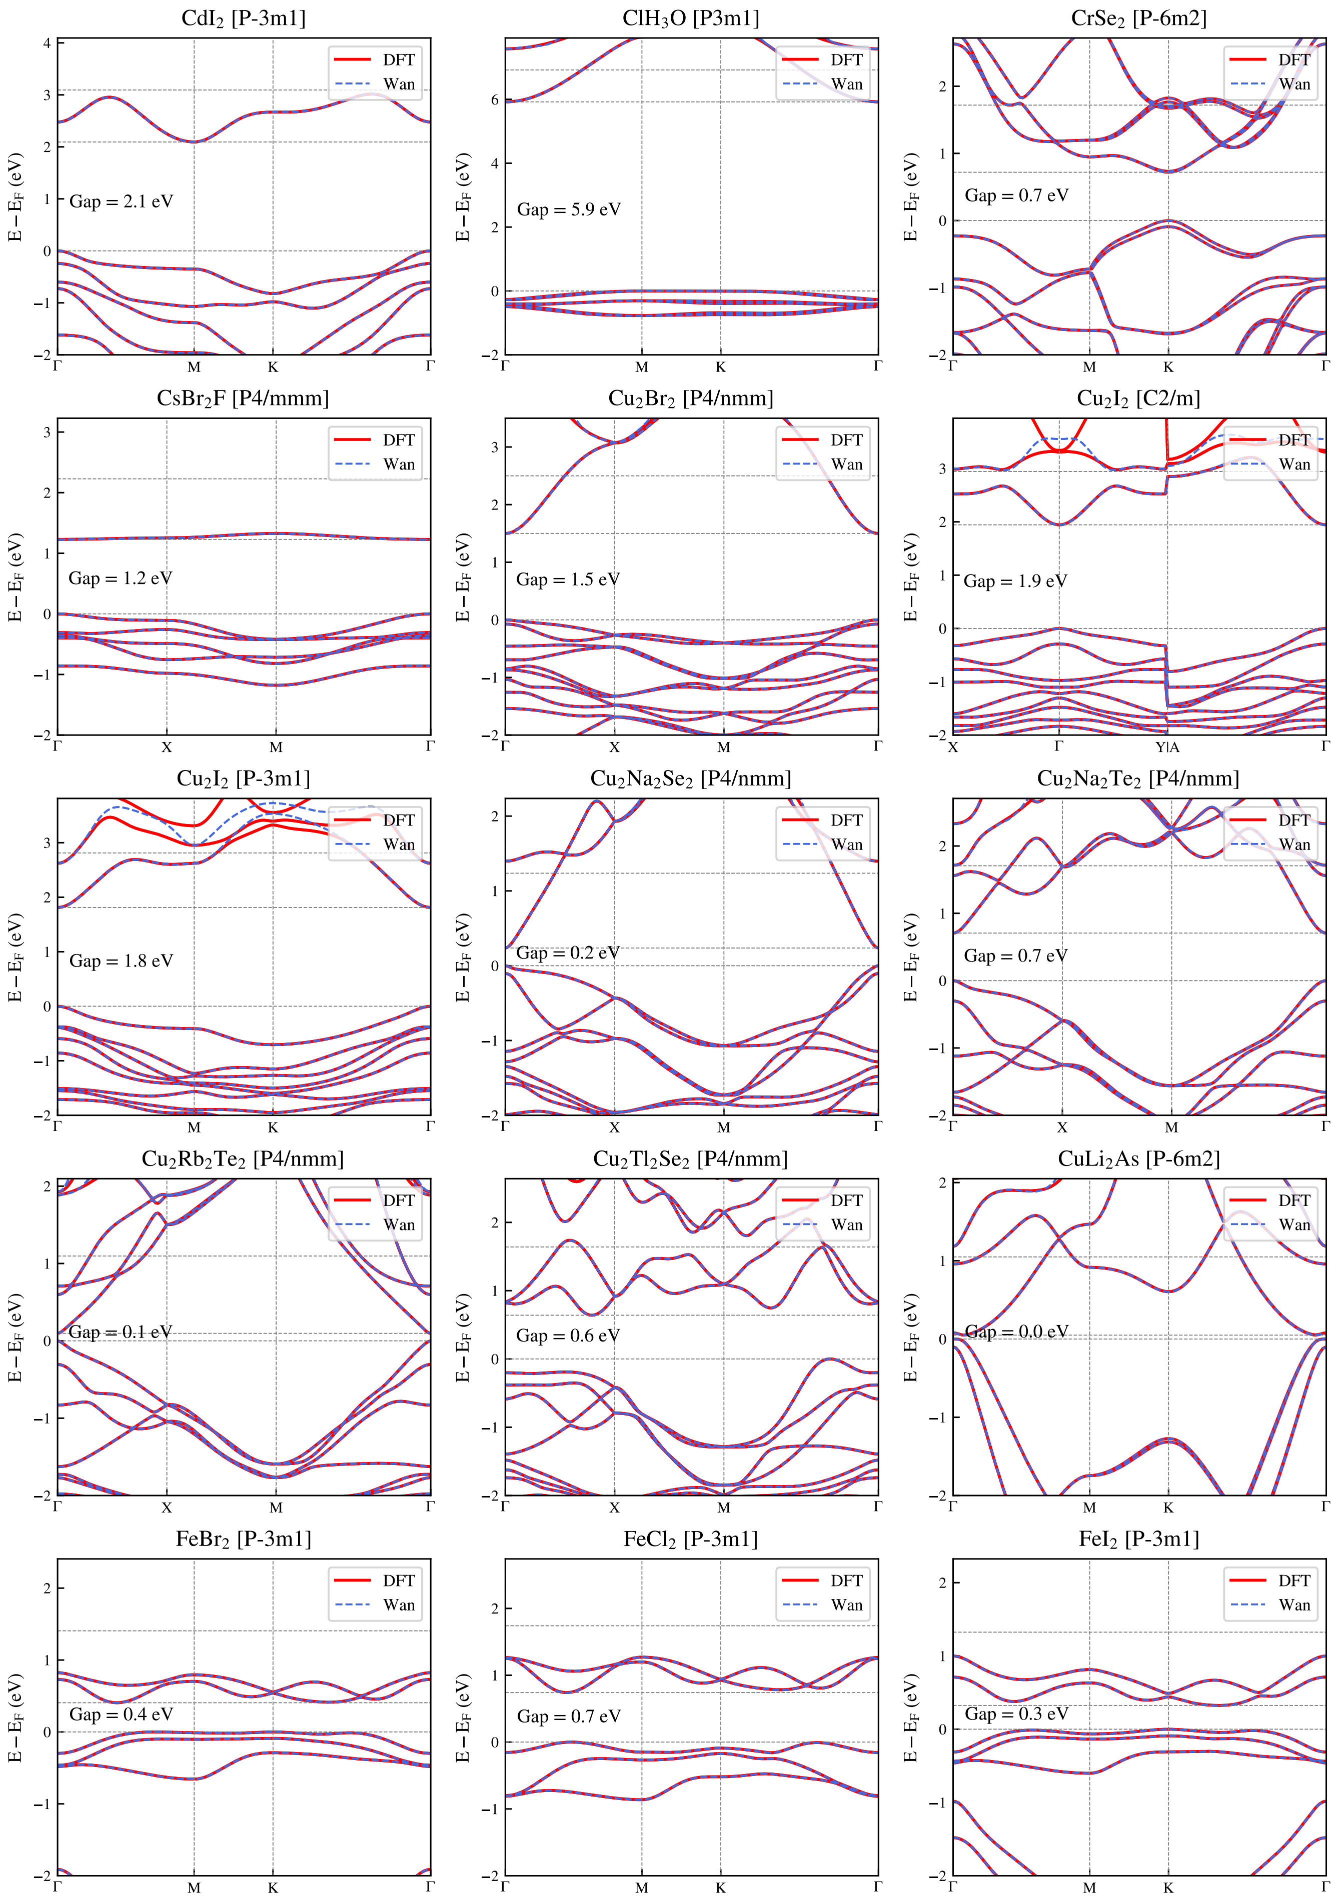
CdI2 [P-3m1]
Gap = 2.1 eV
ClH3O [P3m1]
Gap = 5.9 eV
CrSe2 [P-6m2]
Gap = 0.7 eV
CsBr2F [P4/mmm]
Gap = 1.2 eV
Cu2Br2 [P4/nmm]
Gap = 1.5 eV
Cu2I2 [C2/m]
Gap = 1.9 eV
Cu2I2 [P-3m1]
Gap = 1.8 eV
Cu2Na2Se2 [P4/nmm]
Gap = 0.2 eV
Cu2Na2Te2 [P4/nmm]
Gap = 0.7 eV
Cu2Rb2Te2 [P4/nmm]
Gap = 0.1 eV
Cu2Tl2Se2 [P4/nmm]
Gap = 0.6 eV
CuLi2As [P-6m2]
Gap = 0.0 eV
FeBr2 [P-3m1]
Gap = 0.4 eV
FeCl2 [P-3m1]
Gap = 0.7 eV
FeI2 [P-3m1]
Gap = 0.3 eV
DFT
Wan
E − EF (eV)
Γ
M
K
X
Y|A

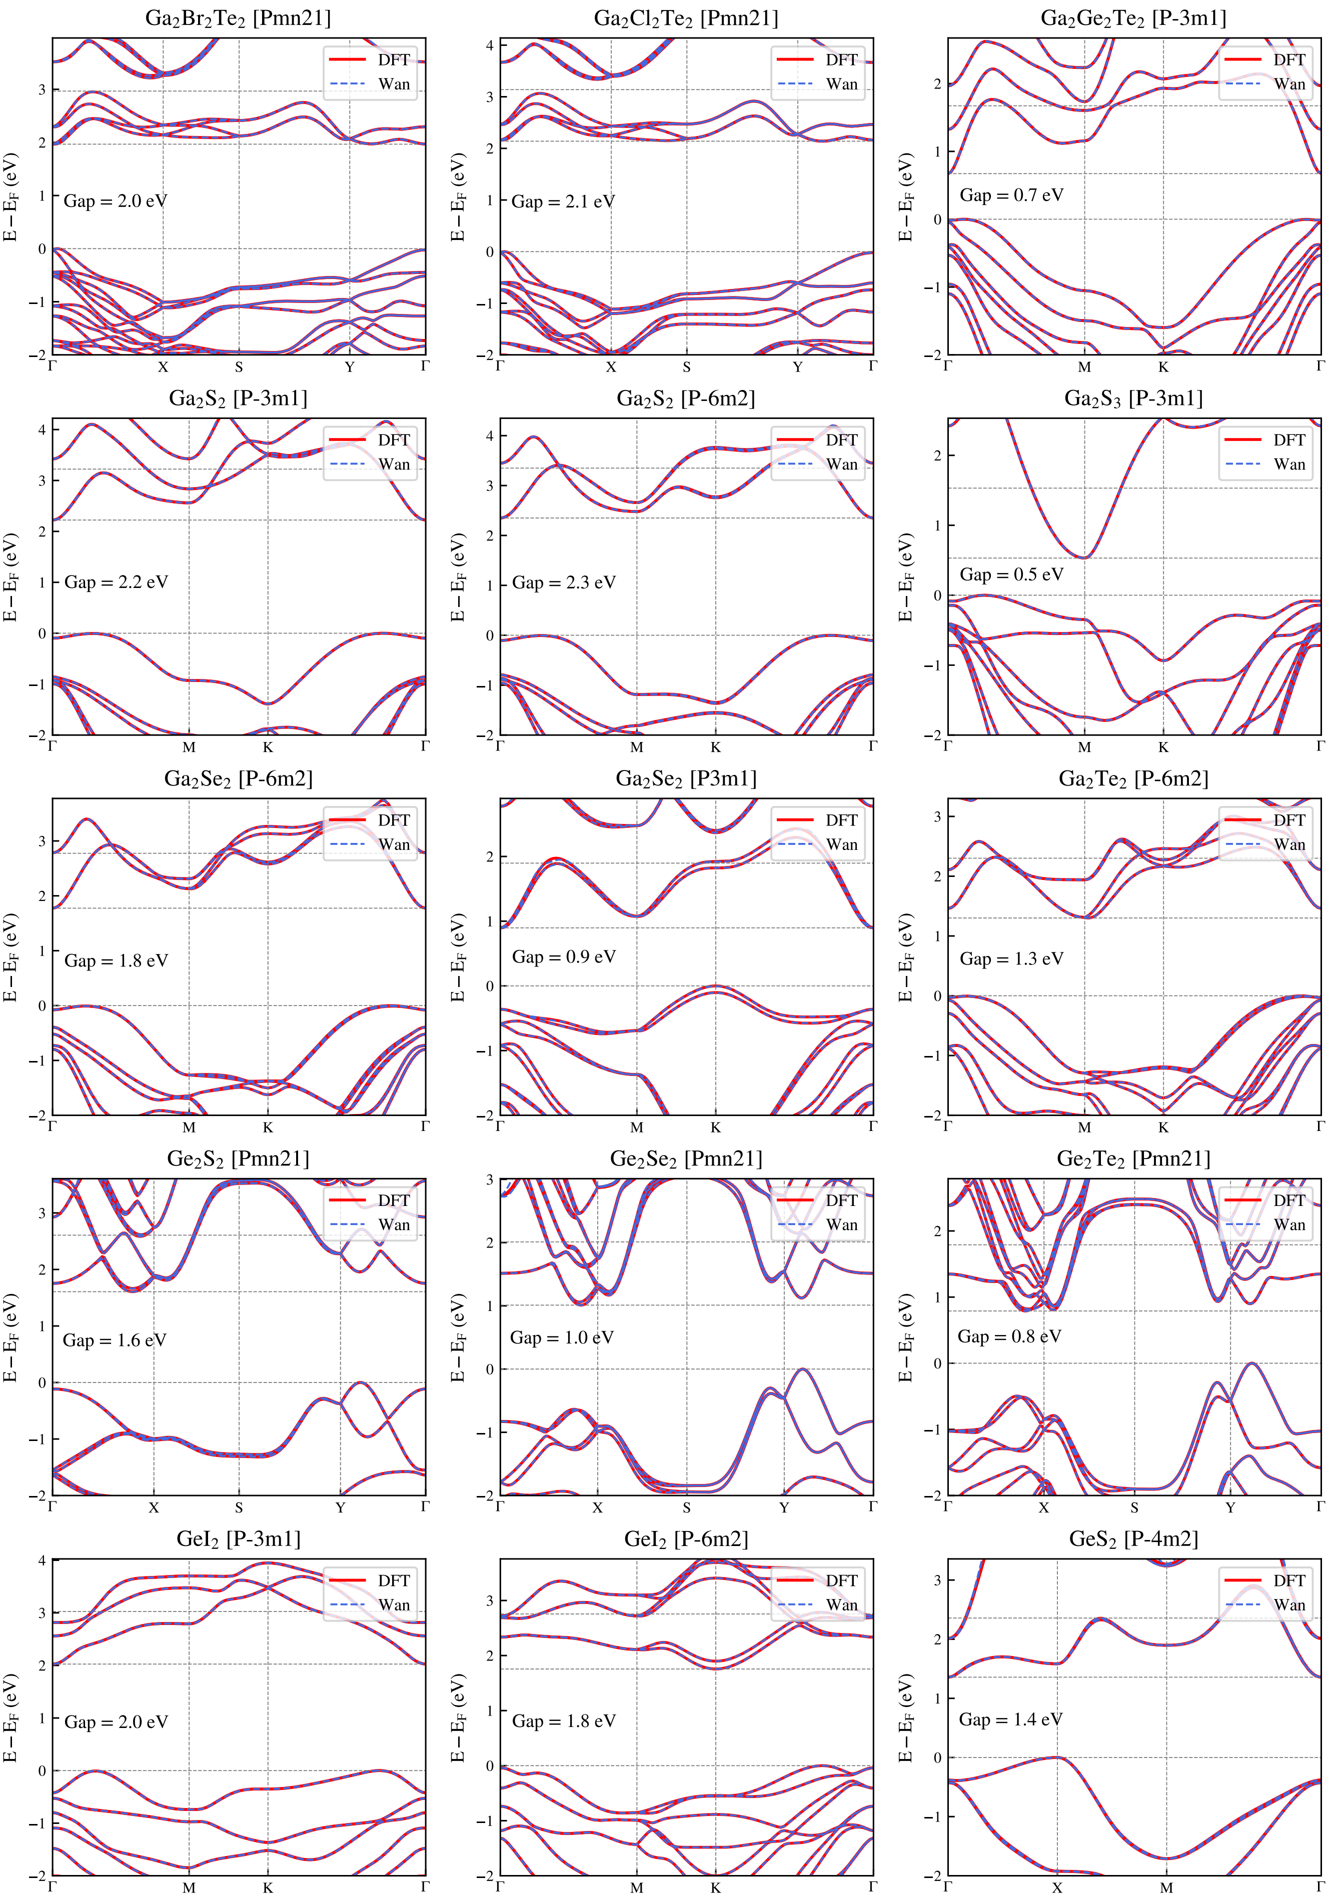
$Ga_2Br_2Te_2$ [Pmn21]
Gap = 2.0 eV
$Ga_2Cl_2Te_2$ [Pmn21]
Gap = 2.1 eV
$Ga_2Ge_2Te_2$ [P-3m1]
Gap = 0.7 eV
$Ga_2S_2$ [P-3m1]
Gap = 2.2 eV
$Ga_2S_2$ [P-6m2]
Gap = 2.3 eV
$Ga_2S_3$ [P-3m1]
Gap = 0.5 eV
$Ga_2Se_2$ [P-6m2]
Gap = 1.8 eV
$Ga_2Se_2$ [P3m1]
Gap = 0.9 eV
$Ga_2Te_2$ [P-6m2]
Gap = 1.3 eV
$Ge_2S_2$ [Pmn21]
Gap = 1.6 eV
$Ge_2Se_2$ [Pmn21]
Gap = 1.0 eV
$Ge_2Te_2$ [Pmn21]
Gap = 0.8 eV
$GeI_2$ [P-3m1]
Gap = 2.0 eV
$GeI_2$ [P-6m2]
Gap = 1.8 eV
$GeS_2$ [P-4m2]
Gap = 1.4 eV
DFT
Wan
$E - E_F$ (eV)
Γ X S Y Γ
Γ M K Γ
Γ X M Γ

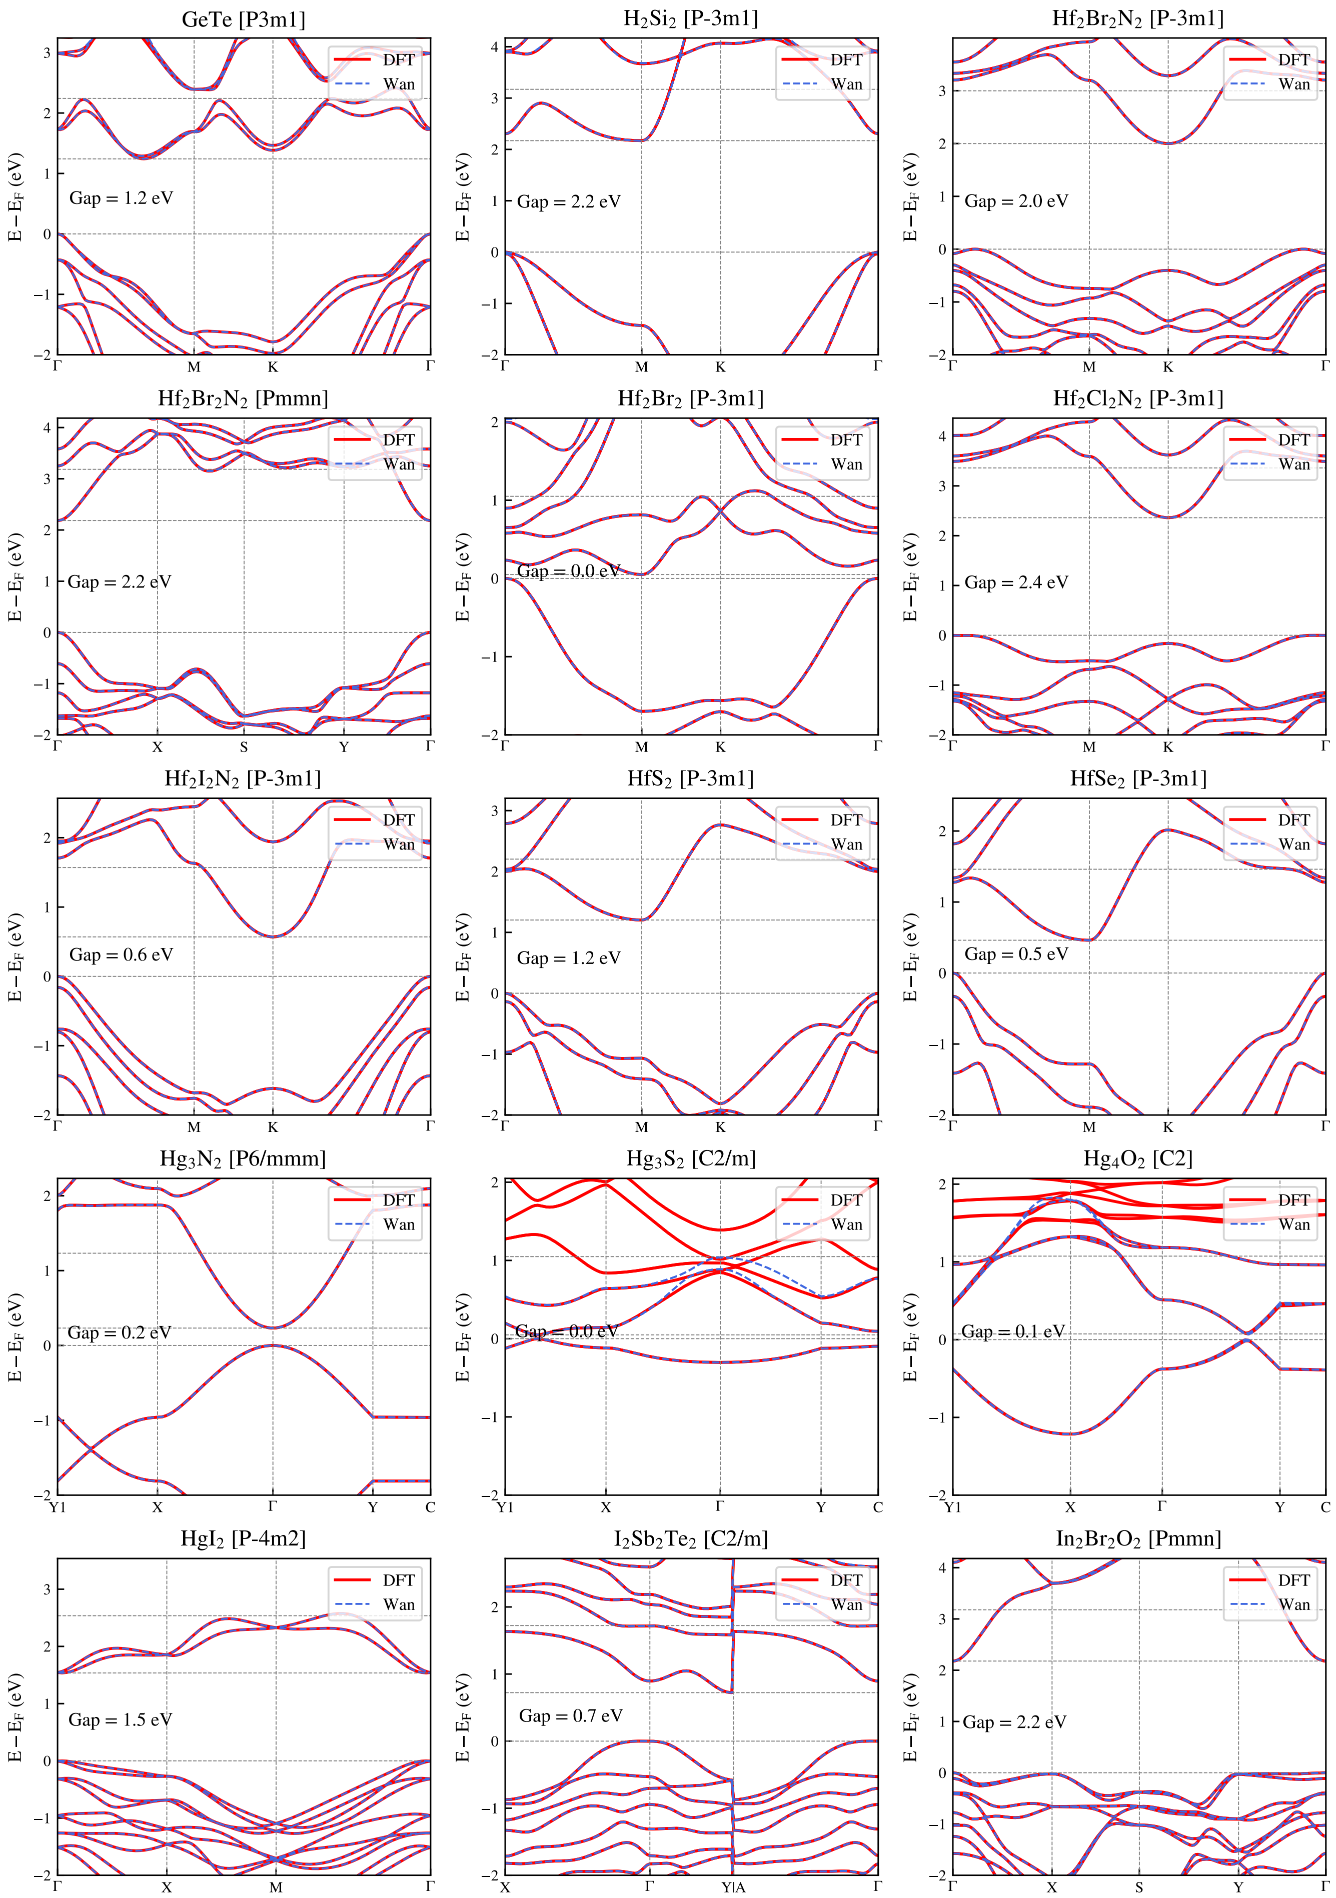
GeTe [P3m1]
Gap = 1.2 eV
H2Si2 [P-3m1]
Gap = 2.2 eV
Hf2Br2N2 [P-3m1]
Gap = 2.0 eV
Hf2Br2N2 [Pmmn]
Gap = 2.2 eV
Hf2Br2 [P-3m1]
Gap = 0.0 eV
Hf2Cl2N2 [P-3m1]
Gap = 2.4 eV
Hf2I2N2 [P-3m1]
Gap = 0.6 eV
HfS2 [P-3m1]
Gap = 1.2 eV
HfSe2 [P-3m1]
Gap = 0.5 eV
Hg3N2 [P6/mmm]
Gap = 0.2 eV
Hg3S2 [C2/m]
Gap = 0.0 eV
Hg4O2 [C2]
Gap = 0.1 eV
HgI2 [P-4m2]
Gap = 1.5 eV
I2Sb2Te2 [C2/m]
Gap = 0.7 eV
In2Br2O2 [Pmmn]
Gap = 2.2 eV
DFT
Wan
E − EF (eV)
Γ
M
K
X
S
Y
Y1
C
Y|A

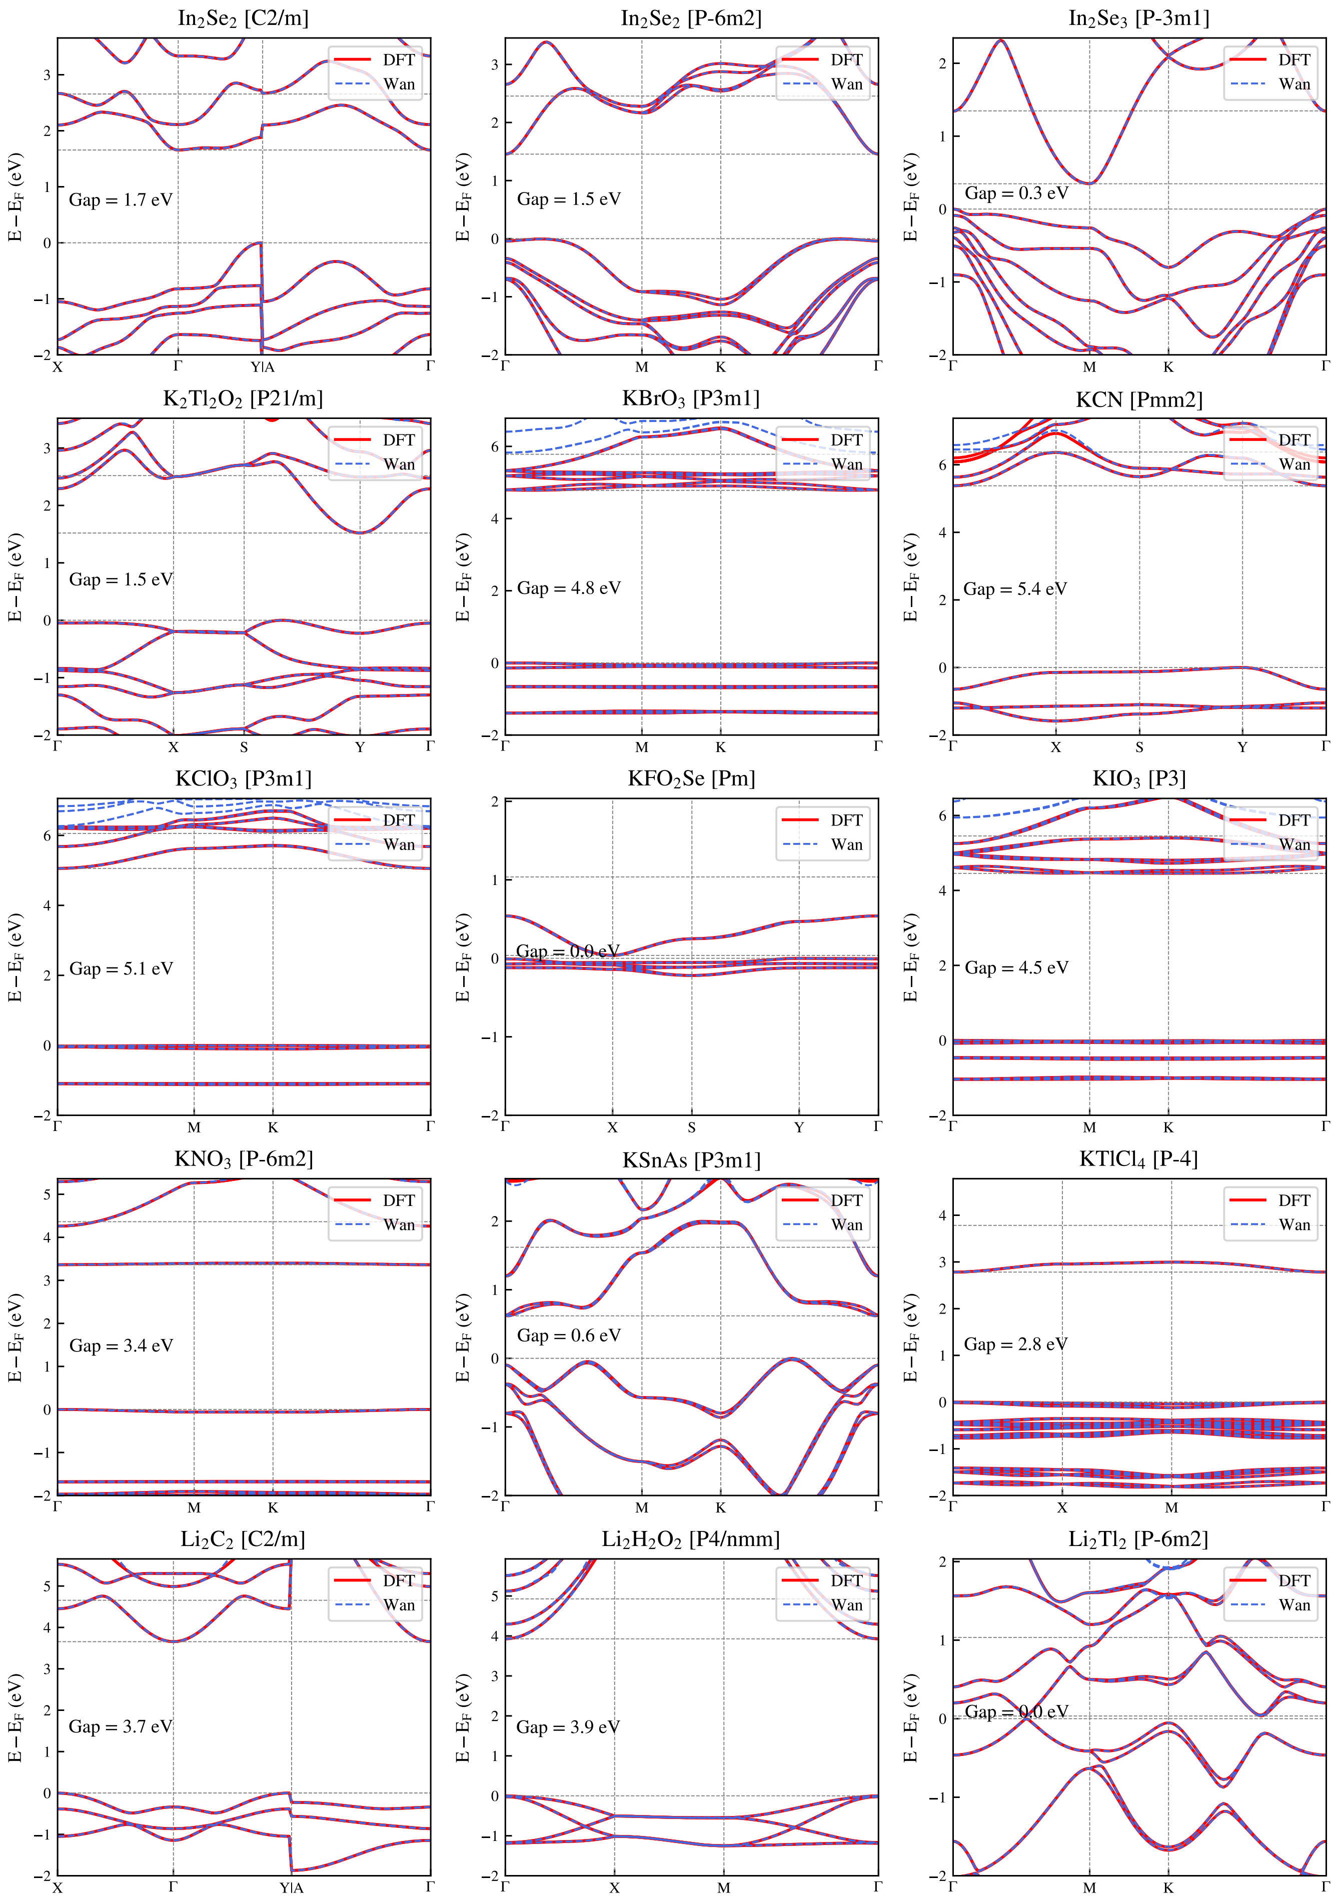

$In_2Se_2$ [C2/m]
Gap = 1.7 eV
$In_2Se_2$ [P-6m2]
Gap = 1.5 eV
$In_2Se_3$ [P-3m1]
Gap = 0.3 eV
$K_2Tl_2O_2$ [P21/m]
Gap = 1.5 eV
$KBrO_3$ [P3m1]
Gap = 4.8 eV
KCN [Pmm2]
Gap = 5.4 eV
$KClO_3$ [P3m1]
Gap = 5.1 eV
$KFO_2Se$ [Pm]
Gap = 0.0 eV
$KIO_3$ [P3]
Gap = 4.5 eV
$KNO_3$ [P-6m2]
Gap = 3.4 eV
KSnAs [P3m1]
Gap = 0.6 eV
$KTlCl_4$ [P-4]
Gap = 2.8 eV
$Li_2C_2$ [C2/m]
Gap = 3.7 eV
$Li_2H_2O_2$ [P4/nmm]
Gap = 3.9 eV
$Li_2Tl_2$ [P-6m2]
Gap = 0.0 eV
DFT
Wan
$E - E_F$ (eV)

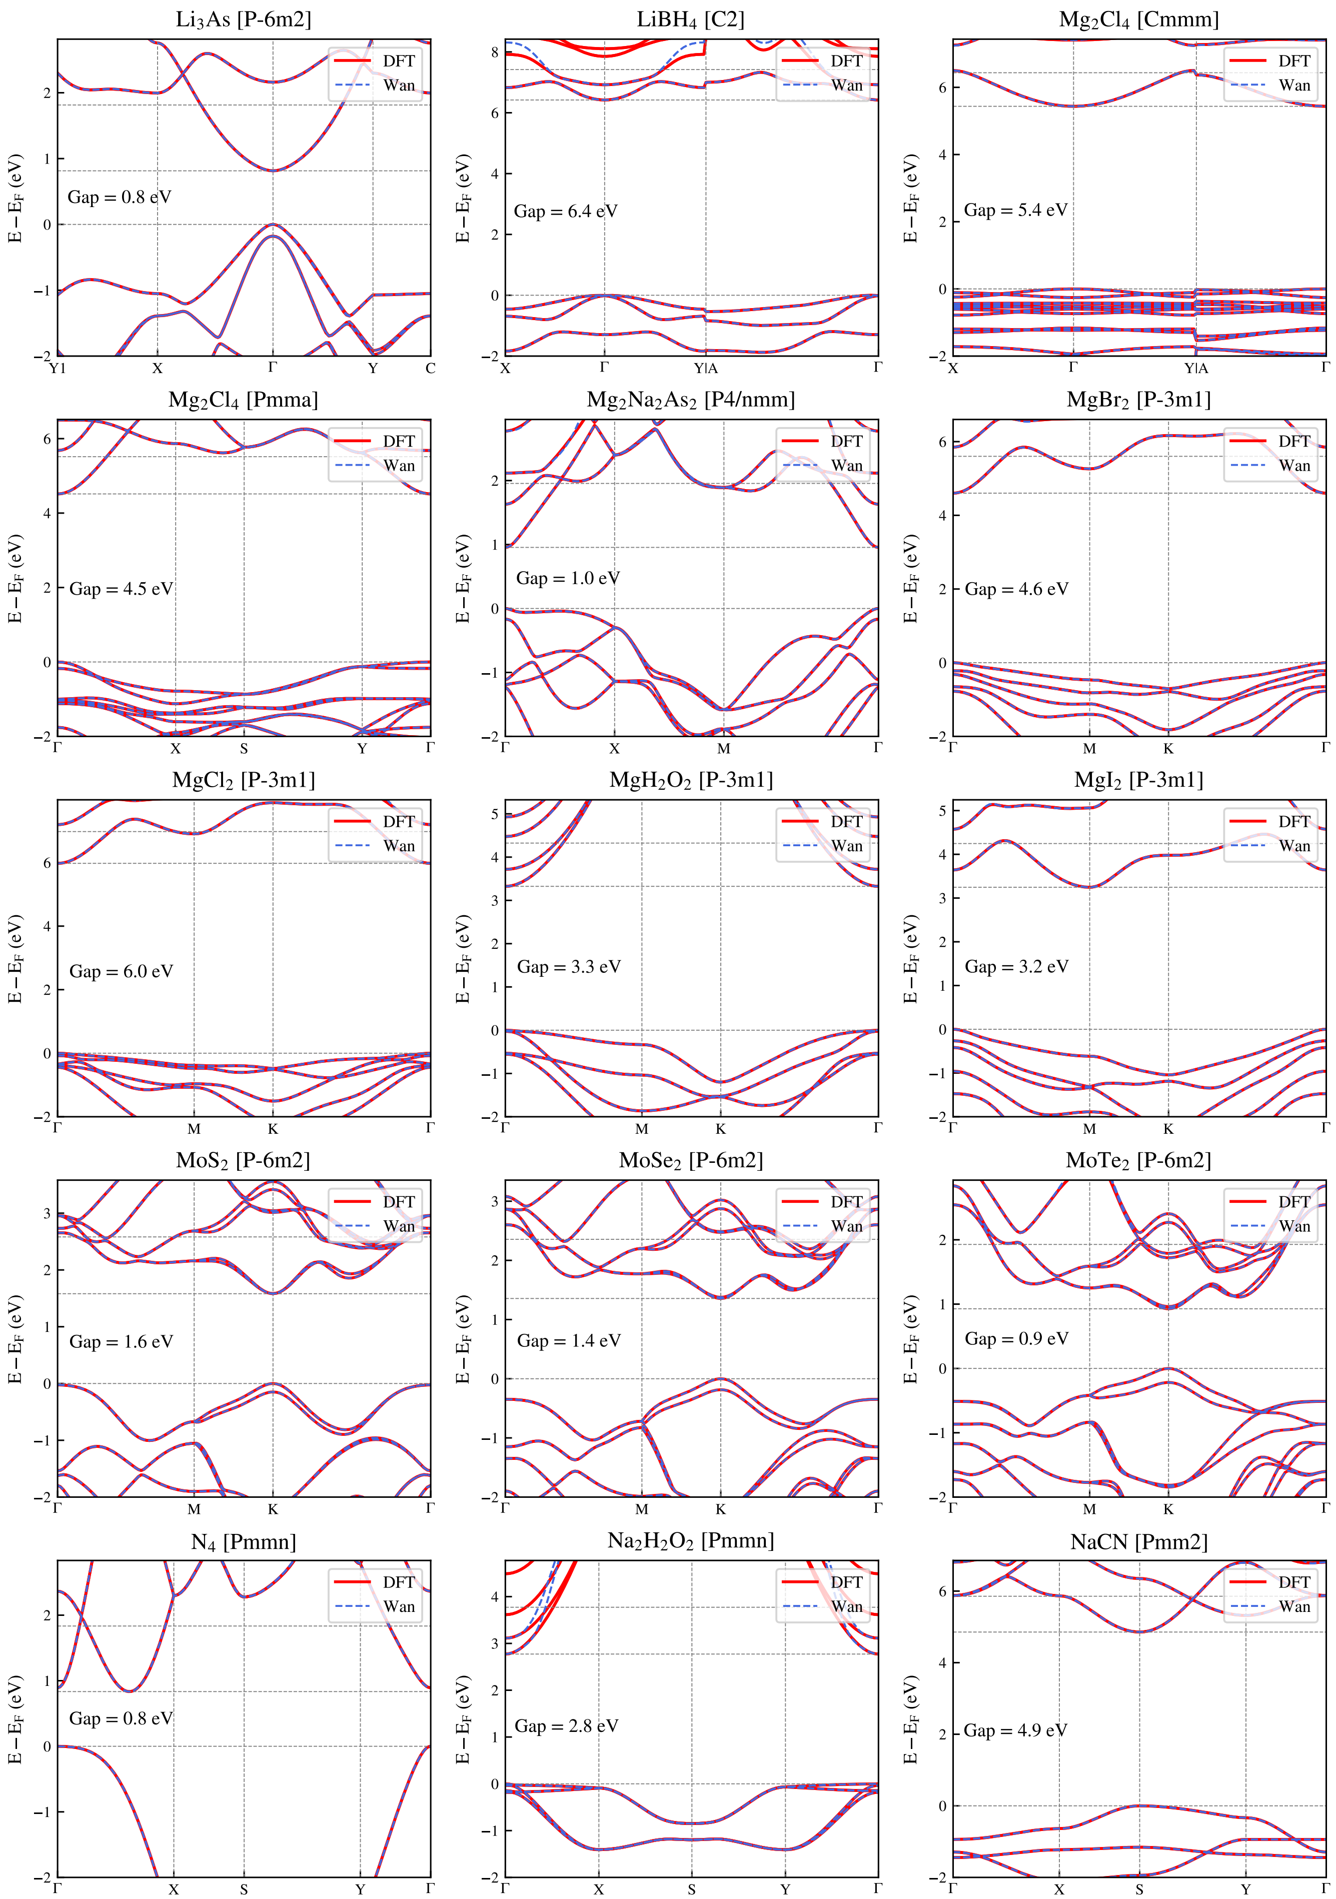

$Li_3As$ [P-6m2]
Gap = 0.8 eV
$LiBH_4$ [C2]
Gap = 6.4 eV
$Mg_2Cl_4$ [Cmmm]
Gap = 5.4 eV
$Mg_2Cl_4$ [Pmma]
Gap = 4.5 eV
$Mg_2Na_2As_2$ [P4/nmm]
Gap = 1.0 eV
$MgBr_2$ [P-3m1]
Gap = 4.6 eV
$MgCl_2$ [P-3m1]
Gap = 6.0 eV
$MgH_2O_2$ [P-3m1]
Gap = 3.3 eV
$MgI_2$ [P-3m1]
Gap = 3.2 eV
$MoS_2$ [P-6m2]
Gap = 1.6 eV
$MoSe_2$ [P-6m2]
Gap = 1.4 eV
$MoTe_2$ [P-6m2]
Gap = 0.9 eV
$N_4$ [Pmmn]
Gap = 0.8 eV
$Na_2H_2O_2$ [Pmmn]
Gap = 2.8 eV
NaCN [Pmm2]
Gap = 4.9 eV
DFT
Wan
$E - E_F$ (eV)

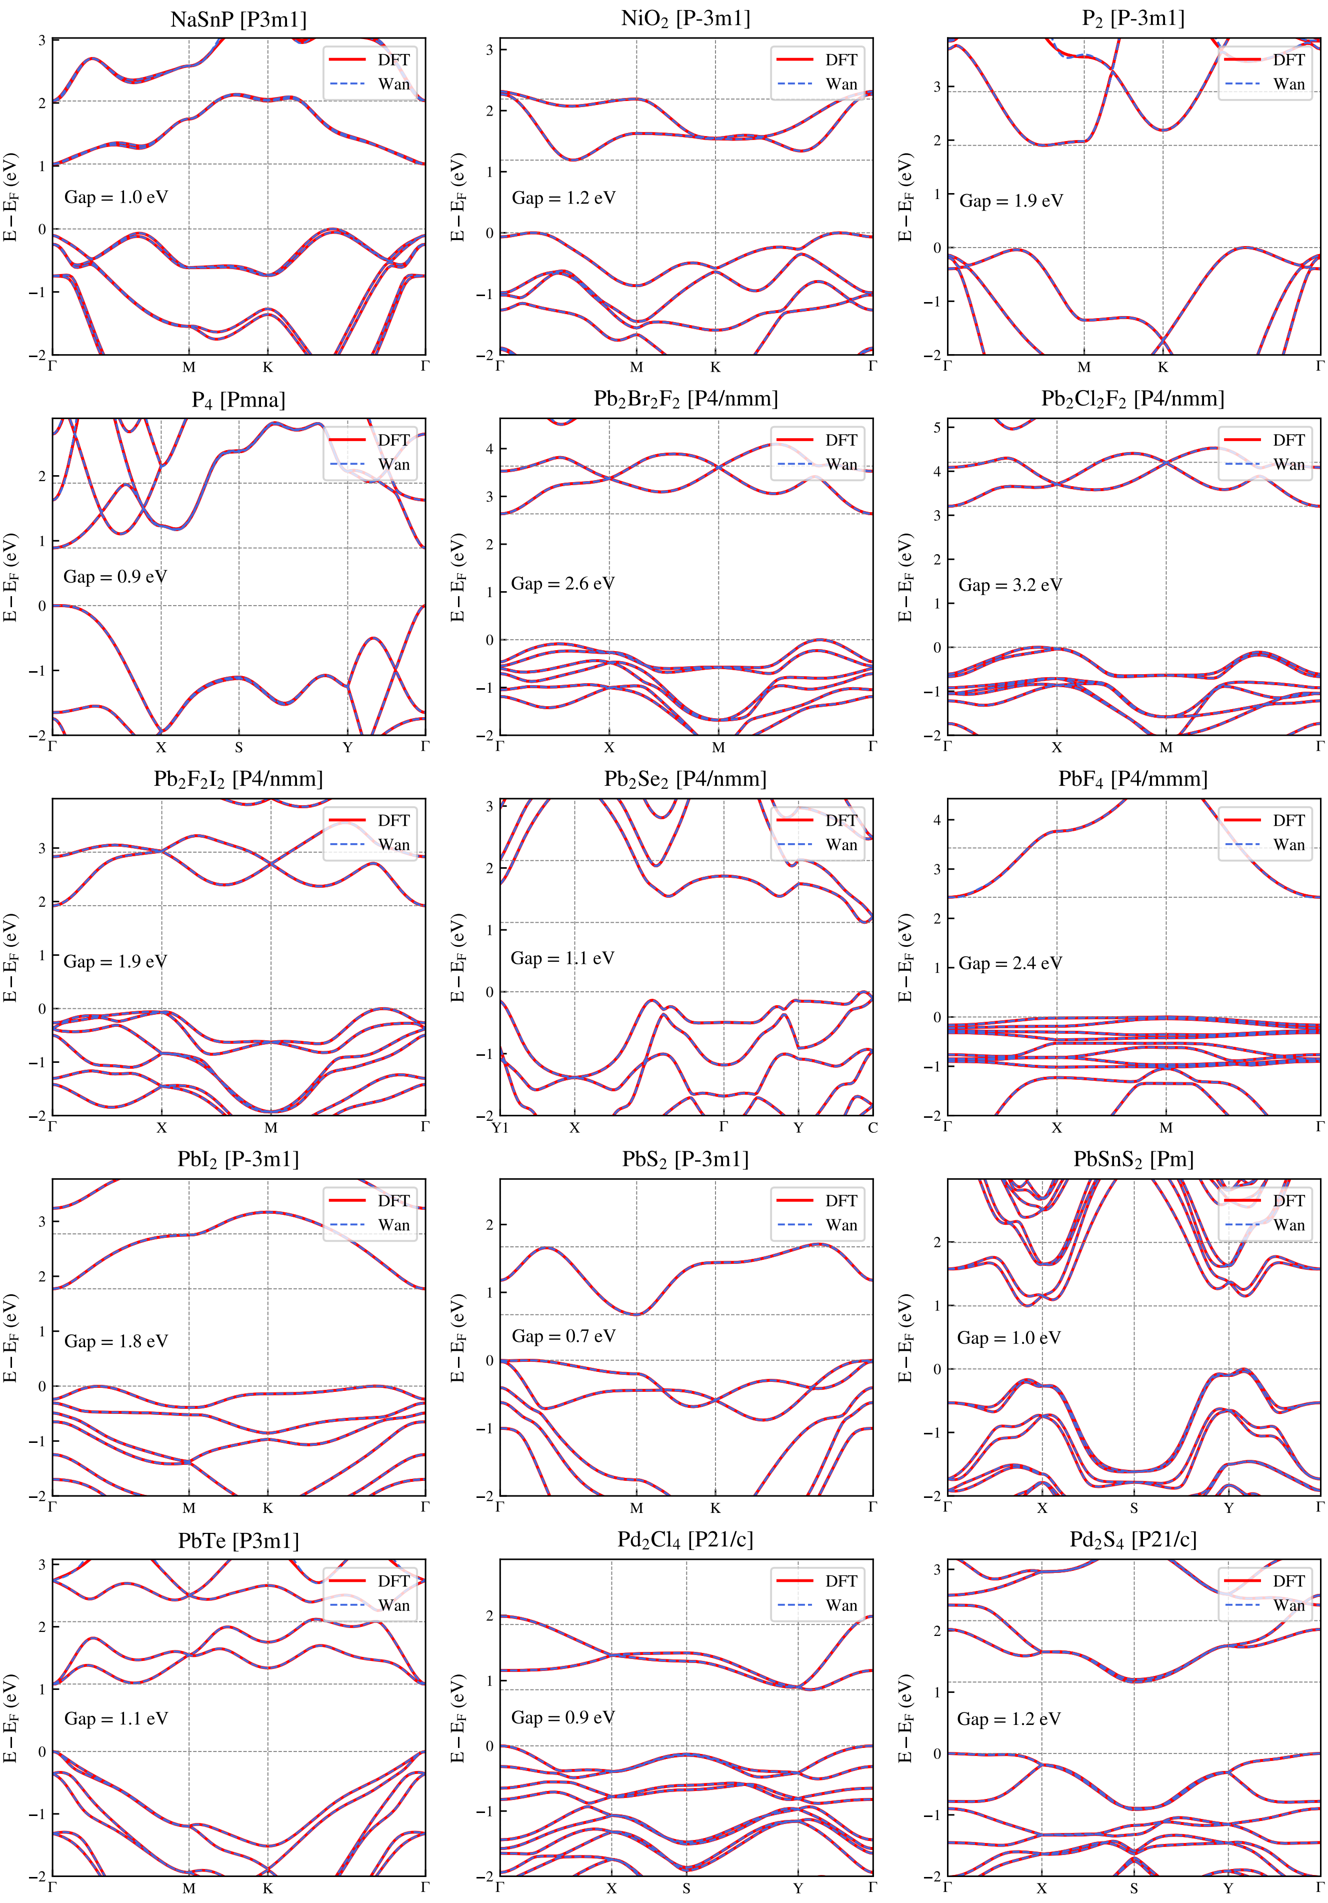
NaSnP [P3m1]
Gap = 1.0 eV
NiO2 [P-3m1]
Gap = 1.2 eV
P2 [P-3m1]
Gap = 1.9 eV
P4 [Pmna]
Gap = 0.9 eV
Pb2Br2F2 [P4/nmm]
Gap = 2.6 eV
Pb2Cl2F2 [P4/nmm]
Gap = 3.2 eV
Pb2F2I2 [P4/nmm]
Gap = 1.9 eV
Pb2Se2 [P4/nmm]
Gap = 1.1 eV
PbF4 [P4/mmm]
Gap = 2.4 eV
PbI2 [P-3m1]
Gap = 1.8 eV
PbS2 [P-3m1]
Gap = 0.7 eV
PbSnS2 [Pm]
Gap = 1.0 eV
PbTe [P3m1]
Gap = 1.1 eV
Pd2Cl4 [P21/c]
Gap = 0.9 eV
Pd2S4 [P21/c]
Gap = 1.2 eV
DFT
Wan
E − EF (eV)
Γ
M
K
X
S
Y
Y1
C

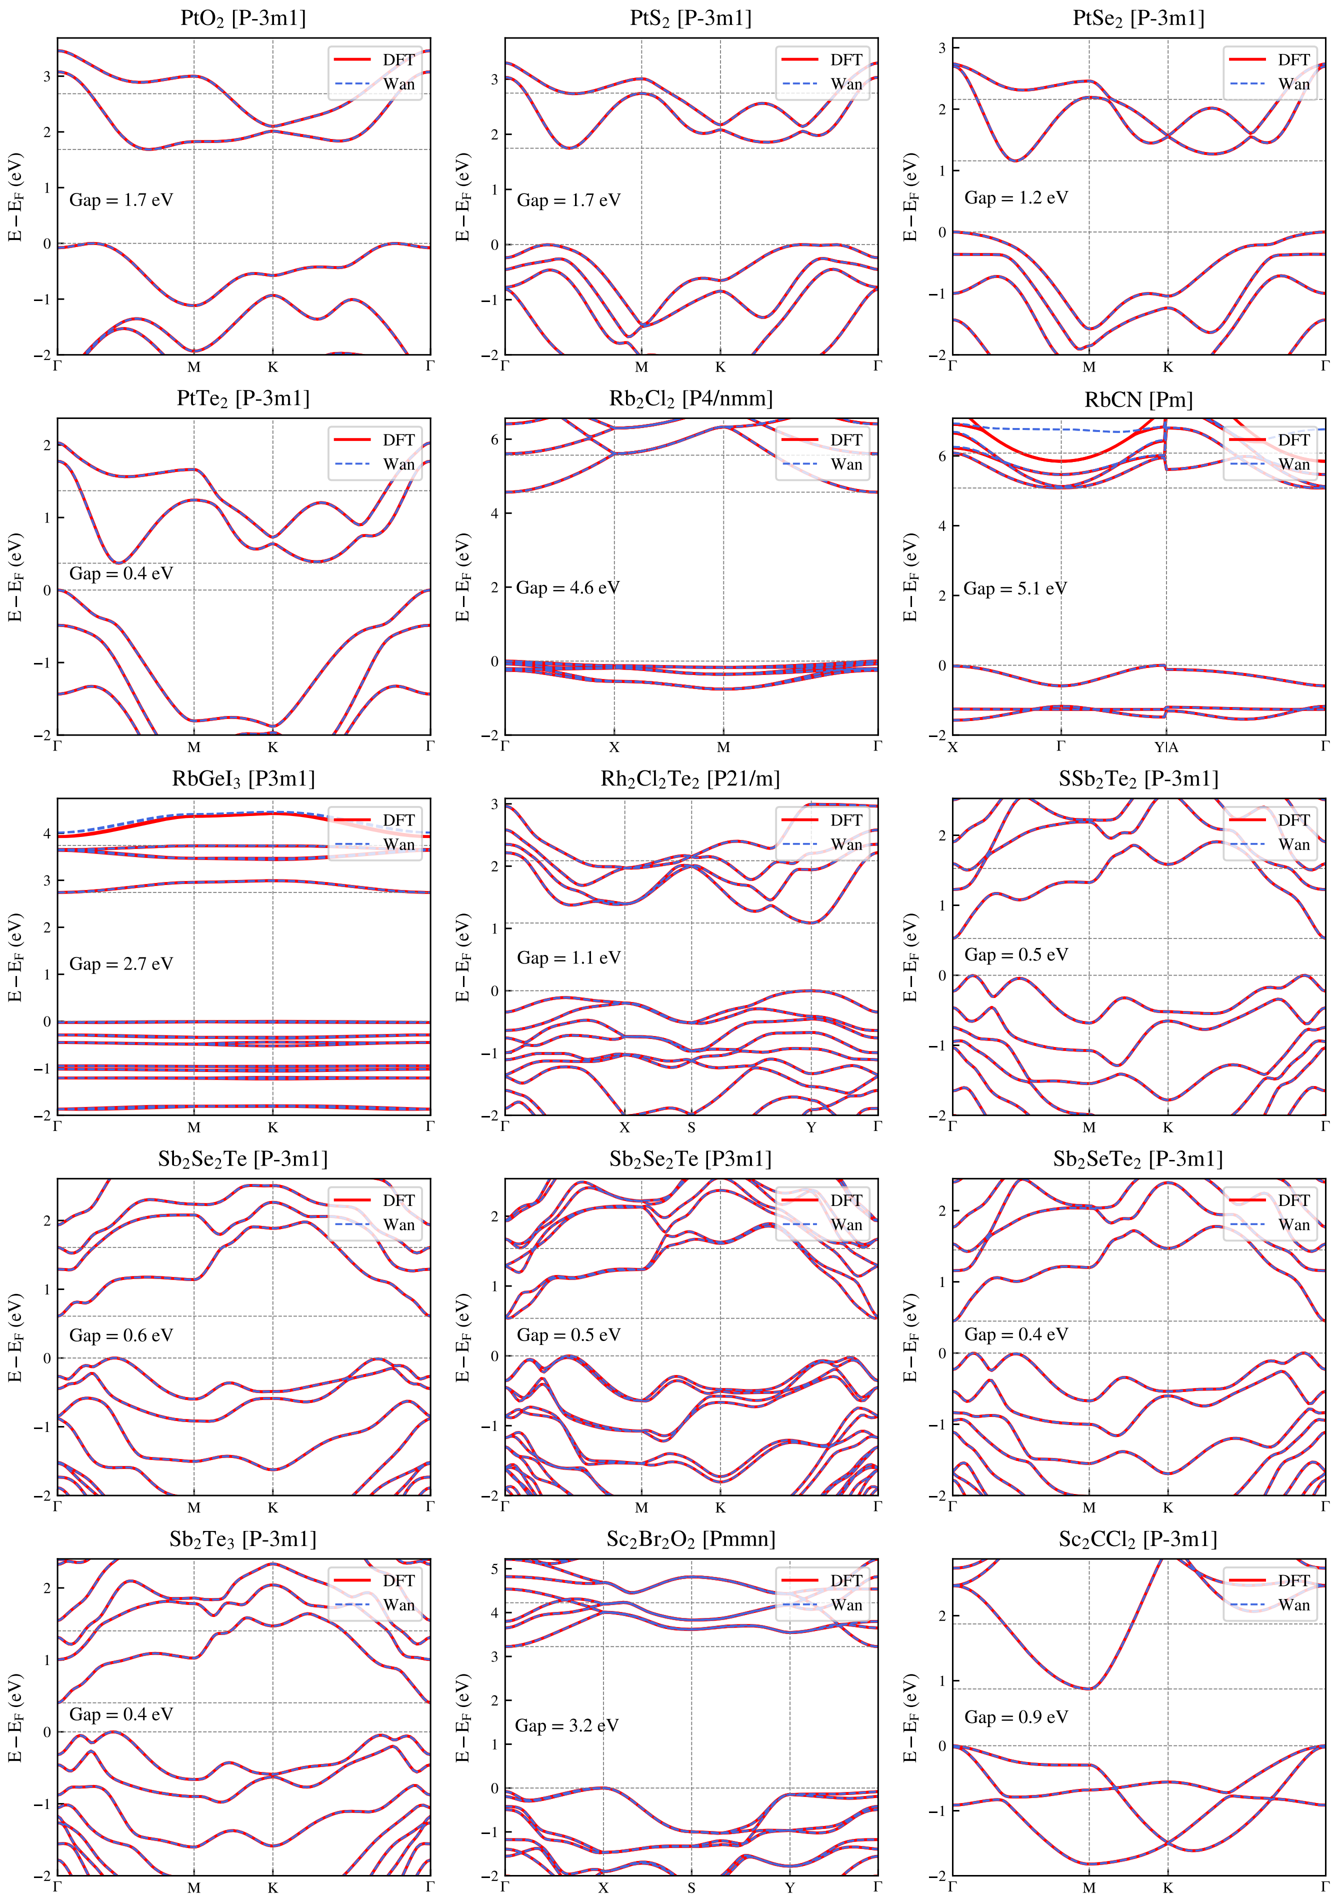
PtO2 [P-3m1]
Gap = 1.7 eV
PtS2 [P-3m1]
Gap = 1.7 eV
PtSe2 [P-3m1]
Gap = 1.2 eV
PtTe2 [P-3m1]
Gap = 0.4 eV
Rb2Cl2 [P4/nmm]
Gap = 4.6 eV
RbCN [Pm]
Gap = 5.1 eV
RbGeI3 [P3m1]
Gap = 2.7 eV
Rh2Cl2Te2 [P21/m]
Gap = 1.1 eV
SSb2Te2 [P-3m1]
Gap = 0.5 eV
Sb2Se2Te [P-3m1]
Gap = 0.6 eV
Sb2Se2Te [P3m1]
Gap = 0.5 eV
Sb2SeTe2 [P-3m1]
Gap = 0.4 eV
Sb2Te3 [P-3m1]
Gap = 0.4 eV
Sc2Br2O2 [Pmmn]
Gap = 3.2 eV
Sc2CCl2 [P-3m1]
Gap = 0.9 eV
DFT
Wan
E − E_F (eV)
Γ M K Γ
Γ X M Γ
X Γ Y|A Γ
Γ X S Y Γ

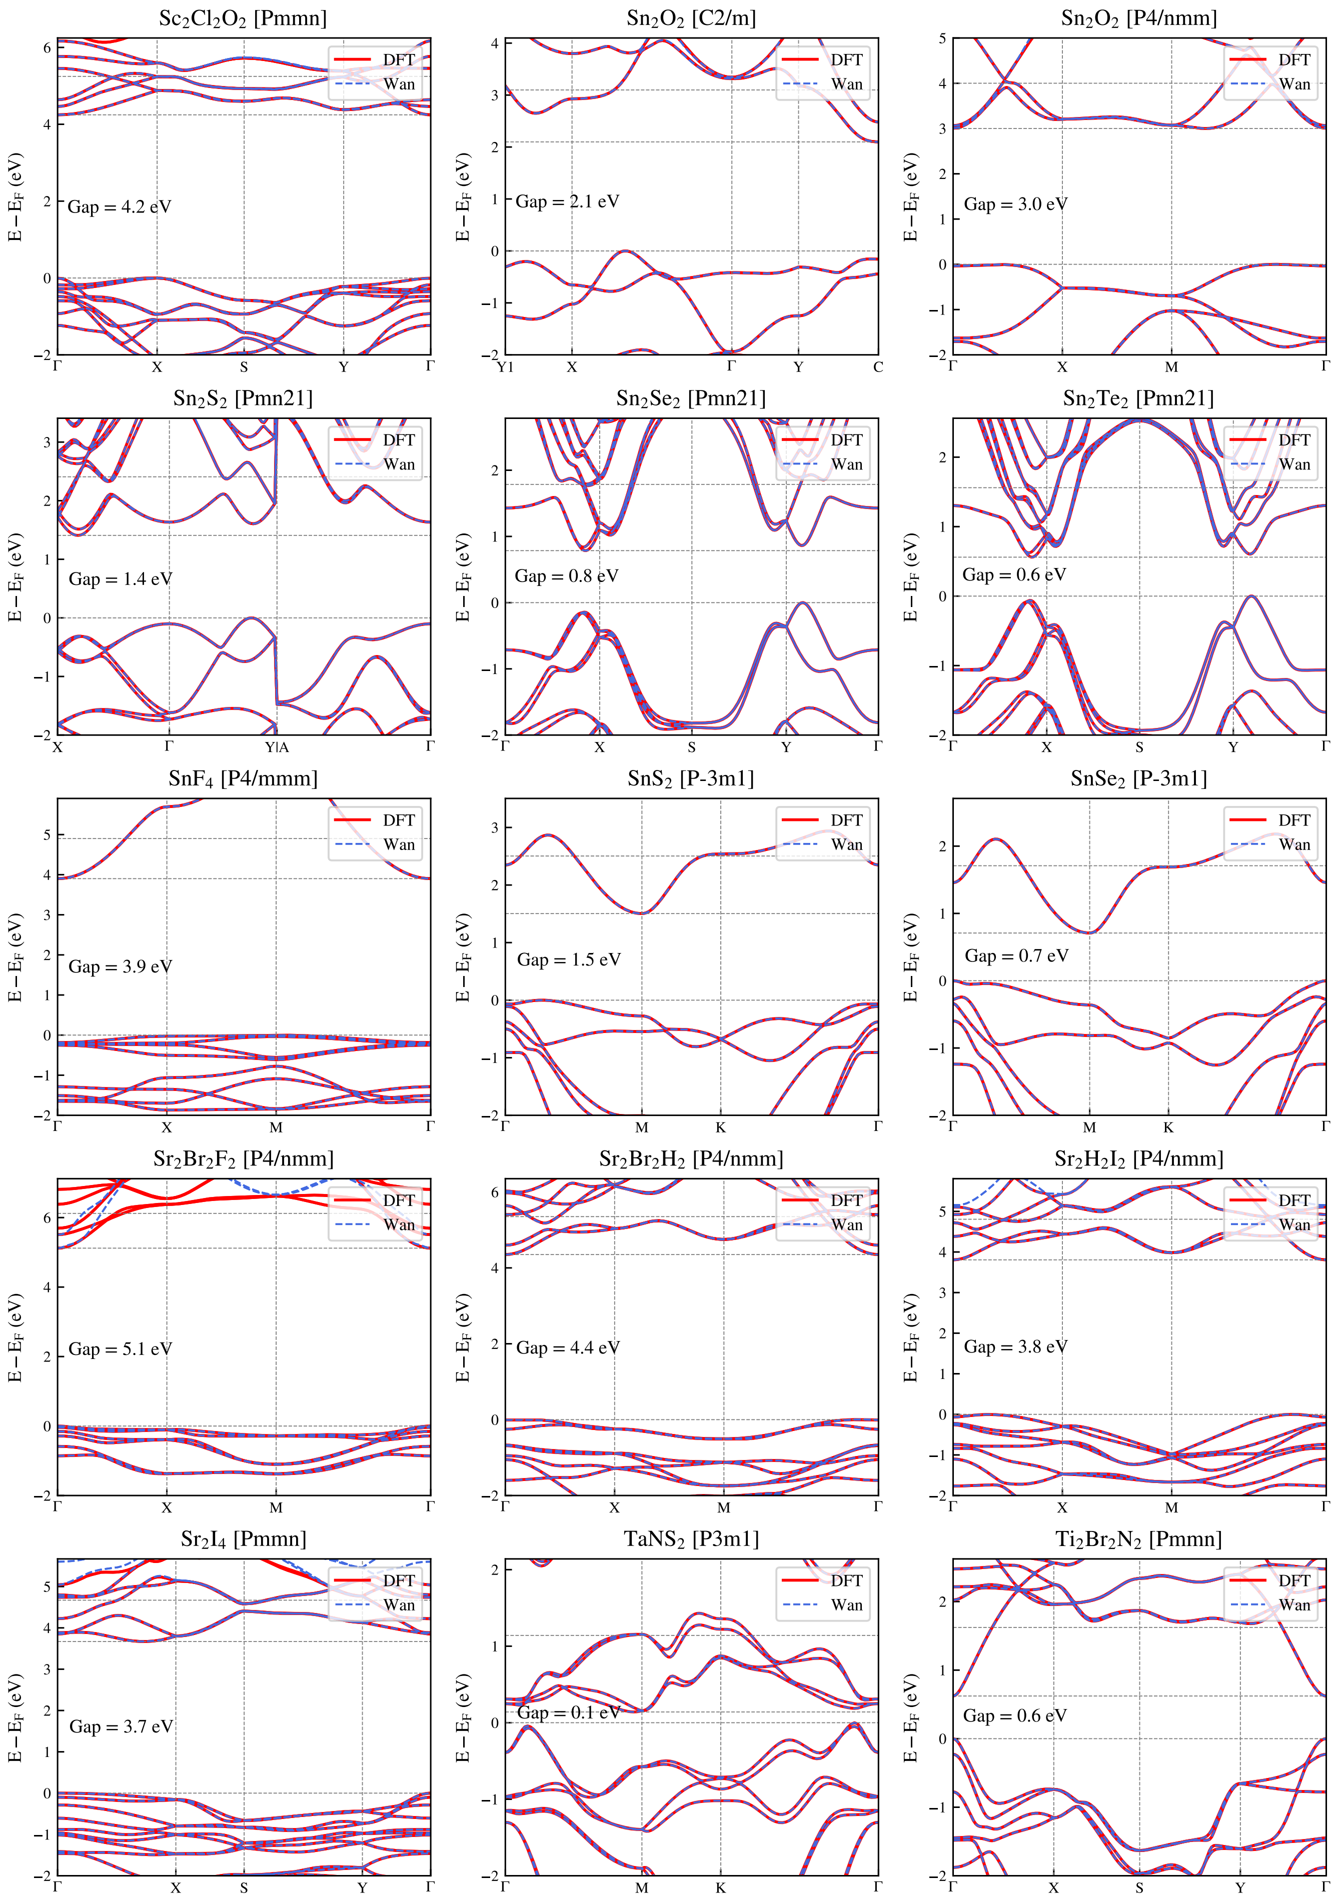

Sc2Cl2O2 [Pmmn]
Gap = 4.2 eV
Γ X S Y Γ
Sn2O2 [C2/m]
Gap = 2.1 eV
Y1 X Γ Y C
Sn2O2 [P4/nmm]
Gap = 3.0 eV
Γ X M Γ
Sn2S2 [Pmn21]
Gap = 1.4 eV
X Γ Y|A Γ
Sn2Se2 [Pmn21]
Gap = 0.8 eV
Γ X S Y Γ
Sn2Te2 [Pmn21]
Gap = 0.6 eV
Γ X S Y Γ
SnF4 [P4/mmm]
Gap = 3.9 eV
Γ X M Γ
SnS2 [P-3m1]
Gap = 1.5 eV
Γ M K Γ
SnSe2 [P-3m1]
Gap = 0.7 eV
Γ M K Γ
Sr2Br2F2 [P4/nmm]
Gap = 5.1 eV
Γ X M Γ
Sr2Br2H2 [P4/nmm]
Gap = 4.4 eV
Γ X M Γ
Sr2H2I2 [P4/nmm]
Gap = 3.8 eV
Γ X M Γ
Sr2I4 [Pmmn]
Gap = 3.7 eV
Γ X S Y Γ
TaNS2 [P3m1]
Gap = 0.1 eV
Γ M K Γ
Ti2Br2N2 [Pmmn]
Gap = 0.6 eV
Γ X S Y Γ
DFT
Wan
E − EF (eV)

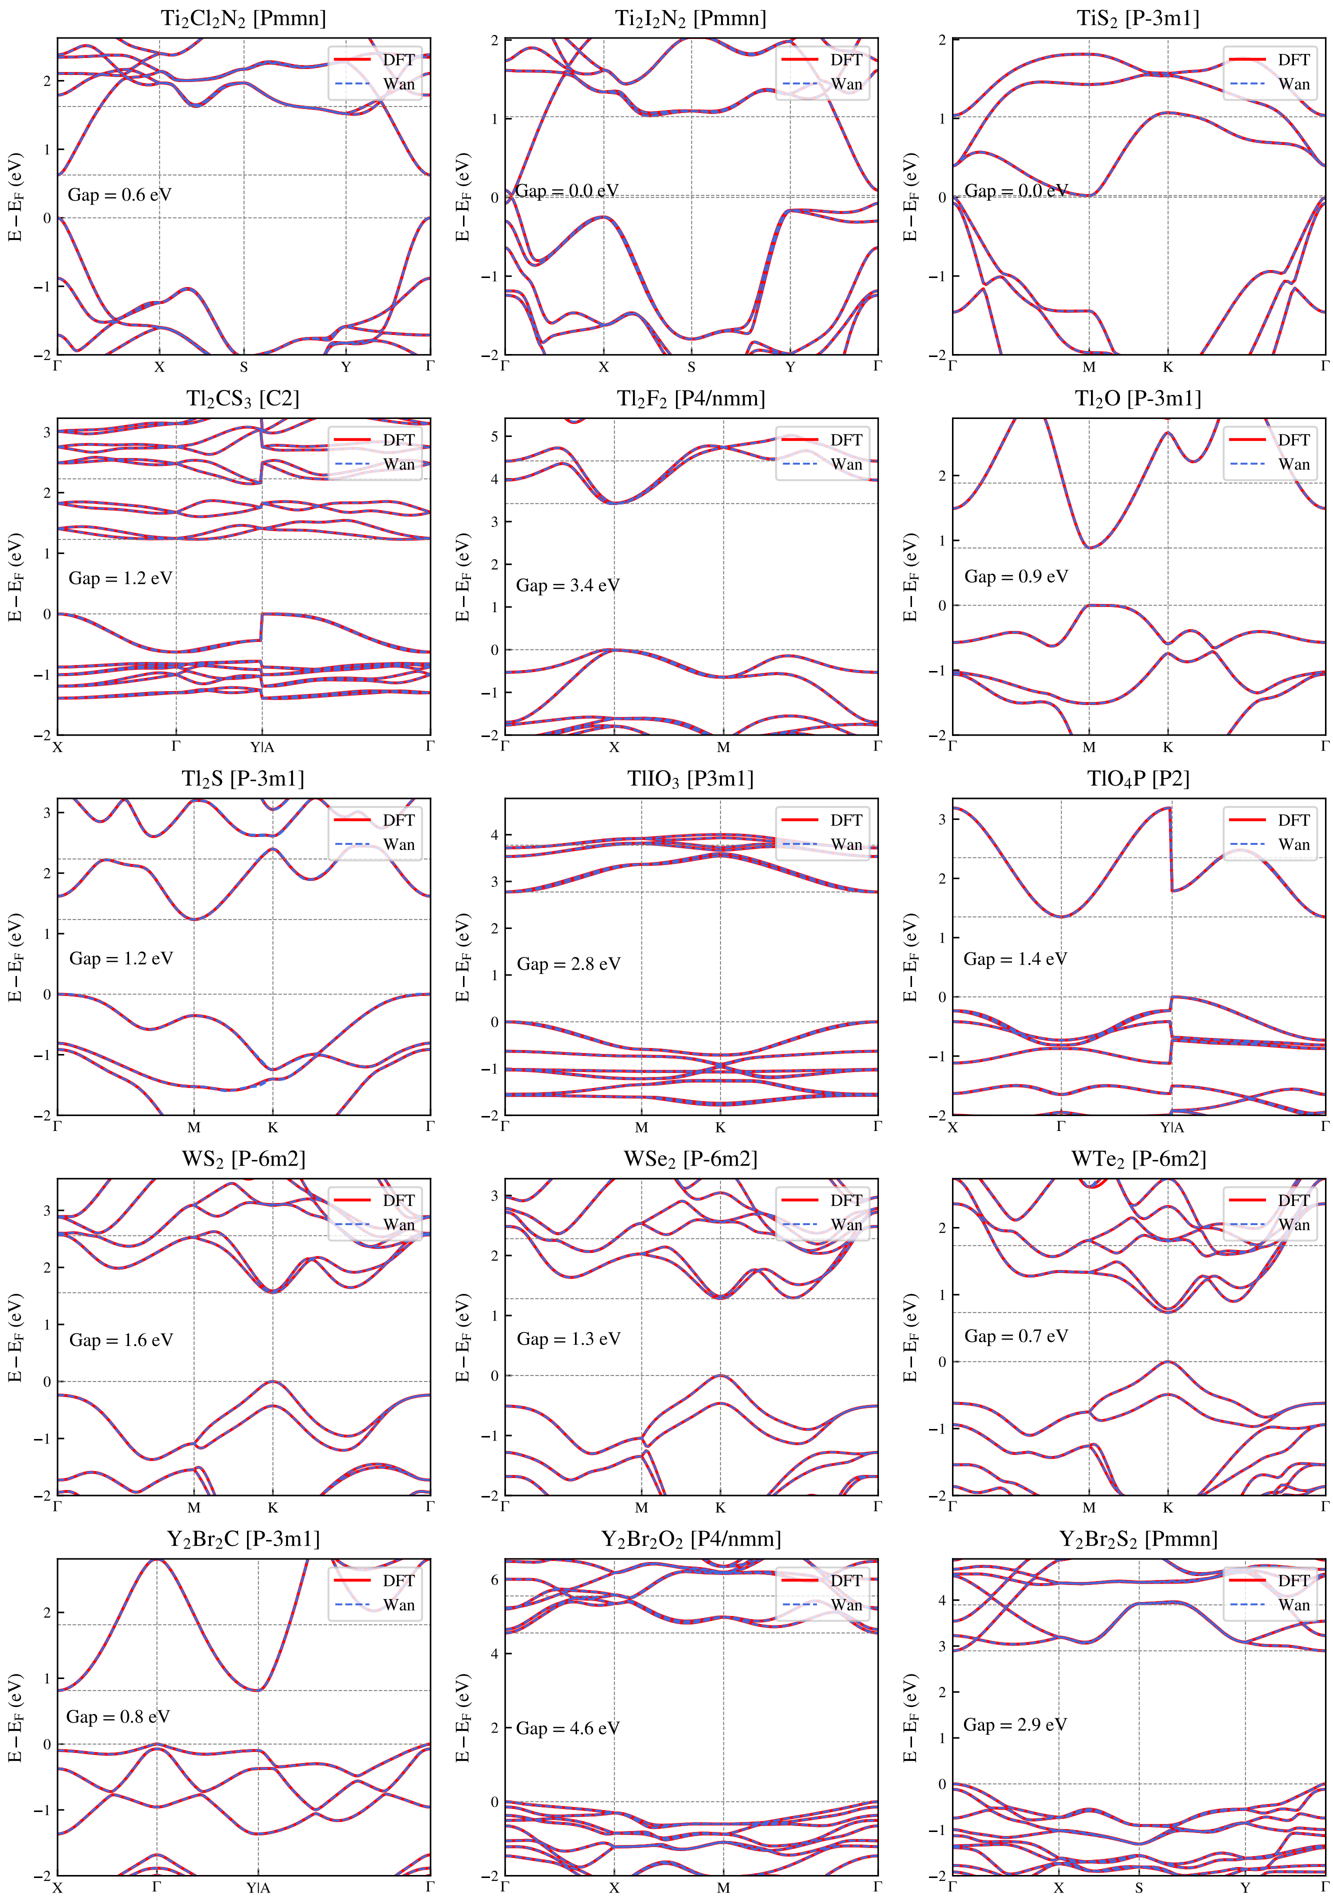
Ti2Cl2N2 [Pmmn]
Gap = 0.6 eV
Ti2I2N2 [Pmmn]
Gap = 0.0 eV
TiS2 [P-3m1]
Gap = 0.0 eV
Tl2CS3 [C2]
Gap = 1.2 eV
Tl2F2 [P4/nmm]
Gap = 3.4 eV
Tl2O [P-3m1]
Gap = 0.9 eV
Tl2S [P-3m1]
Gap = 1.2 eV
TlIO3 [P3m1]
Gap = 2.8 eV
TlO4P [P2]
Gap = 1.4 eV
WS2 [P-6m2]
Gap = 1.6 eV
WSe2 [P-6m2]
Gap = 1.3 eV
WTe2 [P-6m2]
Gap = 0.7 eV
Y2Br2C [P-3m1]
Gap = 0.8 eV
Y2Br2O2 [P4/nmm]
Gap = 4.6 eV
Y2Br2S2 [Pmmn]
Gap = 2.9 eV
DFT
Wan
E − EF (eV)

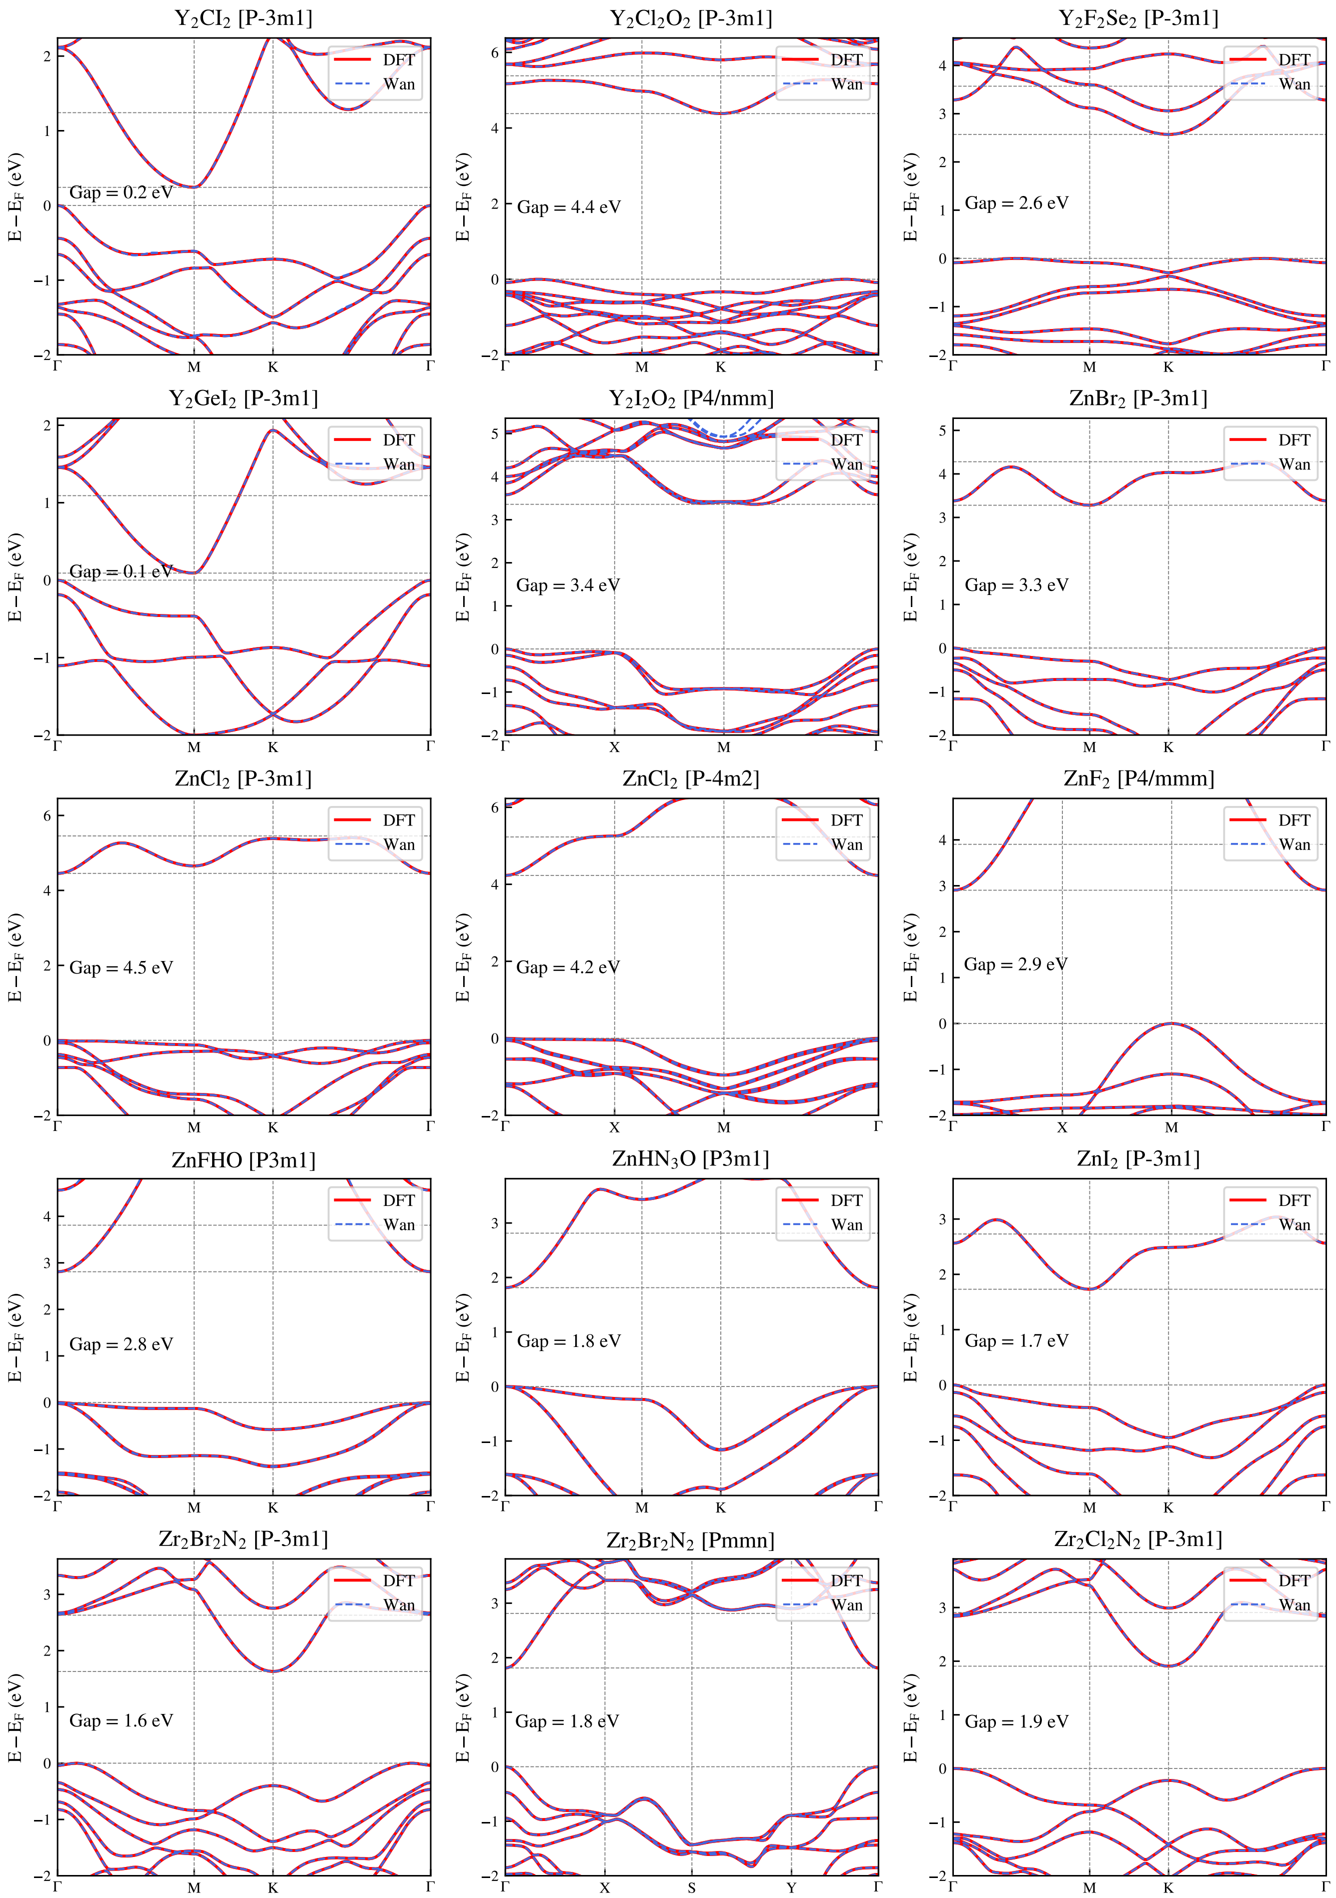

$Y_2CI_2$ [P-3m1]
Gap = 0.2 eV
$Y_2Cl_2O_2$ [P-3m1]
Gap = 4.4 eV
$Y_2F_2Se_2$ [P-3m1]
Gap = 2.6 eV
$Y_2GeI_2$ [P-3m1]
Gap = 0.1 eV
$Y_2I_2O_2$ [P4/nmm]
Gap = 3.4 eV
$ZnBr_2$ [P-3m1]
Gap = 3.3 eV
$ZnCl_2$ [P-3m1]
Gap = 4.5 eV
$ZnCl_2$ [P-4m2]
Gap = 4.2 eV
$ZnF_2$ [P4/mmm]
Gap = 2.9 eV
ZnFHO [P3m1]
Gap = 2.8 eV
$ZnHN_3O$ [P3m1]
Gap = 1.8 eV
$ZnI_2$ [P-3m1]
Gap = 1.7 eV
$Zr_2Br_2N_2$ [P-3m1]
Gap = 1.6 eV
$Zr_2Br_2N_2$ [Pmmn]
Gap = 1.8 eV
$Zr_2Cl_2N_2$ [P-3m1]
Gap = 1.9 eV
DFT
Wan
$E - E_F$ (eV)
Γ
M
K
X
S
Y

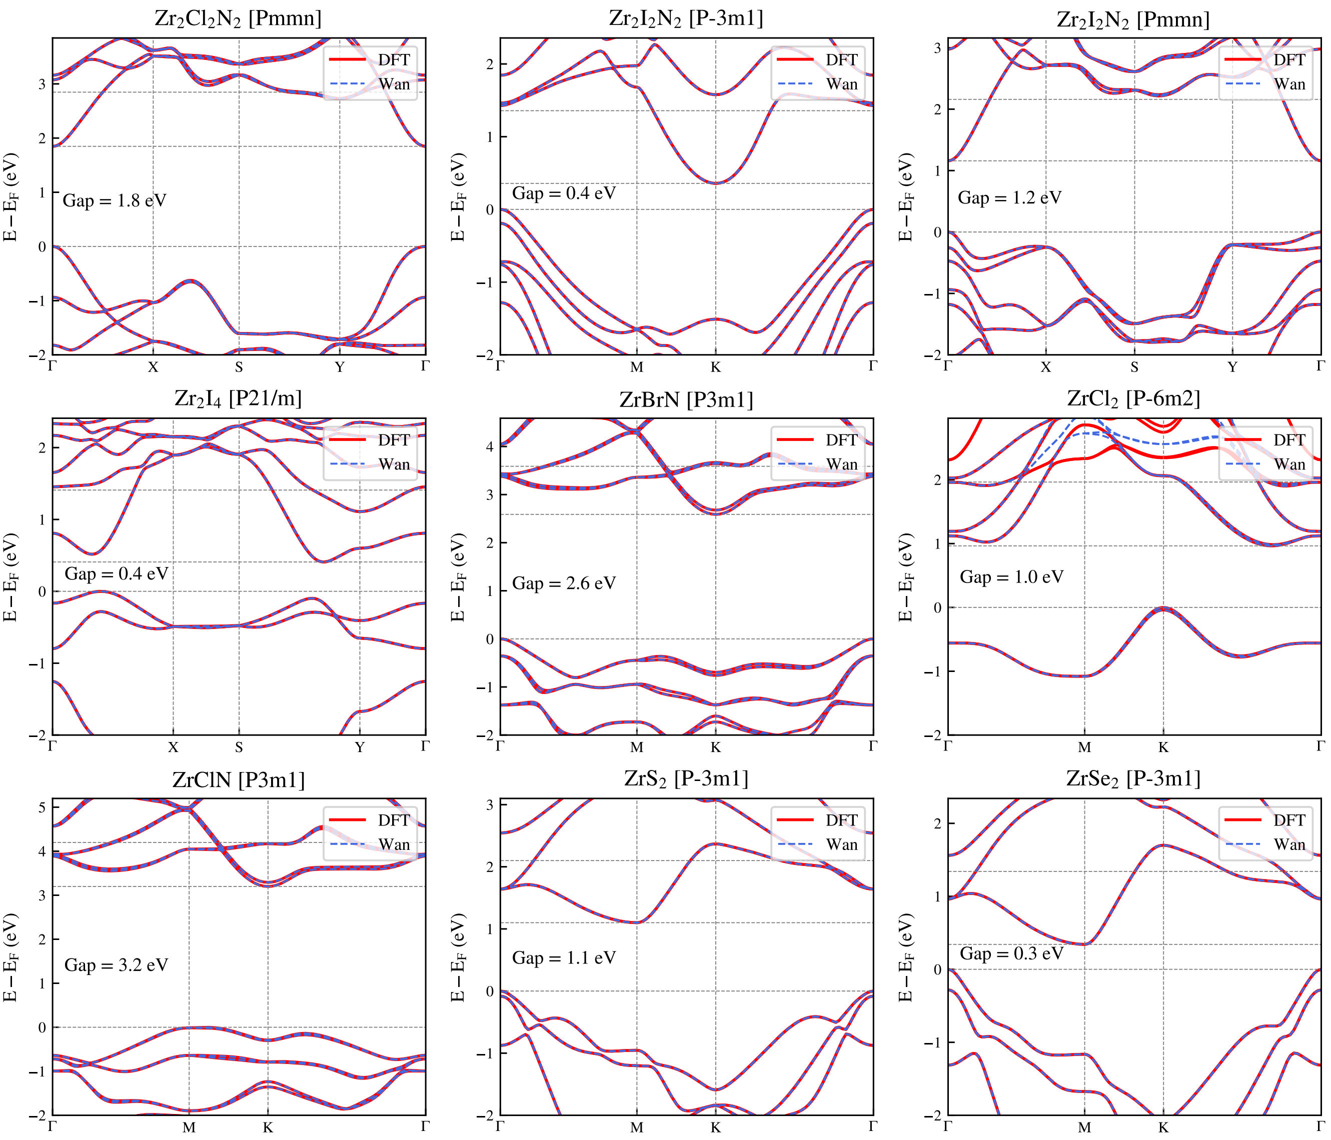
$Zr_2Cl_2N_2$ [Pmmn]
Gap = 1.8 eV
$Zr_2I_2N_2$ [P-3m1]
Gap = 0.4 eV
$Zr_2I_2N_2$ [Pmmn]
Gap = 1.2 eV
$Zr_2I_4$ [P21/m]
Gap = 0.4 eV
ZrBrN [P3m1]
Gap = 2.6 eV
$ZrCl_2$ [P-6m2]
Gap = 1.0 eV
ZrClN [P3m1]
Gap = 3.2 eV
$ZrS_2$ [P-3m1]
Gap = 1.1 eV
$ZrSe_2$ [P-3m1]
Gap = 0.3 eV
DFT
Wan
$E - E_F$ (eV)
Γ
X
S
Y
M
K

## REFERENCES


[1] Gutierrez-Amigo, M. *et al.* Purely anharmonic charge density wave in the two-dimensional Dirac semimetal SnP. *Phys. Rev. B* **109**, 174112 (2024).

[2] Jiang, Z., Wang, P., Xing, J., Jiang, X. & Zhao, J. Screening and Design of Novel 2D Ferromagnetic Materials with High Curie Temperature above Room Temperature. *ACS Appl. Mater. Interfaces* **10**, 39032–39039 (2018).

[3] Timrov, I., Marzari, N. & Cococcioni, M. HP – A code for the calculation of Hubbard parameters using density-functional perturbation theory. *Comput. Phys. Commun.* **279**, 108455 (2022).

[4] Gong, C. & Zhang, X. Two-dimensional magnetic crystals and emergent heterostructure devices. *Science* **363**, eaav4450 (2019).

[5] Lado, J. L. & Fernández-Rossier, J. On the origin of magnetic anisotropy in two dimensional $CrI_3$. *2D Mater.* **4**, 035002 (2017).

[6] Li, J. *et al.* Intrinsic magnetic topological insulators in van der waals layered $MnBi_2Te_4$-family materials. *Science Advances* **5**, eaaw5685 (2019).

[7] Otrokov, M. M. *et al.* Unique Thickness-Dependent Properties of the van der Waals Interlayer Antiferromagnet $MnBi_2Te_4$ Films. *Phys. Rev. Lett.* **122**, 107202 (2019).
